# Supplementary material for: Nonlinear Random Matrices and Applications to the Sum of Squares Hierarchy
Source: arXiv:2302.04462 source file (2023-02-09)
Supplement: Supplementary file 1 [file appendix.tex]

%\begin{appendix}
\section{Omitted technical details}
	\subsection{Proof that the Leftmost and Rightmost Minimum Vertex Separators are Well-defined}\label{separatorswelldefinedsection}
	In this section, we give a general proof that the leftmost and rightmost minimum vertex separators are well-defined.
	\begin{lemma}\label{leftrightseparatorlemma}
		For any two distinct vertex separators $S_1$ and $S_2$ of $\alpha$, there exist vertex separators $S_L$ and $S_R$ of $\alpha$ such that:
		\begin{enumerate}
			\item $S_L$ is a vertex separator of $U_{\alpha}$ and $S_1$ and a vertex separator of $U_{\alpha}$ and $S_2$.
			\item $S_R$ is a vertex separator of $S_1$ and $V_{\alpha}$ and a vertex separator of $S_2$ and $V_{\alpha}$.
			\item $w(S_L) + w(S_R) \leq w(S_1) + w(S_2)$
		\end{enumerate}
	\end{lemma}
	\begin{proof}
		Take $S_L$ to be the set of vertices $v \in V(\alpha) \cap (S_1 \cup S_2)$ such that there is a path from $U_{\alpha}$ to $v$ which doesn't intersect $S_1 \cup S_2$ before reaching $v$. Similarly, take $S_R$ to be the set of vertices $v \in V(\alpha) \cap (S_1 \cup S_2)$ such that there is a path from $V_{\alpha}$ to $v$ which doesn't intersect $S_1 \cup S_2$ before reaching $v$.
		
		Now observe that $S_L$ is a vertex separator between $U_{\alpha}$ and $S_1$. To see this, note that for any path $P$ from $U_{\alpha}$ to a vertex $v \in S_1$, either $P$ intersects $S_L$ before reaching $v$ or $P$ does not intersect $S_L$ before reaching $v$. In the latter case, $v \in S_L$. Thus, in either case, $P$ intersects $S_L$. Following similar logic, $S_L$ is also a vertex separator between $U_{\alpha}$ and $S_2$, $S_R$ is a vertex separator between $S_1$ and $V_{\alpha}$, and $S_R$ is also a vertex separator between $S_2$ and $V_{\alpha}$.
		
		To show that $w(S_L) + w(S_R) \leq w(S_1) + w(S_2)$, observe that $w(S_L) + w(S_R) = w(S_R \cup S_R) + w(S_L \cap S_R)$ and $w(S_1) + w(S_2) = w(S_1 \cup S_2) + w(S_1 \cap S_2)$. Thus, to show that $w(S_L) + w(S_R) \leq w(S_1) + w(S_2)$, it is sufficient to show that
		\begin{enumerate}
			\item $S_L \cup S_R \subseteq S_1 \cup S_2$
			\item $S_L \cap S_R \subseteq S_1 \cap S_2$
		\end{enumerate}
		For the first statement, note that by definition any vertex in $S_L \cup S_R$ must be in $S_1 \cup S_2$. For the second statement, note that if $v \in S_L \cap S_R$ then there is a path from $U_{\alpha}$ to $v$ which does not intersect any other vertices in $S_1 \cup S_2$ and there is a path from $v$ to $V_{\alpha}$ which does not intersect any other vertices in $S_1 \cup S_2$. Combining these paths, we obtain a path $P$ from $U_{\alpha}$ to $V_{\alpha}$ such that $v$ is the only vertex in $P$ which is in $S_1 \cup S_2$. This implies that $v \in S_1 \cap S_2$ as otherwise either $S_1$ or $S_2$ would not be a vertex separator between $U_{\alpha}$ and $V_{\alpha}$.
	\end{proof}
	\begin{corollary}
		The leftmost and rightmost minimum vertex separators between $U_{\alpha}$ and $V_{\alpha}$ are well-defined.
	\end{corollary}
	\begin{proof}
		Assume that there is no minimum leftmost vertex separator. If so, then there exists a minimum vertex separator $S_1$ between $U_{\alpha}$ and $V_{\alpha}$ such that 
		\begin{enumerate}
			\item There does not exist a minimum vertex separator $S'$ of $\alpha$ such that $S'$ is also a minimum vertex separator of $U_{\alpha}$ and $S_1$ (otherwise we would take $S'$ rather than $S$)
			\item There exists a minimum vertex separator $S_2$ of $\alpha$ such that $S'$ is not a minimum vertex separator of $U_{\alpha}$ and $S_2$ (as otherwise $S_1$ would be the leftmost minimum vertex separator)
		\end{enumerate}
		Now let $S_L$ and $S_R$ be the vertex separators of $\alpha$ obtained by applying Lemma \ref{leftrightseparatorlemma} to $S_1$ and $S_2$. Since $S_1$ and $S_2$ are minimum vertex separators of $\alpha$, we must have that $w(S_L) = w(S_R) = w(S_1) = w(S_2)$. Since $S_L$ is a vertex separator of $U_{\alpha}$ and $S_2$, $S_L \neq S_1$. However, $S_L$ is a vertex separator of $U_{\alpha}$ and $S_1$, which contradicts our choice of $S_1$.
		
		Thus, there must be a leftmost minimum vertex separator of $\alpha$. Following similar logic, there must be a rightmost minimum vertex separator of $\alpha$ as well.
	\end{proof}
	\subsection{Proofs with Canonical Maps}\label{canonicalmapsection}
	In this section, we give alternative proofs of Lemmas \ref{lm:morthsimplereexpression} and \ref{lm:singleshapeintersections} using canonical maps.
	\begin{definition}[Canonical Maps]
		For each shape $\alpha$ and each ribbon $R$ of shape $\alpha$, we arbitrarily choose a canonical map $\phi_R: V(\alpha) \to V(R)$ such that $\phi_R(H_{\alpha}) = H_R$, $\phi_{R}(U_{\alpha}) = A_R$, and $\phi_{R}(V_{\alpha}) = B_R$. Note that there are $|Aut(\alpha)|$ possible choices for this map.
	\end{definition}
	\subsection{Proof of Lemma \ref{lm:morthsimplereexpression}}
	\begin{lemma}
		\[
		M^{orth}_{\tau}(H) = \sum_{\sigma \in Row(H),\sigma' \in Col(H)}{H(\sigma,\sigma')|Decomp(\sigma,\tau,{\sigma'}^T)|M_{\sigma \circ \tau \circ {\sigma'}^T}}
		\]
	\end{lemma}
	\begin{proof}
		Observe that there is a bijection between ribbons $R$ with shape $\sigma \circ \tau \circ {\sigma'}^T$ together with an element $\pi \in Decomp(\sigma,\tau,\sigma')$ and triples of ribbons $(R_1,R_2,R_3)$ such that
		\begin{enumerate}
			\item $R_1,R_2,R_3$ have shapes $\sigma$, $\tau$, and ${\sigma'}^T$, respectively.
			\item $V(R_1) \cap V(R_2) = A_{R_2} = B_{R_1}$,  $V(R_2) \cap V(R_3) = A_{R_3} = B_{R_2}$, and $V(R_1) \cap V(R_3) = A_{R_2} \cap B_{R_2}$
		\end{enumerate}
		To see this, note that given such ribbons $R_1,R_2,R_3$, the ribbon $R = R_1 \circ R_2 \circ R_3$ has shape $\sigma \circ \tau \circ {\sigma'}^T$. Further note that we have two bijective maps from $V(\sigma \circ \tau \circ {\sigma'}^T)$ to $V(R)$. The first map is $\phi_R$. The second map is $\phi_{R_1} \circ \phi_{R_2} \circ \phi_{R_3}$. Using this, we can take $\pi = \phi^{-1}_R(\phi_{R_1} \circ \phi_{R_2} \circ \phi_{R_3})$
		
		Conversely, given a ribbon $R$ of shape $\sigma \circ \tau \circ {\sigma'}^T$ and an element $\pi \in Decomp(\sigma,\tau,\sigma')$, let $R_1 = \phi_R(\pi(\sigma))$, let $R_2 = \phi_R(\pi(\tau))$, and let $R_3 = \phi_R(\pi({\sigma'}^T))$. Note that this is well defined because for any element $\pi' \in Aut(\sigma) \times Aut(\tau) \times Aut({\sigma'}^T)$, $\phi_R(\pi\pi'(\sigma)) = \phi_R(\pi(\pi'(\sigma))) = \phi_R(\pi(\sigma))$. Similarly, $\phi_R(\pi\pi'(\tau)) = \phi_R(\pi(\tau))$ and $\phi_R(\pi\pi'({\sigma'}^T)) = \phi_R(\pi({\sigma'}^T))$.
		
		To confirm that this is bijection, we have to show that these two maps are inverses of each other. Given $R_1$, $R_2$, and $R_3$, applying these two maps gives us ribbons $R'_1 = \phi_R\phi^{-1}_R(\phi_{R_1} \circ \phi_{R_2} \circ \phi_{R_3})(H_{\sigma}) = R_1$, $R'_2 = \phi_R\phi^{-1}_R(\phi_{R_1} \circ \phi_{R_2} \circ \phi_{R_3})(H_{\tau}) = R_2$, and $R'_3 = \phi_R\phi^{-1}_R(\phi_{R_1} \circ \phi_{R_2} \circ \phi_{R_3})(H_{{\sigma'}^T}) = R_3$. Conversely, given $R$ and an element $\pi \in Decomp(\sigma,\tau,\sigma')$ (which we represent by an element $\pi \in Aut(\sigma \circ \tau \circ {\sigma'}^T)$), applying these two maps gives us the ribbon 
		\[
		R' = \phi_R(\pi(\sigma)) \circ \phi_R(\pi(\tau)) \circ \phi_R(\pi({\sigma'}^T)) = {\phi_R}\pi(\sigma \circ \tau \circ {\sigma'}^T) = R
		\]
		and gives us the map 
		\[
		\phi^{-1}_R(\phi_{\phi_R(\pi(\sigma))} \circ \phi_{\phi_R(\pi(\tau))} \circ \phi_{\phi_R(\pi({\sigma'}^T))})
		\]
		Now observe that both ${\phi_R}\pi$ and $\phi_{\phi_R(\pi(\sigma))}$ give bijective maps from $\sigma$ to the ribbon ${\phi_R}\pi(\sigma)$ so $\phi^{-1}_{\phi_R(\pi(\sigma))}{\phi_R}\pi \in Aut(\sigma)$. Following similar logic for $\tau$ and ${\sigma'}^T$, in $Decomp(\sigma,\tau,\sigma')$ this map is equivalent to $
		\phi^{-1}_R({\phi_R}\pi) = \pi$
	\end{proof}
	\subsection{Proof of Lemma \ref{lm:singleshapeintersections}}
	\begin{definition}[Rigorous definition of intersection patterns]
		We define an intersection pattern $P$ on composable shapes $\gamma,\tau,{\gamma'}^T$ to consist of the shape $\gamma \circ \tau \circ {\gamma'}^T$ together with a non-empty set of constraint edges $E(P)$ on $V(\gamma \circ \tau \circ {\gamma'}^T)$ such that:
		\begin{enumerate}
			\item For all vertices $u,v,w \in V(\gamma \circ \tau \circ {\gamma'}^T)$, if $(u,v),(v,w) \in E(P)$ then $(u,w) \in E(P)$
			\item $E(P)$ does not contain a path between two vertices of $\gamma$, two vertices of $\tau$, or two vertices of ${\gamma'}^T$. This ensures that when we consider $\gamma,\tau,\gamma'$ individually, their vertices are distinct.
			\item Defining $V_{*}(\gamma) \subseteq V(\gamma)$ to be the vertices of $\gamma$ which are incident to an edge in $E(P)$, $U_{\gamma}$ is the unique minimum-weight vertex separator between $U_{\gamma}$ and $V_{*}(\gamma) \cup V_{\gamma}$
			\item Similarly, defining $V_{*}({\gamma'}^T) \subseteq V({\gamma'}^T)$ to be the vertices of ${\gamma'}^T$ which are incident to an edge in $E(P)$, $V_{{\gamma'}^T}$ is the unique minimum-weight vertex separator between $V_{*}({\gamma'}^T) \cup U_{{\gamma'}^T}$ and $V_{U_{{\gamma'}^T}}$
			\item[5.*] All edges in $E(P)$ are between vertices of the same type.
		\end{enumerate}
	\end{definition}
	\begin{definition}
		We say that two intersection patterns $P,P'$ on shapes $\gamma,\tau,{\gamma'}^T$ are equivalent (which we write as $P \equiv P'$) if there is an automorphism $\pi \in Aut(\gamma) \times Aut(\tau) \times Aut({\gamma'}^T)$ such that $\pi(P) = P'$ (i.e. if $E(P)$ and $E(P')$ are the constraint edges for $P$ and $P'$ respectively then $\pi(E(P)) = E(P')$).
	\end{definition}
	\begin{definition}
		Given composable shapes $\gamma,\tau,{\gamma'}^T$, we define $\mathcal{P}_{\gamma,\tau,{\gamma'}^T}$ to be the set of all possible intersection patterns $P$ on $\gamma,\tau,{\gamma'}^T$ (up to equivalence)
	\end{definition}
	\begin{definition}
		Given composable (but not properly composable) ribbons $R_1$, $R_2$, $R_3$ of shapes $\gamma, \tau, {\gamma'}$, we define the intersection pattern $P \in \mathcal{P}_{\gamma,\tau,{\gamma'}^T}$ induced by $R_1,R_2,R_3$ as follows:
		\begin{enumerate}
			\item Take the canonical maps $\phi_{R_1}: V(\gamma) \to V(R_1)$, $\phi_{R_2}: V(\tau) \to V(R_2)$, and $\phi_{R_3}: V({\gamma'}^T) \to V(R_3)$
			\item Given vertices $u \in V(\gamma)$ and $v \in V(\tau)$, add a constraint edge between $u$ and $v$ if and only if $\phi_{R_1}(u) = \phi_{R_2}(v)$. Similarly, given vertices $u \in V(\gamma)$ and $w \in V({\gamma'}^T)$, add a constraint edge between $u$ and $w$ if and only if $\phi_{R_1}(u) = \phi_{R_3}(w)$ and given vertices $v \in V(\tau)$ and $w \in V({\gamma'}^T)$, add a constraint edge between $v$ and $w$ if and only if $\phi_{R_2}(v) = \phi_{R_3}(w)$.
		\end{enumerate}
	\end{definition}
	\begin{definition}
		Given an intersection pattern $P \in \mathcal{P}_{\gamma,\tau,{\gamma'}^T}$, we define $V(\gamma \circ \tau \circ {\gamma'}^T)/E(P)$ to be $V(\gamma \circ \tau \circ {\gamma'}^T)$ where all of the edges in $E(P)$ are contracted (i.e. if $(u,v) \in E(P)$ then $u = v$ and $u = v$ only appears once).
	\end{definition}
	\begin{definition}
		Given an intersection pattern $P \in \mathcal{P}_{\gamma,\tau,{\gamma'}^T}$, we define $\tau_{P}$ to be the shape such that:
		\begin{enumerate}
			\item $V(H_{\tau_P}) = V(\gamma \circ \tau \circ {\gamma'}^T)/E(P)$
			\item $E(H_{\tau_P}) = E(\gamma) \cup E(\tau) \cup E({\gamma'}^{T})$
			\item $U_{\tau_P} = U_{\gamma}$
			\item $V_{\tau_P} = V_{{\gamma'}^T}$
		\end{enumerate}
	\end{definition}
	\begin{definition}
		Given an intersection pattern $P \in \mathcal{P}_{\gamma,\tau,{\gamma'}^T}$, we make the following definitions:
		\begin{enumerate}
			\item We define $Aut(P) = \{\pi \in Aut(\gamma \circ \tau \circ {\gamma'}^T): \pi(E(P)) = E(P)\}$
			\item We define $Aut_{pieces}(P) = \{\pi \in Aut(U_{\gamma}) \times Aut(\tau) \times Aut({\gamma'}^T): \pi(E(P)) = E(P)\}$
			\item We define $N(P) = |Aut(P)/Aut_{pieces}(P)|$
		\end{enumerate}
	\end{definition}
	\begin{lemma}
		For all composable $\sigma$, $\tau$, and ${\sigma'}^T$ (inclulding improper $\tau$), 
		\begin{align*}
			&M^{fact}_{\tau}(e_{\sigma}e^T_{\sigma'}) - M^{orth}_{\tau}(e_{\sigma}e^T_{\sigma'}) = \sum_{\sigma_2, \gamma: \gamma \text{ is non-trivial }, \atop \sigma_2 \cup \gamma = \sigma}{\frac{1}{|Aut(U_{\gamma})|}\sum_{P \in \mathcal{P}_{\gamma,\tau,Id_{V_{\tau}}}}N(P)M^{orth}_{\tau_P}(e_{\sigma_2}e^T_{\sigma'})} \\
			&+ \sum_{\sigma'_2, \gamma': \gamma' \text{ is non-trivial }, \atop \sigma'_2 \cup \gamma' = \sigma'}{\frac{1}{|Aut(U_{\gamma'})|}\sum_{P \in \mathcal{P}_{Id_{U_{\tau}},\tau,{\gamma'}^T}}N(P)M^{orth}_{\tau_P}(e_{\sigma}e^T_{\sigma'_2})} \\
			&+ \sum_{\sigma_2, \gamma: \gamma \text{ is non-trivial }, \atop \sigma_2 \cup \gamma = \sigma}{\sum_{\sigma'_2, \gamma': \gamma' \text{ is non-trivial }, \atop \sigma'_2 \cup \gamma' = \sigma'}{
					\frac{1}{|Aut(U_{\gamma})|\cdot|Aut(U_{\gamma'})|}\sum_{P \in \mathcal{P}_{\gamma,\tau,{\gamma'}^T}}N(P)M^{orth}_{\tau_P}(e_{\sigma_2}e^T_{\sigma'_2})}}
		\end{align*}
	\end{lemma}
	\begin{proof}
		This lemma follows from the following bijection. Consider the third term
		\[
		\sum_{\sigma_2, \gamma: \gamma \text{ is non-trivial }, \atop \sigma_2 \cup \gamma = \sigma}{\sum_{\sigma'_2, \gamma': \gamma' \text{ is non-trivial }, \atop \sigma'_2 \cup \gamma' = \sigma'}{
				\frac{1}{|Aut(U_{\gamma})|\cdot|Aut(U_{\gamma'})|}\sum_{P \in \mathcal{P}_{\gamma,\tau,{\gamma'}^T}}N(P)M^{orth}_{\tau_P}(e_{\sigma_2}e^T_{\sigma'_2})}}
		\]
		On one side, we have the following data:
		\begin{enumerate}
			\item Ribbons $R_1$, $R_2$, and $R_3$ such that 
			\begin{enumerate}
				\item $R_1,R_2,R_3$ have shapes $\sigma$, $\tau$, and ${\sigma'}^T$, respectively.
				\item $A_{R_2} = B_{R_1}$ and $A_{R_3} = B_{R_2}$
				\item $\left(V(R_1) \cup V(R_2)\right) \cap V(R_3) \neq A_{R_3}$ and $\left(V(R_2) \cup V(R_3)\right) \cap V(R_1) \neq B_{R_1}$
			\end{enumerate}
			\item An ordering $O_{S'}$ on the leftmost minimum vertex separator $S'$ between $A_{R_1}$ and $V_{*} \cup B_{R_1}$.
			\item An ordering $O_{T'}$ on the rightmost minimum vertex separator $S'$ between $V_{*} \cup A_{R_3}$ and $B_{R_3}$.
		\end{enumerate}
		On the other side, we have the following data
		\begin{enumerate}
			\item An intersection pattern $P \in \mathcal{P}_{\gamma,\tau,{\gamma'}^T}$ where $\gamma$ and ${\gamma'}^T$ are non-trivial.
			\item Ribbons $R'_1$, $R'_2$, $R'_3$ of shapes $\sigma_2$, $\tau_P$, ${\sigma'_2}^T$ such that $V(R'_1) \cap V(R'_2) = A_{R'_2} = B_{R'_1}$, $V(R'_2) \cap V(R'_3) = B_{R'_2} = A_{R'_3}$, and $V(R'_1) \cap V(R'_3) = A_{R'_2} \cap B_{R'_2}$
			\item An element $\pi \in Aut(P)/Aut_{pieces}(P)$
		\end{enumerate}
		To see this bijection, given $R_1,R_2,R_3$, we again implement our strategy for analyzing intersection terms. Recall that $V_{*}$ is the set of vertices in $V(R_1) \cup V(R_2) \cup V(R_3)$ which have an unexpected equality with another vertex, $S'$ is the leftmost minimum vertex separator between $A_{R_1}$ and $B_{R_1} \cup V_{*}$, and $T'$ is the rightmost minimum vertex separator between $A_{R_3} \cup V_{*}$ and $B_{R_3}$.
		\begin{enumerate}
			\item Decompose $R_1$ as $R_1 = {R'}_1 \circ R_4$ where ${R'}_1$ is the part of $R_1$ between $A_{R_1}$ and $(S',O_{S'})$ and $R_4$ is the part of $R_1$ between $(S',O_{S'})$ and $B_{R_1} = A_{R_2}$. Decompose $R_3$ as $R_5 \cup R'_3$ where $R_5$ is the part of $R_3$ between $A_{R_3}$ and $(T',O_{T'})$ and $R'_3$ is the part of $R_3$ between $(T',O_{T'})$ and $B_{R_3}$
			\item Take the intersection pattern $P$ and the ribbon $R'_2$ induced by $R_4$, $R_2$, and $R_5$.
			\item Observe that we have two bijective maps from $V(\gamma \circ \tau \circ {\gamma'}^T)/E(P)$ to $V(R_4) \cup V(R_2) \cup V(R_5)$. The first map is $\phi_{R_4} \circ \phi_{R_2} \circ \phi_{R_5}$ and the second map is $\phi_{R'_2}$. We take $\pi = \phi^{-1}_{R'_2}(\phi_{R_4} \circ \phi_{R_2} \circ \phi_{R_5})$.
		\end{enumerate}
		Conversely, given an intersection pattern $P \in \mathcal{P}_{\gamma,\tau,{\gamma'}^T}$, $R'_1$, $R'_2$, $R'_3$, and an element $\pi \in Aut(P)/Aut_{pieces}(P)$:
		\begin{enumerate}
			\item Take $R_4 = \phi_{R'_2}\pi(V(\gamma))$, $R_2 = \phi_{R'_2}\pi(V(\tau))$, and $R_5 = \phi_{R'_2}\pi(V({\gamma'}^T))$.
			\item Take $R_1 = R'_1 \cup R_4$ and take $R_3 = R_5 \cup R'_3$.
			\item Take $O_S$ and $O_T$ based on $B_{R'_1} = A_{R_4}$ and $B_{R_5} = A_{R'_3}$.
		\end{enumerate}
		To confirm that this is a bijection, we need to show that these maps are inverses of each other.
		
		If we apply the first map and then the second, we obtain the following:
		\begin{enumerate}
			\item We obtain the ribbons 
			\begin{enumerate}
				\item $R''_1 = R'_1 \circ \phi_{R'_2}\phi^{-1}_{R'_2}(\phi_{R_4} \circ \phi_{R_2} \circ \phi_{R_5})(V(\gamma))$
				\item $R''_2 = \phi_{R'_2}\phi^{-1}_{R'_2}(\phi_{R_4} \circ \phi_{R_2} \circ \phi_{R_5})(V(\tau))$
				\item $R''_3 = \phi_{R'_2}\phi^{-1}_{R'_2}(\phi_{R_4} \circ \phi_{R_2} \circ \phi_{R_5})(V({\gamma'}^T)) \circ R'_3$
			\end{enumerate} 
			where 
			\begin{enumerate}
				\item $R'_1$ is the part of $R_1$ between $A_{R_1}$ and $(S',O_{S'})$ where $S'$ is the minimum vertex separator between $A_{R_1}$ and $V_{*} \cup B_{R_1}$.
				\item $R_4$ is the part of $R_1$ between $(S',O_{S'})$ and $B_{R_1}$
				\item $R'_2$ is the ribbon of shape $\tau_{P}$ induced (along with the intersection pattern $P$) by $R_1$, $R_2$, and $R_3$.
				\item $R_5$ is the part of $R_3$ between $A_{R_3}$ and $(T',O_{T'})$.
				\item $R'_3$ is the part of $R_3$ between $(T',O_{T'})$ and $B_{R_3}$
			\end{enumerate}
			This implies that $R''_1 = R'_1 \circ R_4 = R_1$, $R''_2 = R_2$, and $R''_3 = R_5 \circ R'_3 = R_3$. Since the second map leaves $R'_1$ and $R'_3$ unchanged, we recover the orderings $O_S$ and $O_T$ as well.
		\end{enumerate}
		
		Conversely, if we apply the second map, we have that $R_1 = R'_1 \circ \phi_{R'_2}\pi(V(\gamma))$, $R_2 = \phi_{R'_2}\pi(V(\tau))$, and $R_3 = \phi_{R'_2}\pi(V({\gamma'}^T)) \circ R'_3$ and we have the orderings $O_S$ and $O_T$ corresponding to $B_{R'_1}$ and $A_{R'_3}$ respectively. If we apply the first map, 
		\begin{enumerate}
			\item $R'_1$ and $R'_3$ are preserved.
			\item $R''_2$ and $P''$ are the ribbon and intersection pattern induced by the ribbons $\phi_{R'_2}\pi(\gamma)$, $\phi_{R'_2}\pi(\tau)$, and $\phi_{R'_2}\pi({\gamma'}^T)$. To see that $R''_2 = R'_2$, observe that 
			\[
			R''_2 = \phi_{R'_2}\pi(V(\gamma)) \circ \phi_{R'_2}\pi(V(\tau)) \circ \phi_{R'_2}\pi(V({\gamma'}^T)) = \phi_{R'_2}{\pi(\gamma \circ \tau \circ {\gamma'}^T)} = \phi_{R_2}(\gamma \circ \tau \circ {\gamma'}^T) = R'_2
			\]
			To see that $P'' \equiv P$, observe that:
			\begin{enumerate}
				\item We have two bijective maps from $V(\gamma)$ to $V(\phi_{R'_2}\pi(\gamma))$. These two maps are $\phi_{R'_2}\pi$ and $\phi_{\phi_{R'_2}\pi(\gamma)}$.
				\item We have two bijective maps from $V(\tau)$ to $V(\phi_{R'_2}\pi(\tau))$. These two maps are $\phi_{R'_2}\pi$ and $\phi_{\phi_{R'_2}\pi(\tau)}$.
				\item We have two bijective maps from $V({\gamma'}^T)$ to $V(\phi_{R'_2}\pi({\gamma'}^T))$. These two maps are $\phi_{R'_2}\pi$ and $\phi_{\phi_{R'_2}\pi({\gamma'}^T)}$.
				\item For $P''$, the constraint edges are 
				\[
				\left(\phi^{-1}_{\phi_{R'_2}\pi(\gamma)}\phi_{R'_2}\pi \circ \phi^{-1}_{\phi_{R'_2}\pi(\tau)}\phi_{R'_2}\pi \circ \phi^{-1}_{\phi_{R'_2}\pi({\gamma'}^T))}\phi_{R'_2}\pi\right)(E(P))
				\]
			\end{enumerate}
			\item We have that 
			\[
			\pi'' = \phi^{-1}_{R'_2}(\phi_{\phi_{R'_2}\pi(V(\gamma))} \circ \phi_{\phi_{R'_2}\pi(V(\tau))} \circ \phi_{\phi_{R'_2}\pi(V({\gamma'}^T))})
			\]
			To see that $\pi'' \equiv \pi$, note that 
			\[
			\pi = \pi''\left(\phi^{-1}_{\phi_{R'_2}\pi(V(\gamma))}\phi_{R'_2}\pi \circ \phi^{-1}_{\phi_{R'_2}\pi(V(\tau))}\phi_{R'_2}\pi \circ \phi^{-1}_{\phi_{R'_2}\pi(V({\gamma'}^T))}\phi_{R'_2}\pi)\right)
			\]
		\end{enumerate}
		The analysis for the the first term is the same except that when $\gamma'$ is trivial, we always take $\gamma'$ to be the identity so $T = V(V_{\tau}) = V(U_{{\sigma'}^T})$ and the ordering $O_{T}$ is given by $V_{\tau} = U_{{\sigma'}^T}$. 
		Similarly, the analysis for the the second term is the same except that when $\gamma$ is trivial, we always take $\gamma$ to be the identity so $S = V(V_{\sigma}) = V(U_{\tau})$ and the ordering $O_{S}$ is given by $V_{\sigma} = U_{\tau}$.
	\end{proof}

\section{Degree 4 Planted Clique Analysis}\label{sec: deg_4_planted_clique}
For this example, we name the shapes based on what they look like to make them easier to keep track of. With the exception of $Id_{U}$, these names only appear in this section.
\subsection{The shapes $\alpha$ and coefficients $\lambda_{\alpha}$}
After several preprocessing steps, the moment matrix which needs to be analyzed is $M \approx \sum_{\alpha}{\lambda_{\alpha}M_{\alpha}}$ for the following shapes $\alpha$ and coefficients $\lambda_{\alpha}$
\begin{definition} \ 
\begin{enumerate}
\item Given $E \subseteq \{(u_1,v_1), (u_1,v_2), (u_2,v_1), (u_2,v_2)\}$, we define $\alpha_{E}$ to be the shape where $U_{\alpha_E} = (u_1,u_2)$, $V_{\alpha_E} = (v_1,v_2)$, and $E(\alpha) = E$.
\item Given $E \subseteq \{(u_1,v_1), (u_1,v_2), (u_2,v_1), (u_2,v_2)\}$, we define $\alpha_{X,E}$ to be the shape where $U_{\alpha_E} = (u_1,u_2)$, $V_{\alpha_E} = (v_1,v_2)$, there is one additional vertex $w_1$, and $E(\alpha) = E \cup \{(u_1,w_1), (u_2,w_1), (w_1,v_1), (w_1,v_2)\}$.
\item Given $i,j \in \{1,2\}$, we define $\alpha_{u_i = v_j,e}$ to be the shape where $U_{\alpha_{u_i = v_j,e}} = (u_1,u_2)$, $V_{\alpha_{u_i = v_j,e}} = (v_1,v_2)$, $u_i = v_j$, and $E(\alpha_{u_i = v_j,e}) = \{(u_{2-i},v_{2-j})\}$.
\item Given $i,j \in \{1,2\}$, we define $\alpha_{u_i = v_j,\emptyset}$ to be the shape where $U_{\alpha_E} = (u_1,u_2)$, $V_{\alpha_E} = (v_1,v_2)$, $u_i = v_j$, and $E(\alpha) = \emptyset$.
\item We define $\alpha_{Id:} = Id_{(u_1,u_2)}$ to be the shape where $U_{Id_{(u_1,u_2)}} = V_{Id_{(u_1,u_2)}} = (u_1,u_2)$ and $E(Id_{(u_1,u_2)}) = \emptyset$.
\item We define $\alpha_{swap}$ to be the shape where $U_{\alpha_{swap}} = (u_1,u_2)$, $V_{\alpha_{swap}} = (u_2,u_1)$ and $E(\alpha_{swap}) = \emptyset$.
\end{enumerate}
\end{definition}
For illustrations of these shapes $\alpha$, see Figures \ref{zerointersectionalphasfigure}.\\
\begin{figure}[ht]\label{zerointersectionalphasfigure}
\centerline{\includegraphics[height=4cm]{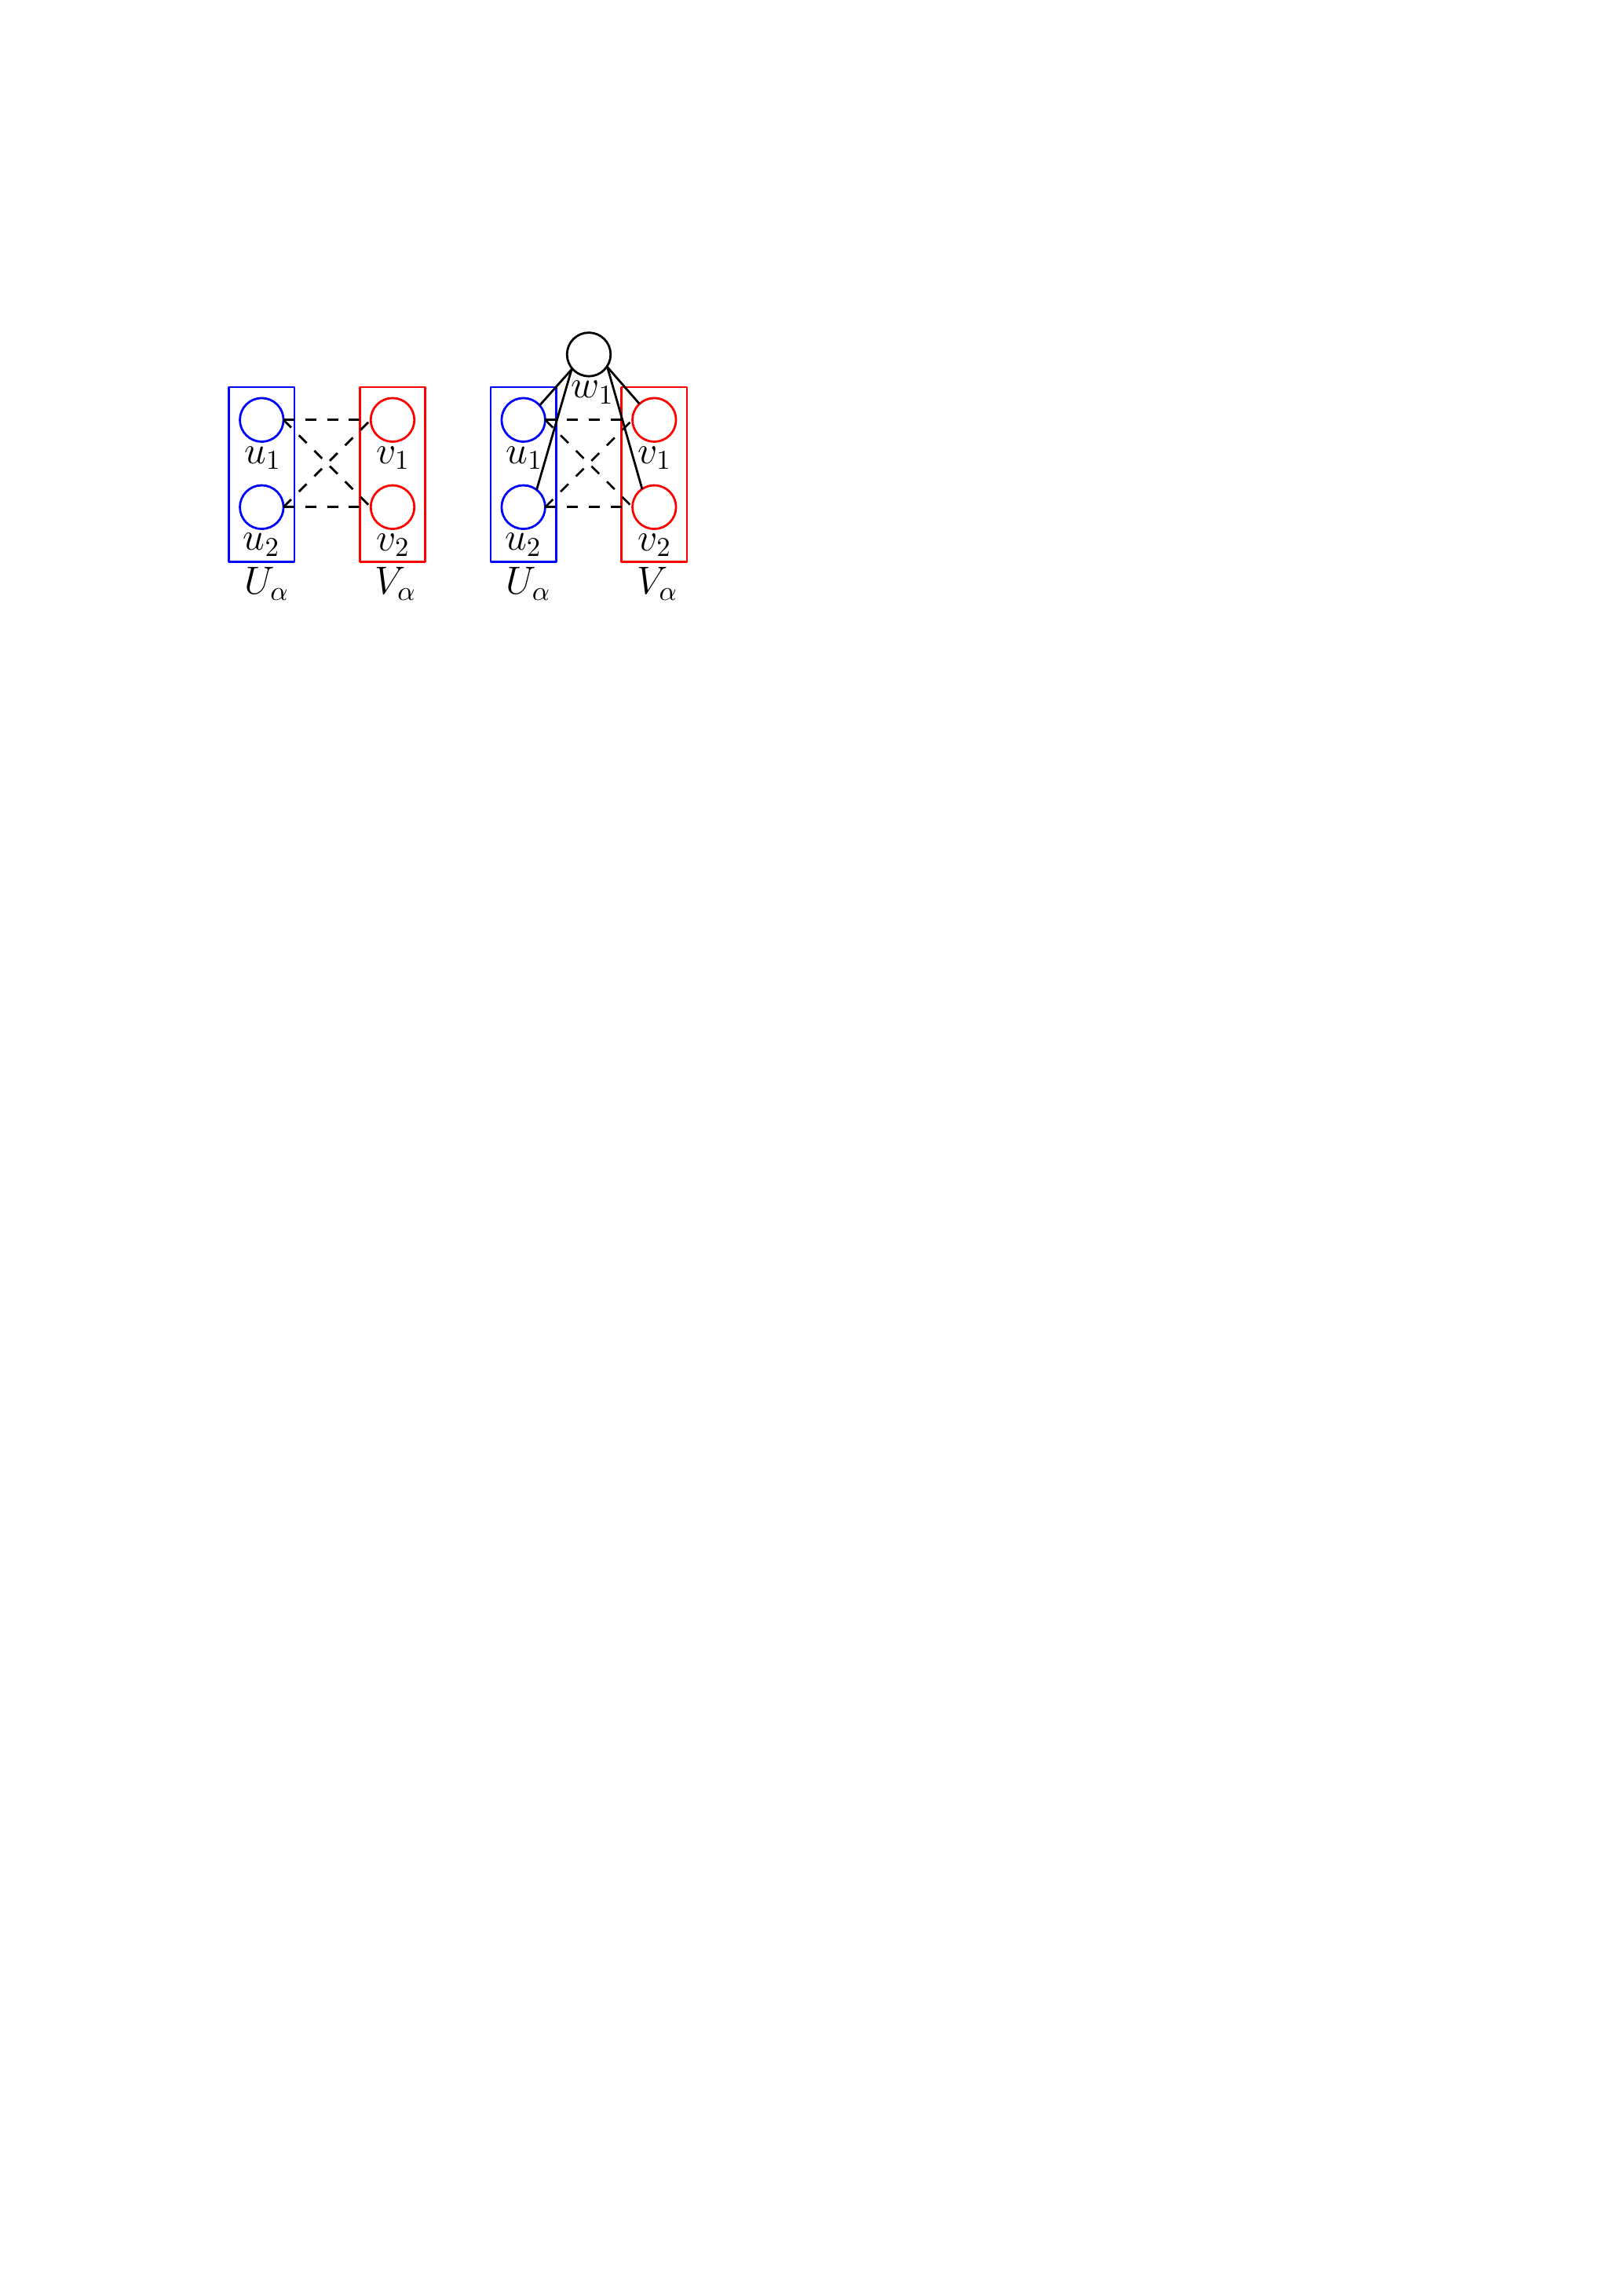}}
\caption{This figure shows the shapes $\alpha$ where $|U_{\alpha} \cap V_{\alpha}| = 0$. On the left we have $\alpha_{E}$ and on the right we have $\alpha_{X,E}$.}
\end{figure}
\begin{figure}[ht]\label{oneintersectionalphasfigure}
\centerline{\includegraphics[height=4cm]{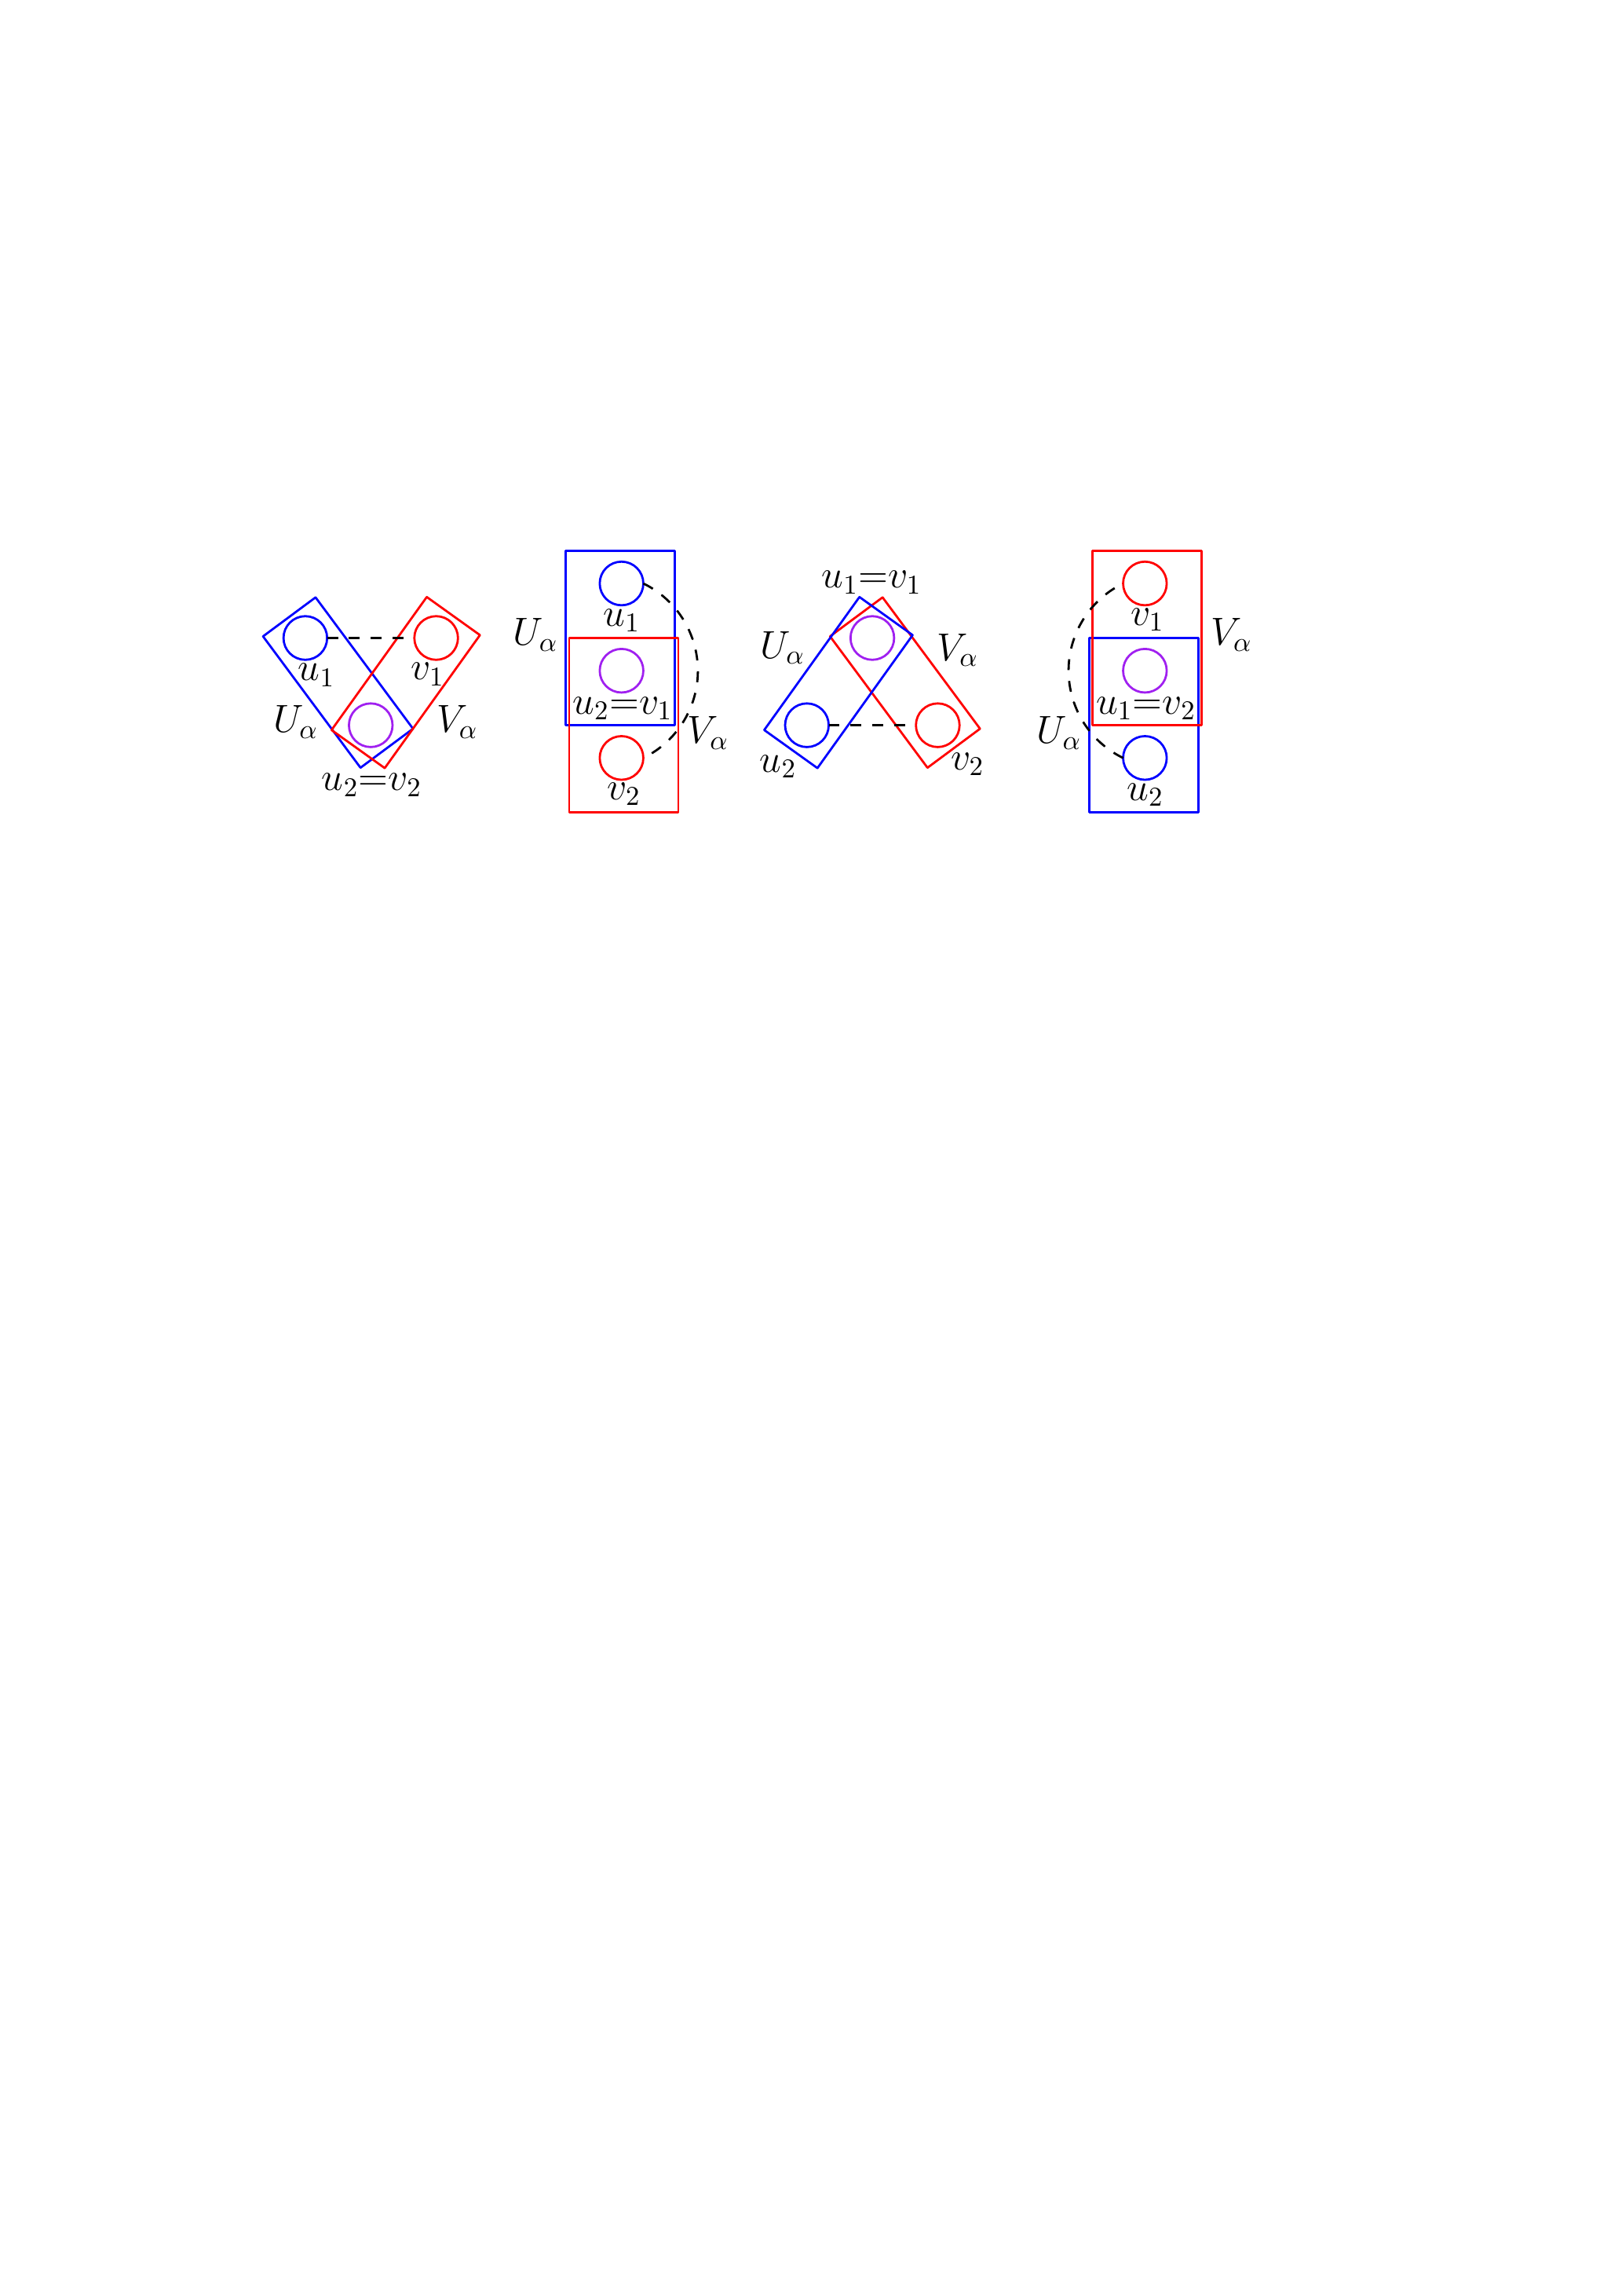}}
\caption{This figure shows the shapes $\alpha$ where $|U_{\alpha} \cap V_{\alpha}| = 1$. From left to right, we have $\alpha_{u_2 = v_2,\emptyset}$ and $\alpha_{u_2 = v_2,e}$, $\alpha_{u_2 = v_1,\emptyset}$ and $\alpha_{u_2 = v_1,e}$, $\alpha_{u_1 = v_1,\emptyset}$ and $\alpha_{u_1 = v_1,e}$, and $\alpha_{u_1 = v_2,\emptyset}$ and $\alpha_{u_1 = v_2,e}$.}
\end{figure}
\begin{figure}[ht]\label{twointersectionalphasfigure}
\centerline{\includegraphics[height=4cm]{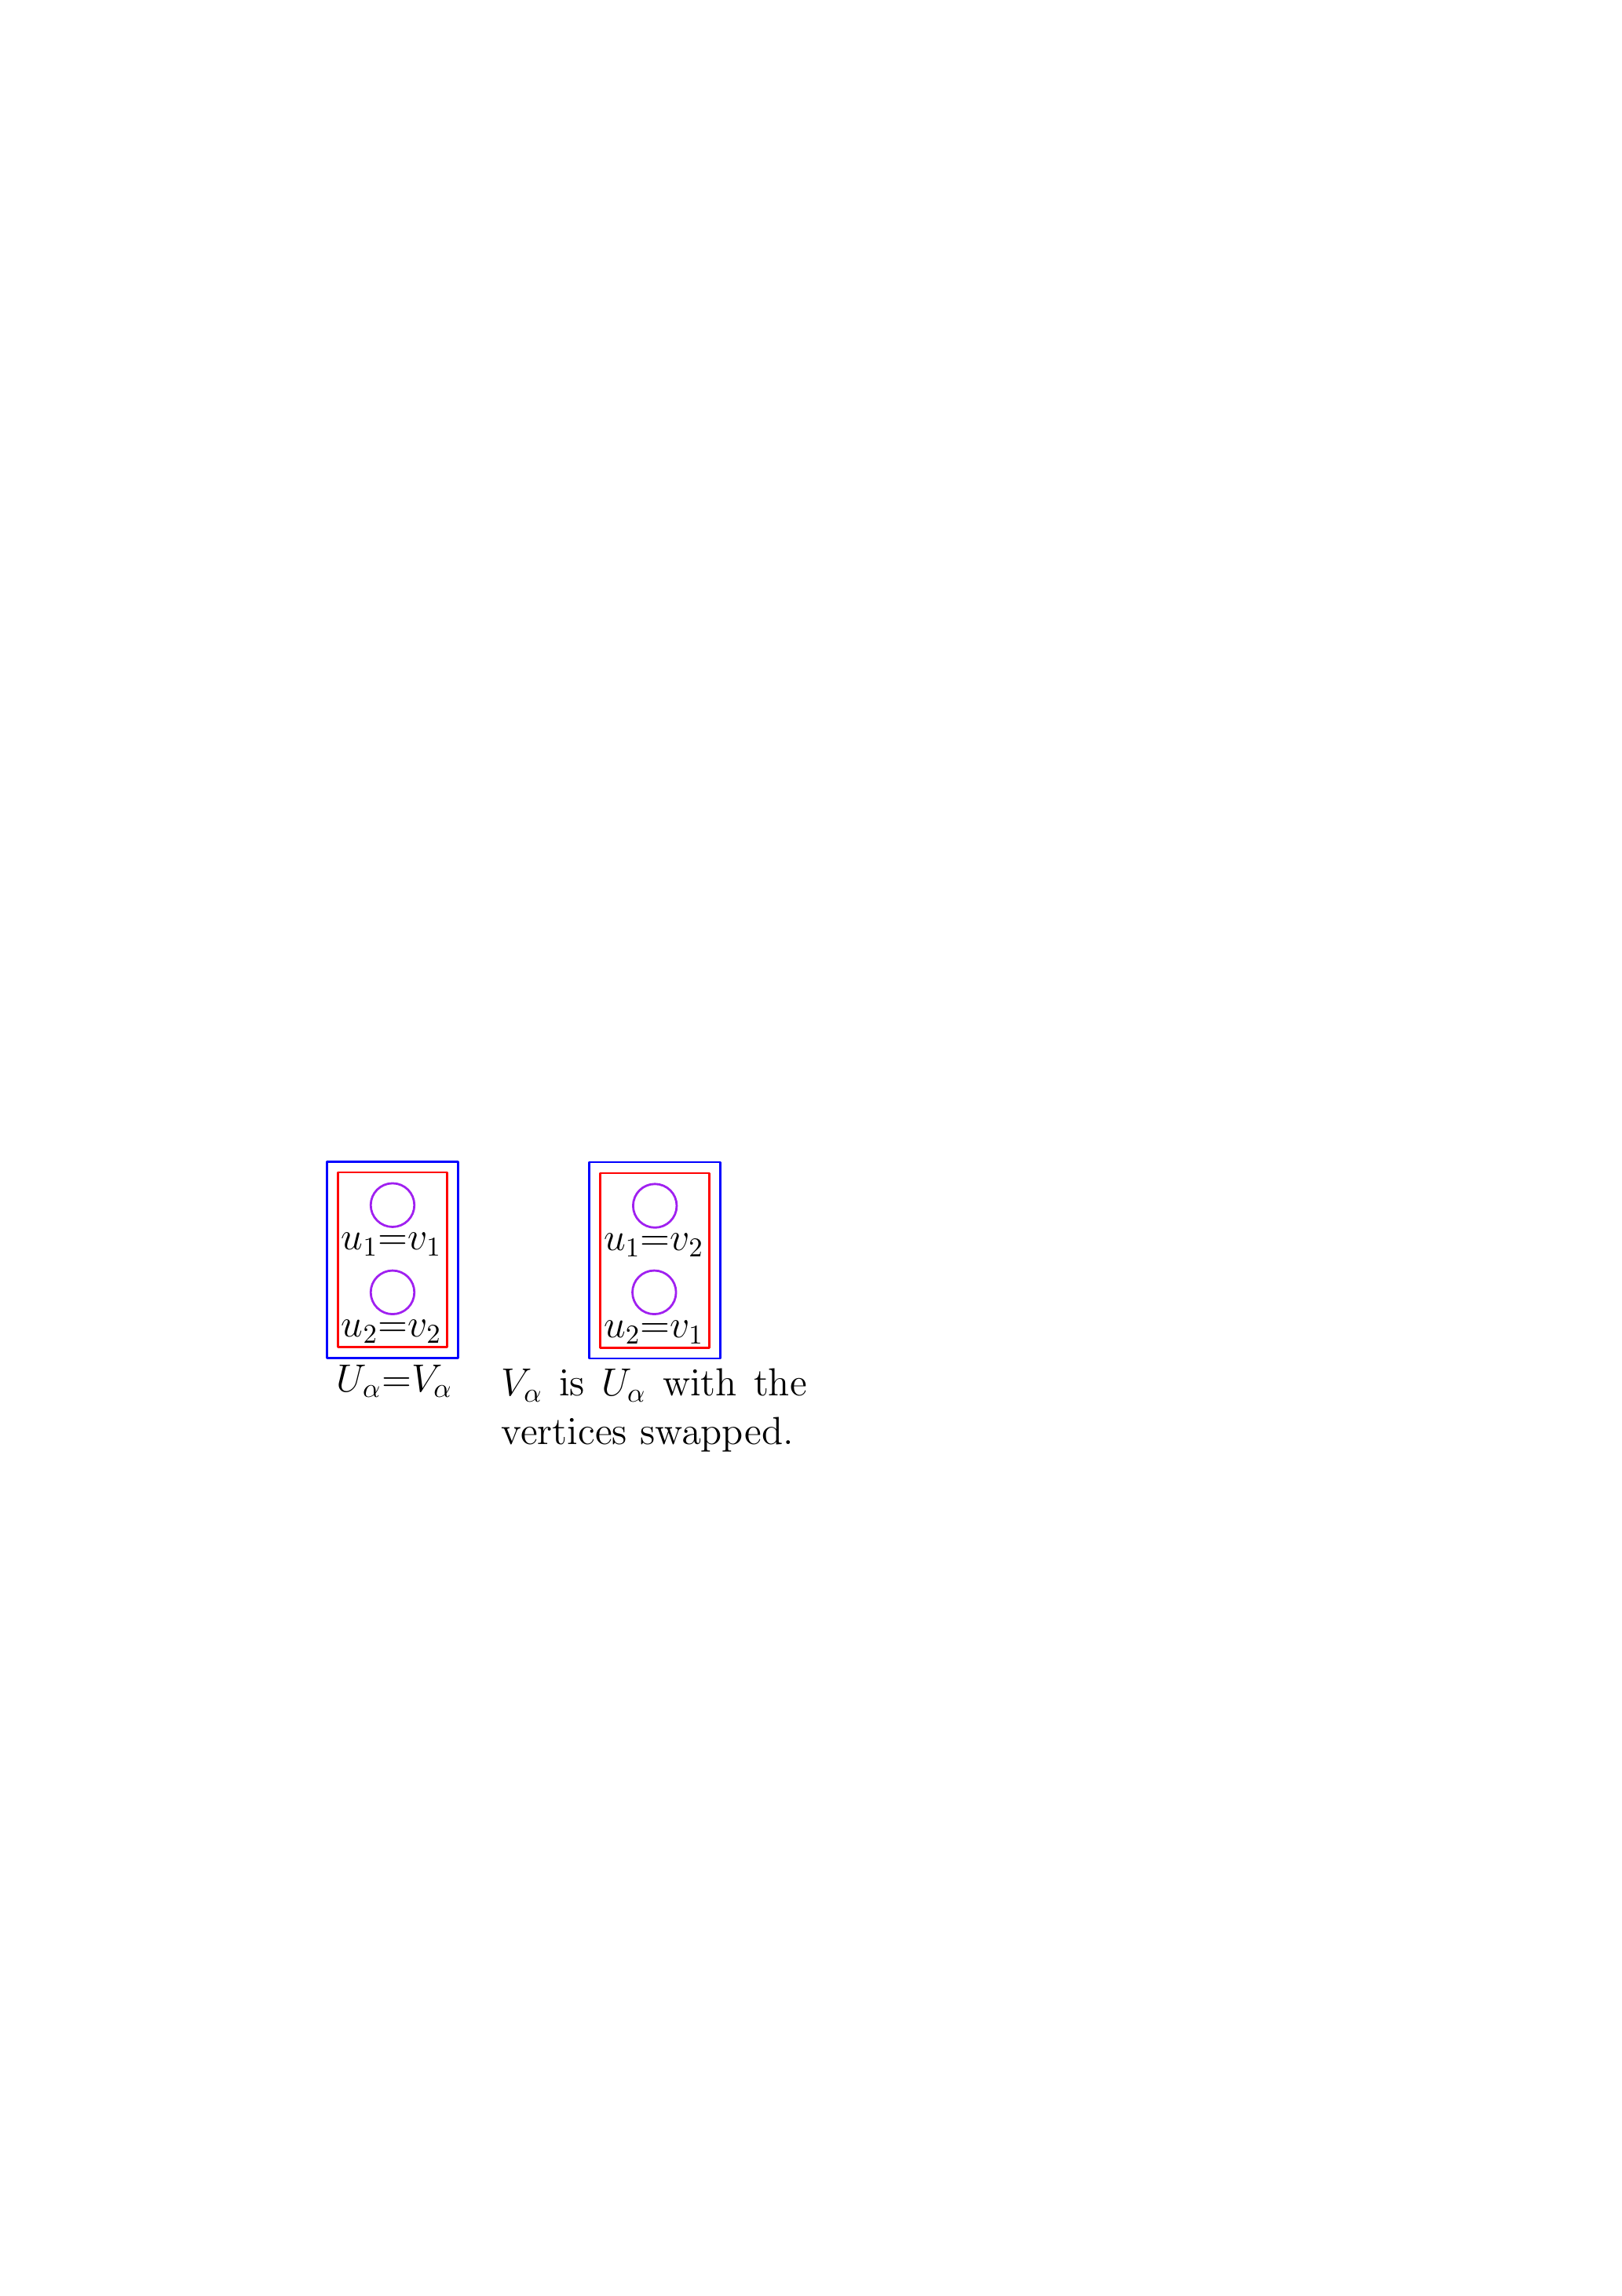}}
\caption{This figure shows the shapes $\alpha$ where $|U_{\alpha} \cap V_{\alpha}| = 2$. On the left we have $\alpha_{Id:}$ and on the right we have $\alpha_{swap}$.}
\end{figure}
We have the following coefficients on these shapes.
\begin{enumerate}
\item For each $E \subseteq \{(u_1,v_1), (u_1,v_2), (u_2,v_1), (u_2,v_2)\}$, $\lambda_{\alpha_E} = \frac{k^4}{n^4}$.
\item For each $E \subseteq \{(u_1,v_1), (u_1,v_2), (u_2,v_1), (u_2,v_2)\}$, $\lambda_{\alpha_{X,E}} = C\frac{k^5}{n^5}$ for some constant $C > 1$. These coefficients are the ad-hoc fix to the candidate pseudo-expectation values for planted clique in \cite{meka2015sum}.
\item For each $i,j \in \{1,2\}$, $\lambda_{\alpha_{u_i = v_j,e}} = \lambda_{\alpha_{u_i = v_j,\emptyset}} = \frac{k^3}{n^3}$.
\item $\lambda_{\alpha_{Id:}} = \lambda_{\alpha_{swap}} = \frac{k^2}{n^2}$
\end{enumerate}
\subsection{Decomposing $\alpha$ and coefficient matrices}
To find the coefficient matrices $H_{Id_{\emptyset}}$, $H_{Id_{(u_1)}}$, $H_{Id_{(u_1,u_2)}}$, and $H_{\tau}$, we need to decompose each $\alpha$ into a left part $\sigma$, a proper middle part $\tau$, and a right part ${\sigma'}^T$. 

The following left shapes will appear in these decompositions
\begin{definition} \ 
\begin{enumerate}
\item Define $\sigma_{Id:} = Id_{(u_1,u_2)}$. Note that $\sigma_{Id:} = \alpha_{Id:}$ but it is playing a different role.
\item Define $\sigma_{swap} = \alpha_{swap}$.
\item Define $\sigma_7$ to be the shape where $U_{\sigma_{7}} = (u_1,u_2)$, $V_{\sigma_{7}} = (v_1)$, and $E(\sigma_{7}) = \{(u_1,v_1),(u_2,v_1)\}$.
\item Define $\sigma_{u_1,u_2 \to u_1}$ to be the shape where $U_{\sigma_{u_1,u_2 \to u_1}} = (u_1,u_2)$, $V_{\sigma_{u_1,u_2 \to u_1}} = (u_1)$, and $E(\sigma_{u_1,u_2 \to u_1}) = \emptyset$.
\item Similarly, define $\sigma_{u_1,u_2 \to u_2}$ to be the shape where $U_{\sigma_{u_1,u_2 \to u_2}} = (u_1,u_2)$, $V_{\sigma_{u_1,u_2 \to u_2}} = (u_2)$, and $E(\sigma_{u_1,u_2 \to u_2}) = \emptyset$.
\item Define $\sigma_{u_1,u_2 \to \emptyset}$ to be the shape where $U_{\sigma_{u_1,u_2 \to \emptyset}} = (u_1,u_2)$, $V_{\sigma_{u_1,u_2 \to \emptyset}} = \emptyset$, and $E(\sigma_{u_1,u_2 \to \emptyset}) = \emptyset$.
\end{enumerate}
\end{definition}
These left shapes are illustrated in Figure \ref{onerightsidevertexsigmasfigure}. \\
\begin{figure}[ht]\label{onerightsidevertexsigmasfigure}
\centerline{\includegraphics[height=4cm]{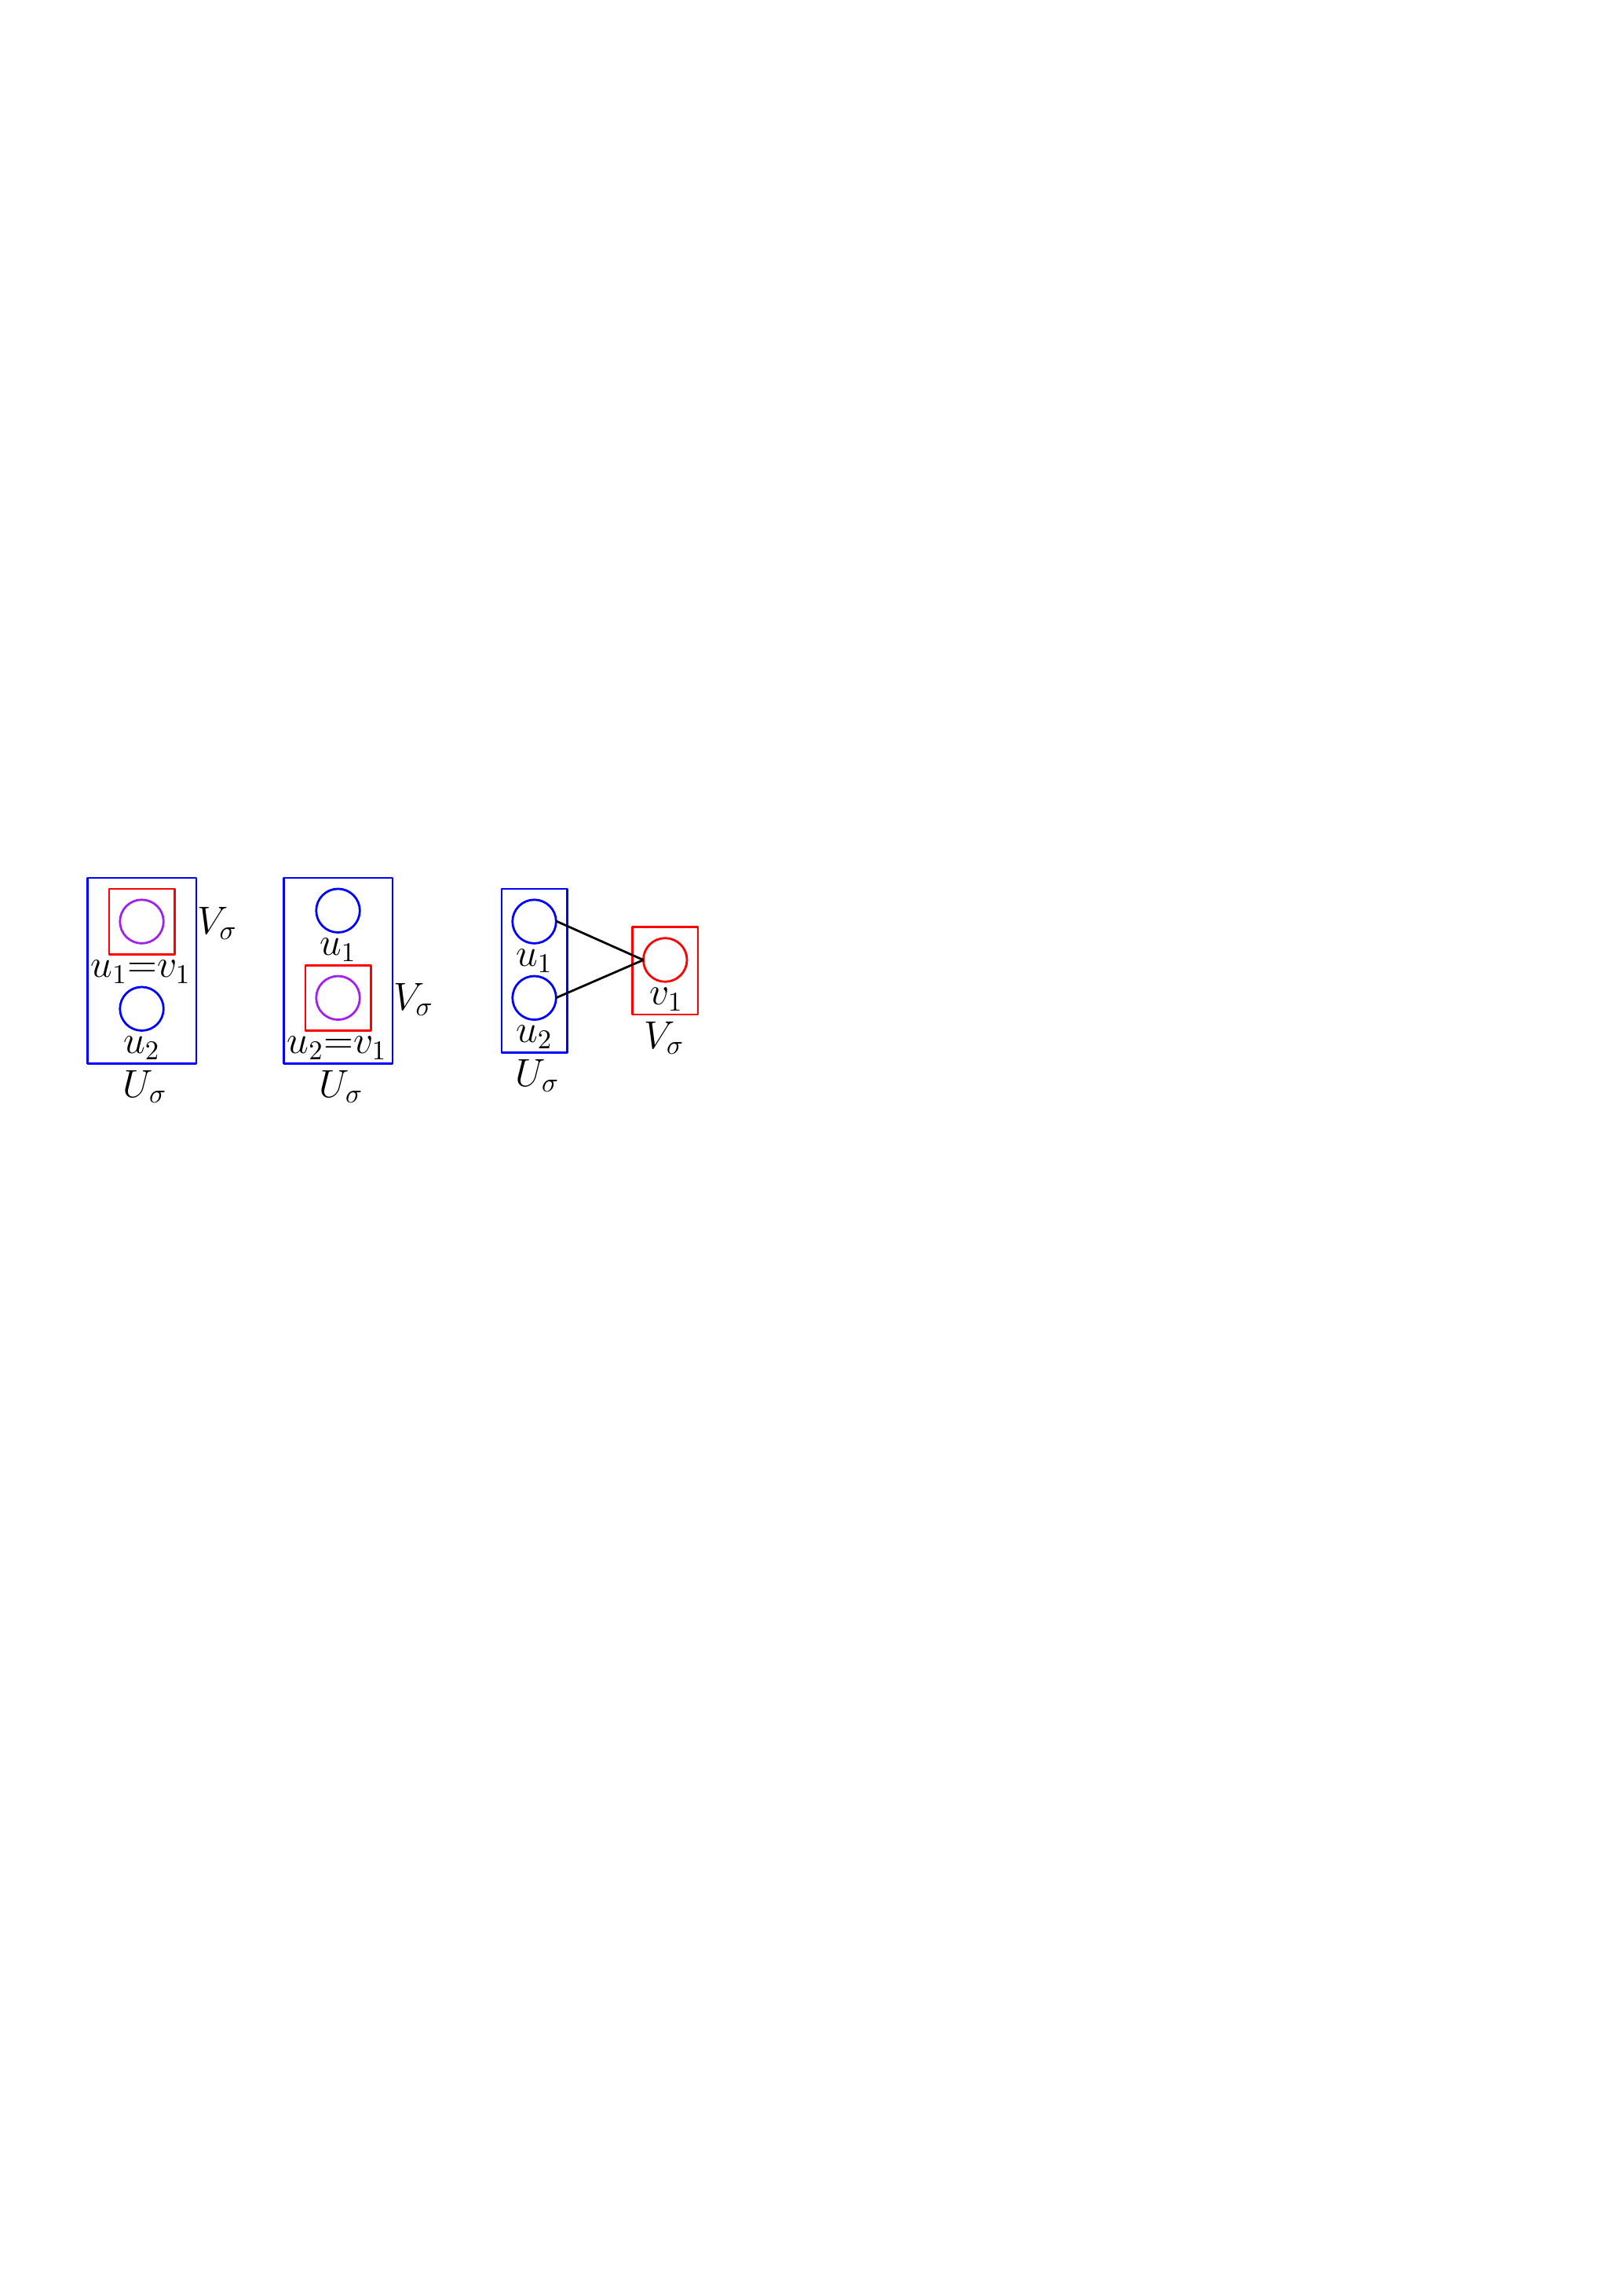}}
\caption{This figure shows the left shapes $\sigma$ where $|V_{sigma}| = 1$. From left to right we have $\sigma_{u_1,u_2 \to u_1}$, $\sigma_{u_1,u_2 \to u_2}$, and $\sigma_7$.}
\end{figure}
\begin{figure}[ht]\label{zeroortworightvertexsigmasfigure}
\centerline{\includegraphics[height=4cm]{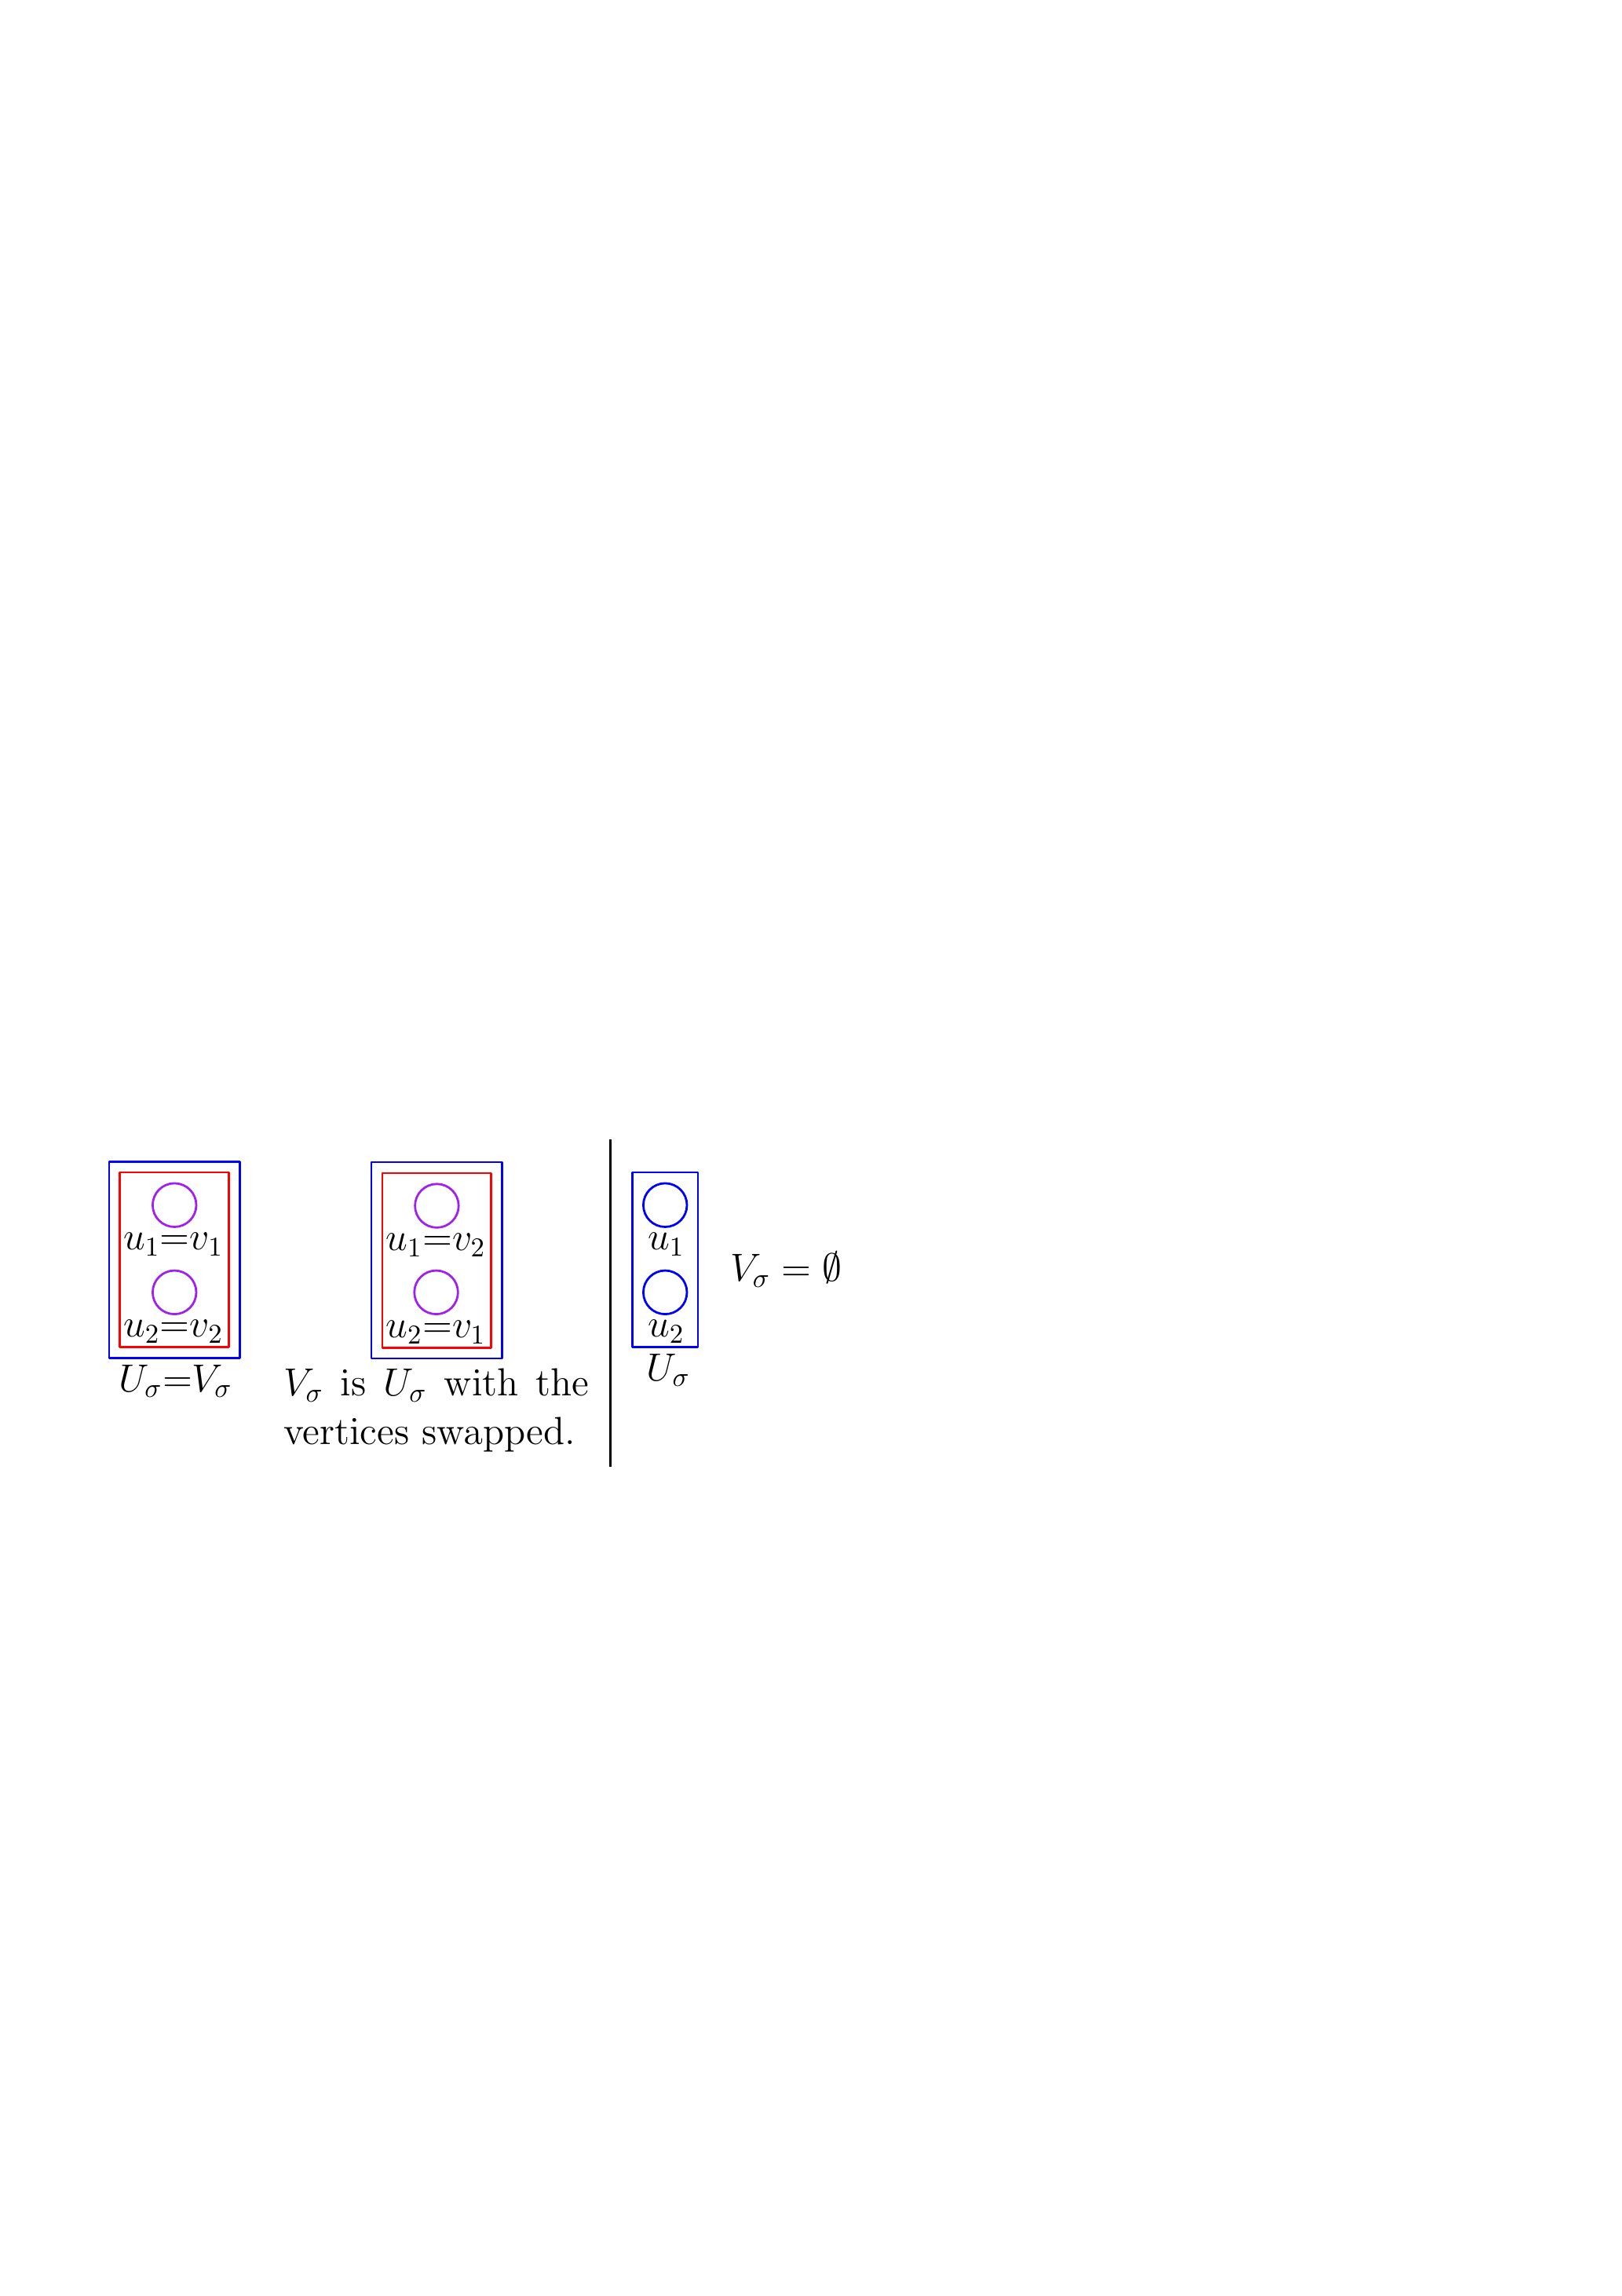}}
\caption{This figure shows the left shapes $\sigma$ where $|V_{\sigma}| = 2$ or $|V_{\sigma}| = 0$. On the left we have $\sigma_{Id:}$ and $\sigma_{swap}$. On the right we have $\sigma_{u_1,u_2 \to \emptyset}$.}
\end{figure}

The following proper middle shapes will appear in these decompositions.
\begin{definition} \ 
\begin{enumerate}
\item Define $\tau_{Id:} = Id_{(u_1,u_2)}$
\item Given $E \subseteq \{(u_1,v_1), (u_1,v_2), (u_2,v_1), (u_2,v_2)\}$ such that all four vertices $u_1,u_2,v_1,v_2$ are incident to at least one edge in $E$, we define $\tau_{E} = \alpha_{E}$.
\item Given $E \subseteq \{(u_1,v_1), (u_1,v_2), (u_2,v_1), (u_2,v_2)\}$ such that $E \neq \emptyset$, we define $\tau_{X,E} = \alpha_{X,E}$.
\item Given $i,j \in \{1,2\}$, we define $\tau_{u_i = v_j,e} = \alpha_{u_i = v_j,e}$.
\item Define $\tau_{Id\cdot} = Id_{(u_1)}$ to be the shape where $U_{Id_{(u_1)}} = V_{Id_{(u_1)}} = (u_1)$ and $E(Id_{(u_1)}) = \emptyset$.
\item Define $\tau_{e}$ to be the shape where $U_{\tau_{e}} = (u_1)$, $V_{\tau_{e}} = (v_1)$, and $E(\tau_{e}) = \{(u_1,v_1)\}$.
\item Define $\tau_{\emptyset}$ to be the empty shape with no vertices. 
\end{enumerate}
\end{definition}
These proper middle shapes (except for $\tau_{\emptyset}$) are illustrated in Figure \ref{twovertexseparatortausfigure}. \\
\begin{figure}[ht]\label{twovertexseparatortausfigure}
\centerline{\includegraphics[height=8cm]{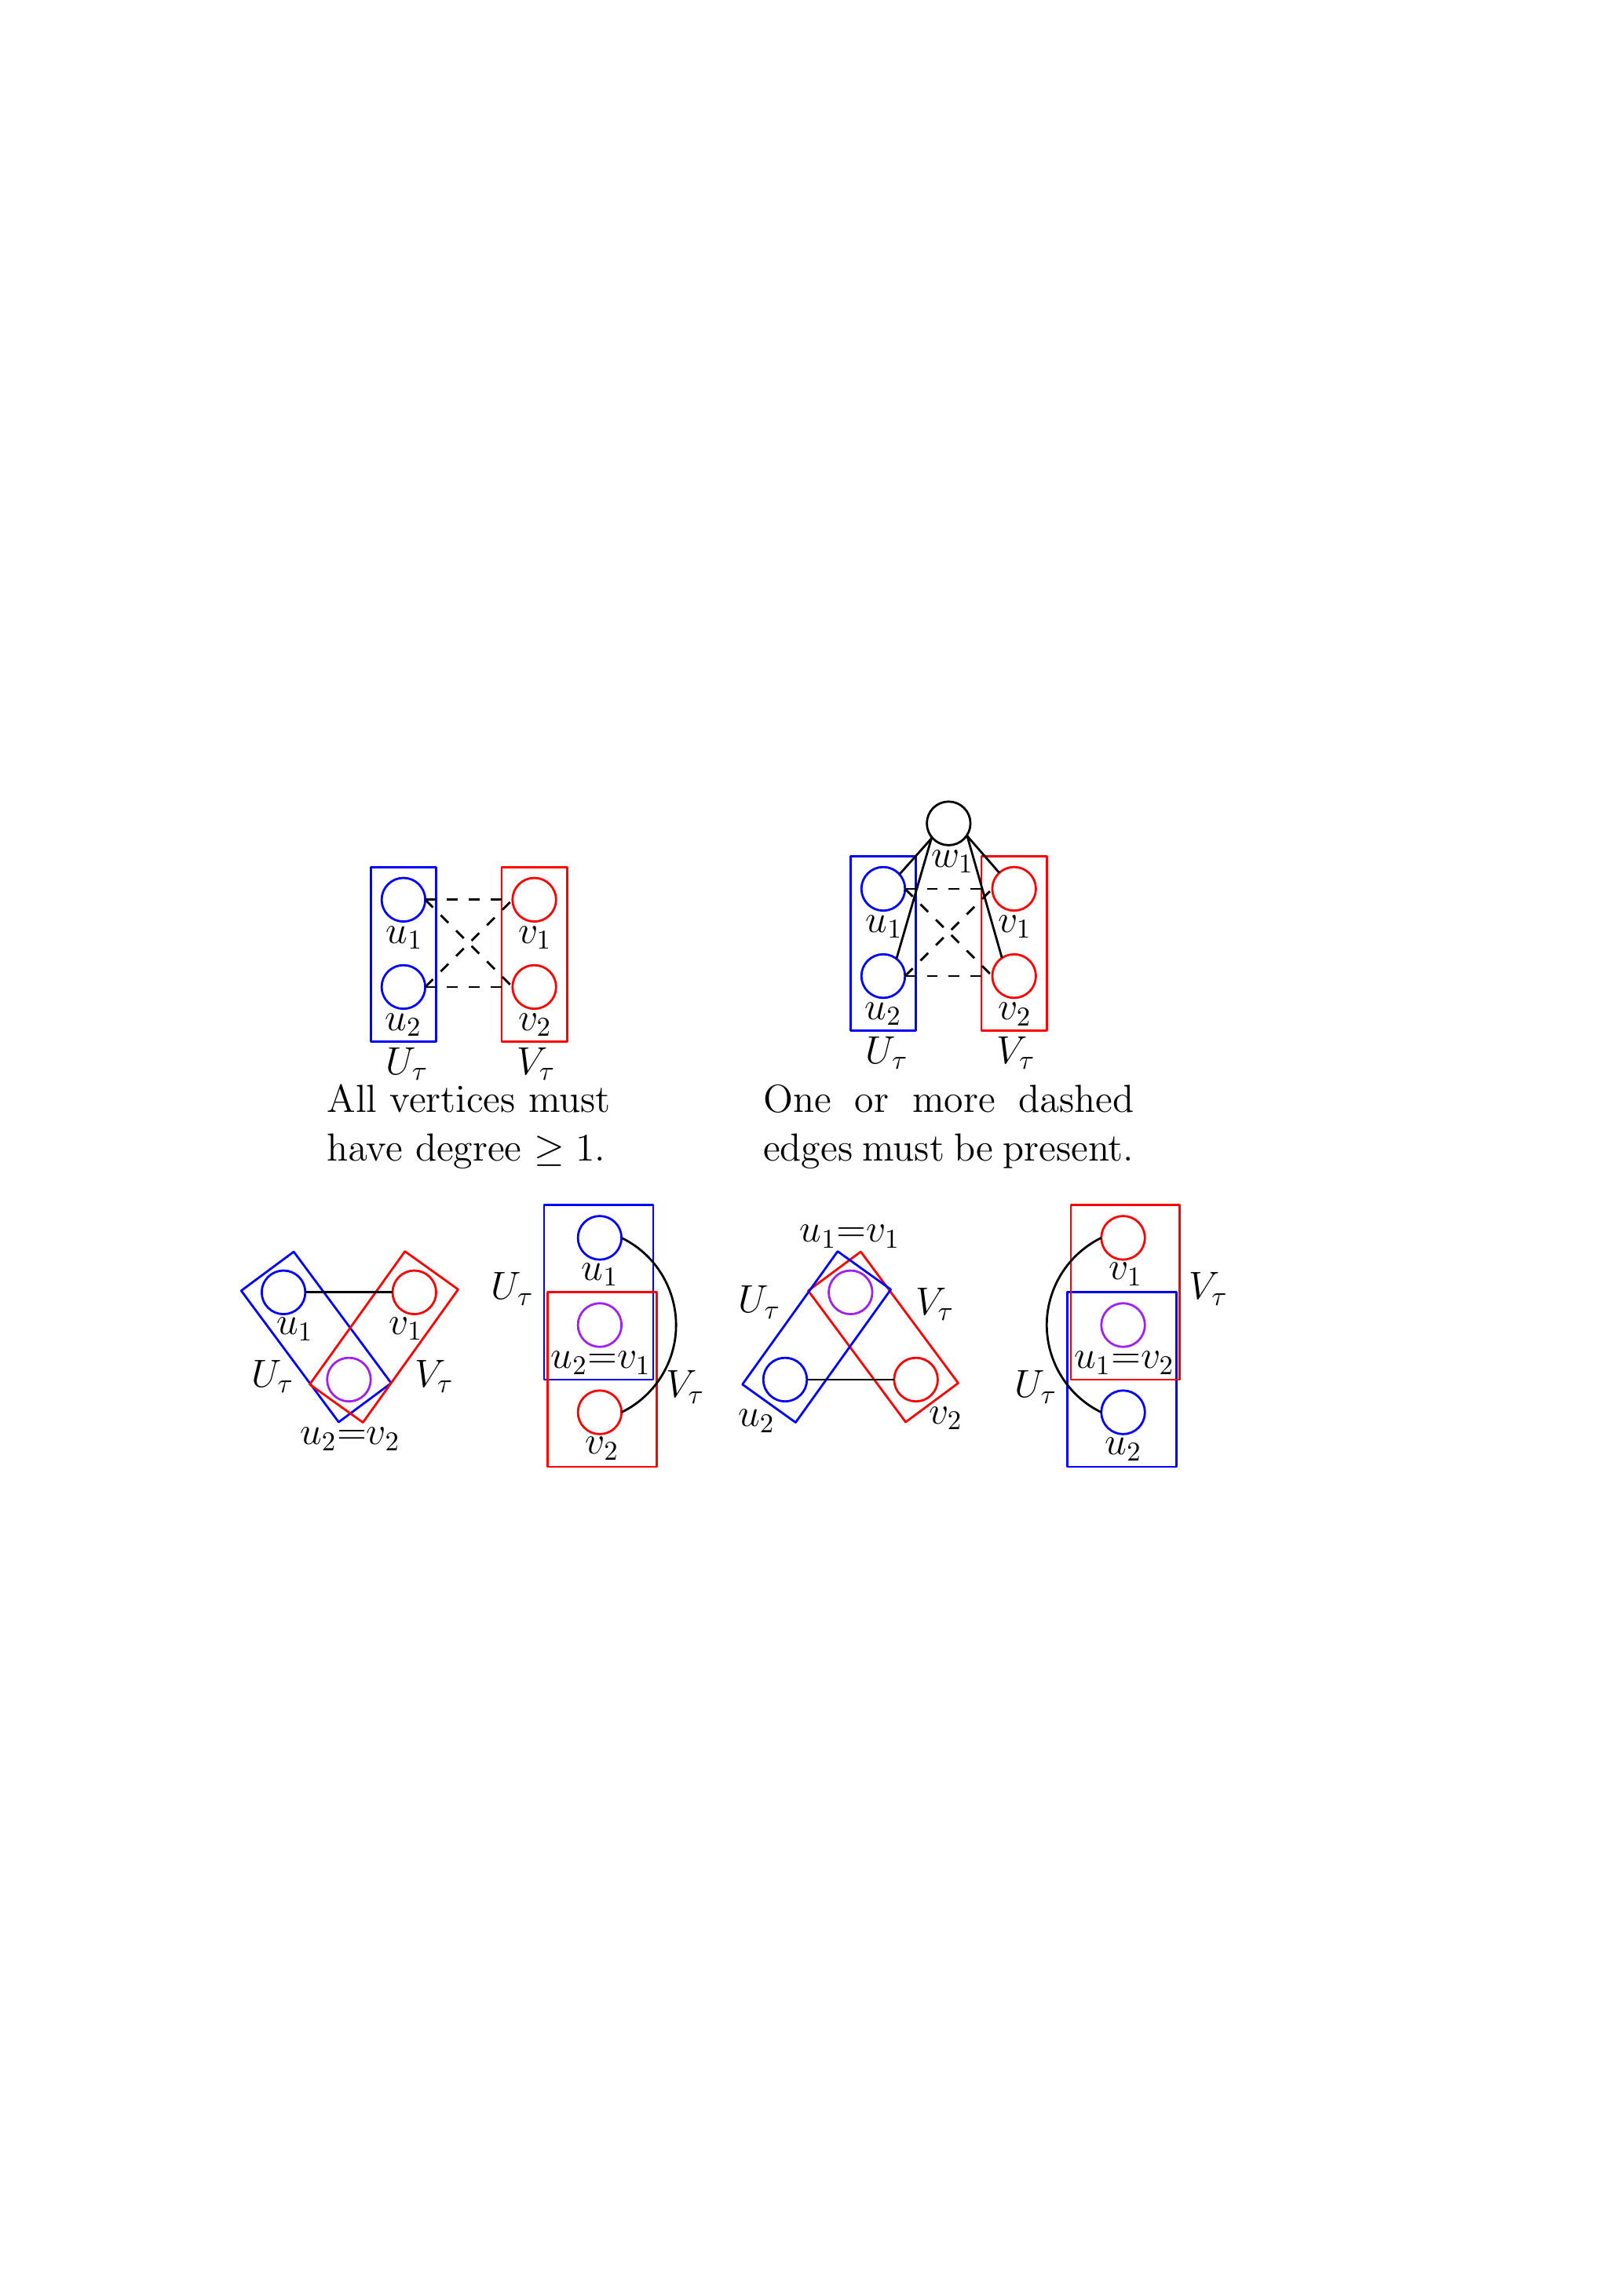}}
\caption{This figure shows the proper middle shapes $\tau$ where $|U_{tau}| = |V_{tau}| = 2$. In the upper row, we have $\tau_{Id:}$, $\tau_{E}$, and $\tau_{X,E}$. In the bottom row, we have  $\tau_{u_2 = v_2,e}$, $\tau_{u_2 = v_1,e}$, $\tau_{u_1 = v_1,e}$, and $\tau_{u_1 = v_2,e}$.}
\end{figure}
\begin{figure}[ht]\label{onevertexseparatortausfigure}
\centerline{\includegraphics[height=3cm]{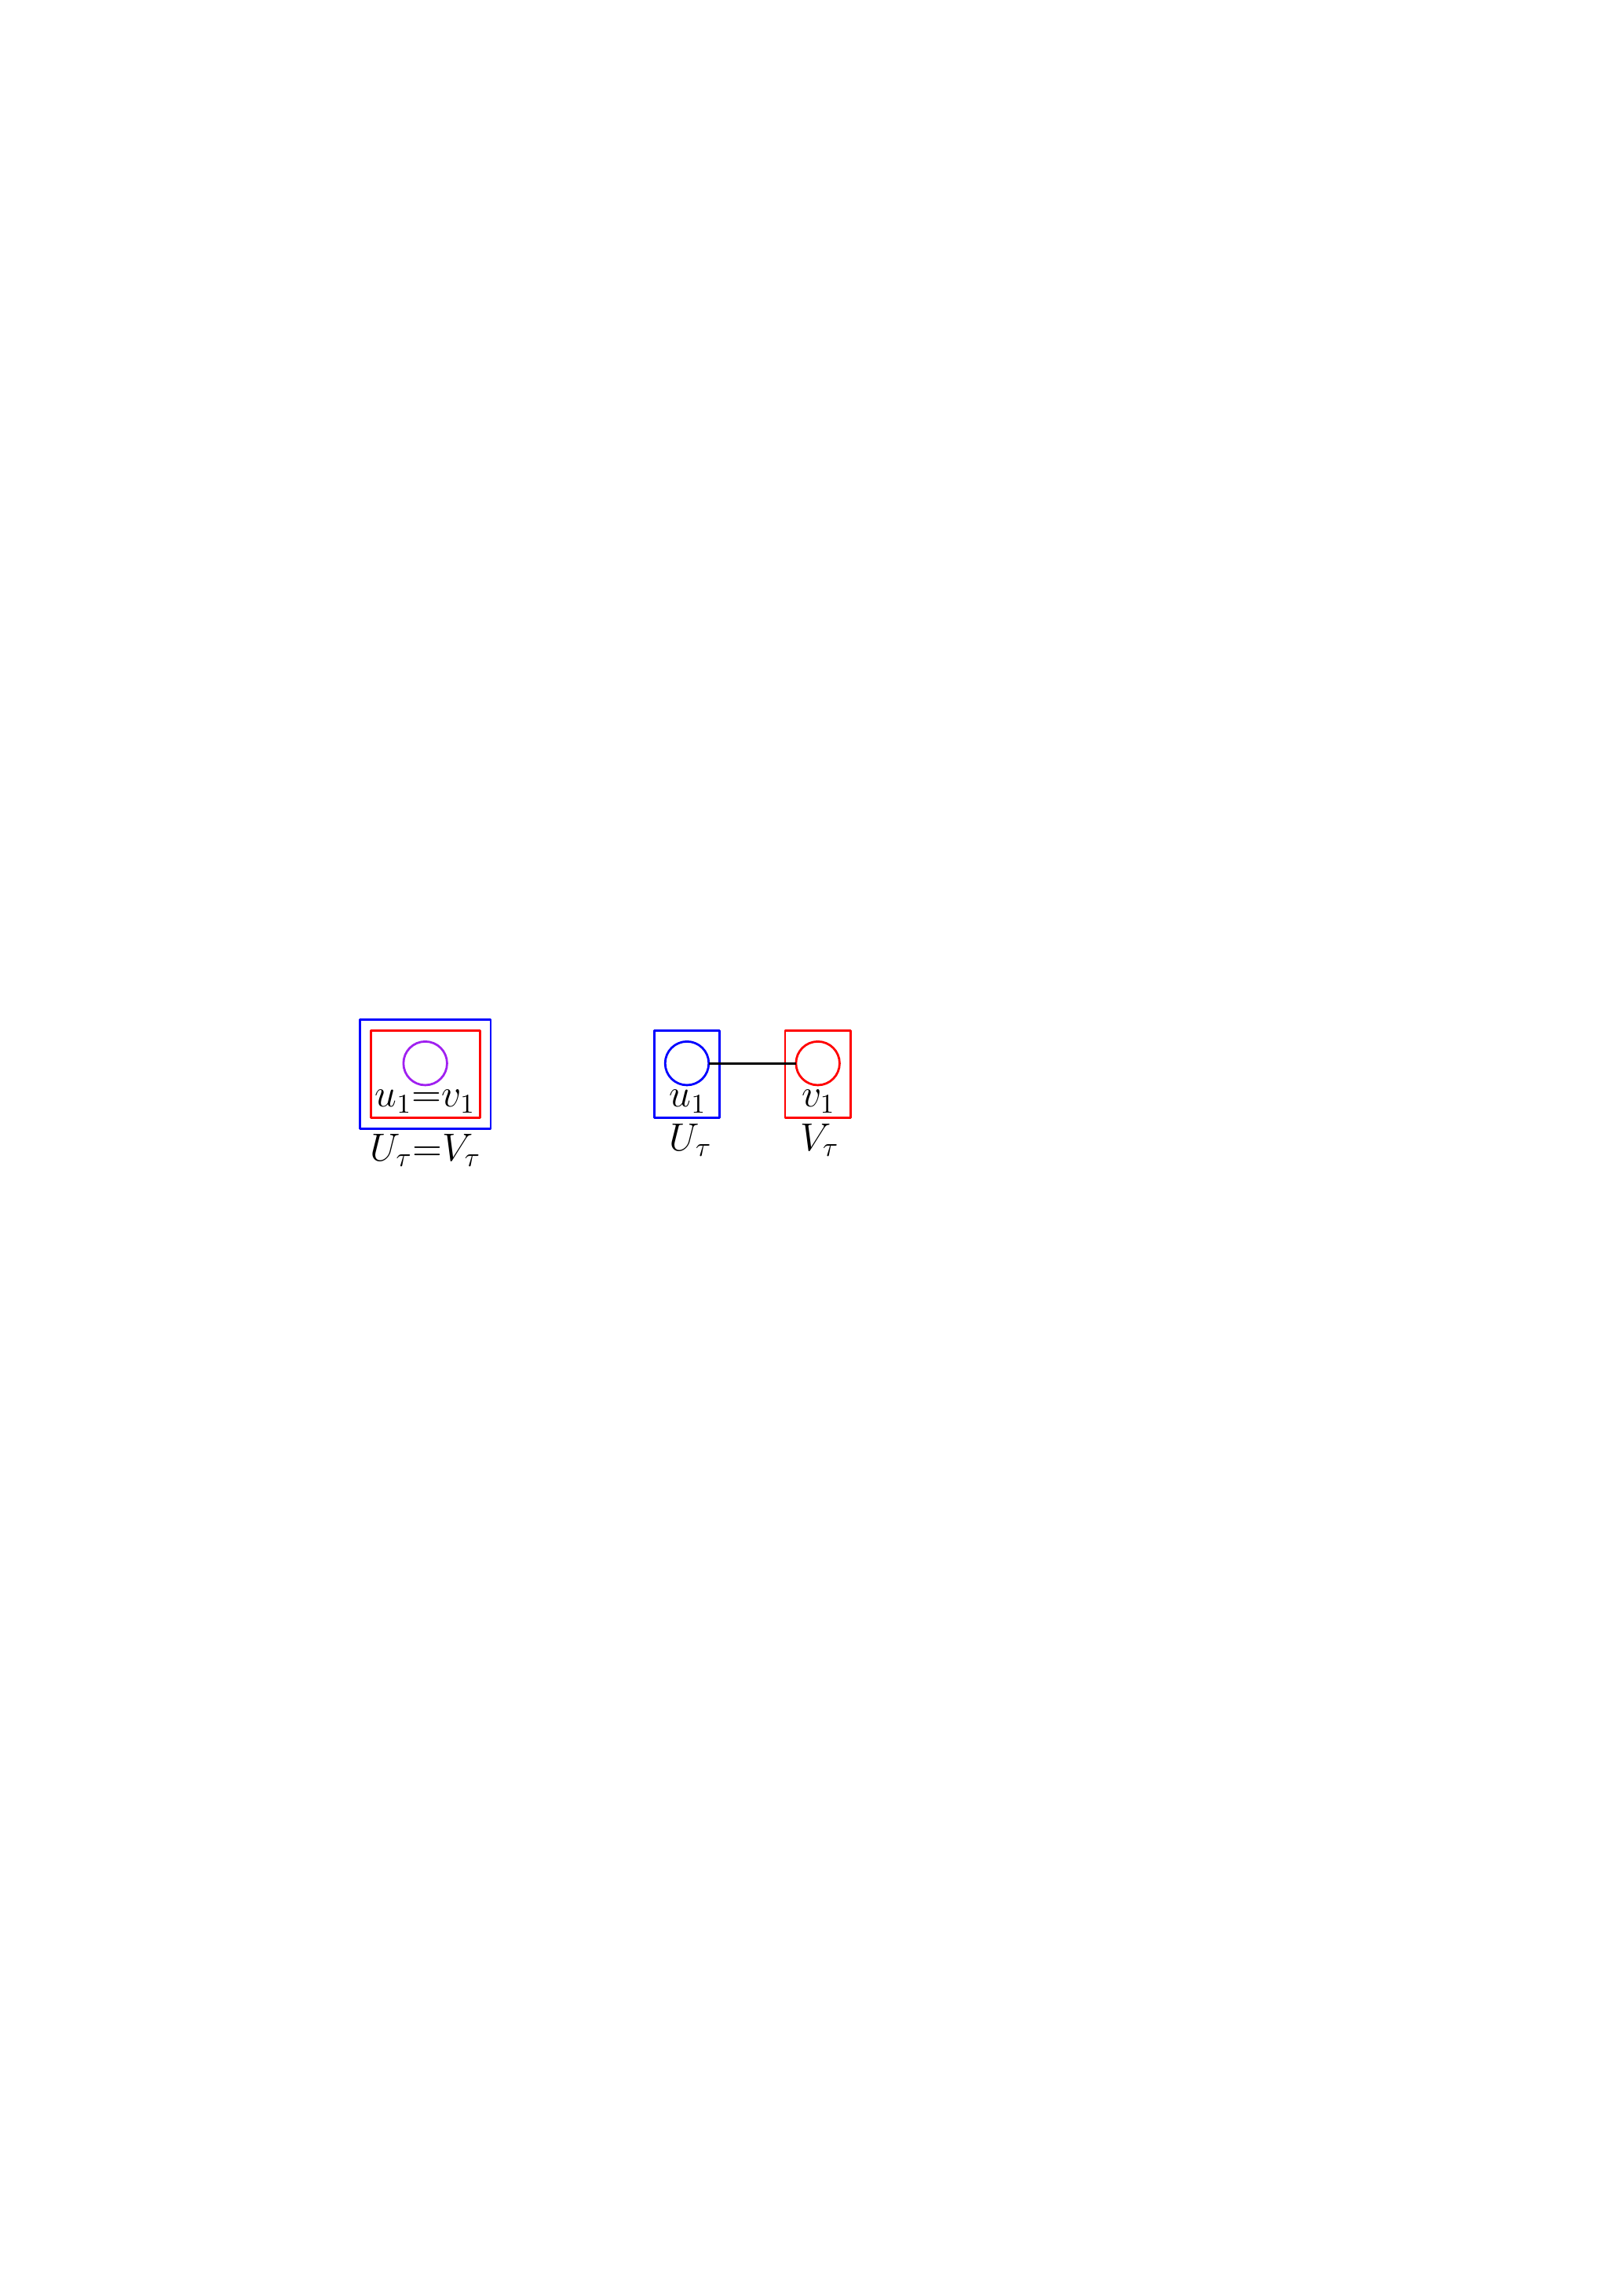}}
\caption{This figure shows the proper middle shapes $\tau$ where $|U_{tau}| = |V_{tau}| = 1$. On the left we have $\tau_{Id\cdot}$ and on the right we have $\tau_{e}$.}
\end{figure}

Some decompositions are as follows:
\begin{example} \ 
\begin{enumerate}
\item $\alpha_{X,\emptyset} = \sigma_7 \circ \tau_{Id\cdot} \circ \sigma_7^T$ (see Figure \ref{decompositiononefigure}).
\item $\alpha_{\{(u_1,v_1),(u_2,v_1)\}} = \sigma_7 \circ \tau_{Id\cdot} \circ \sigma_{u_1,u_2 \to u_1}^T$ (see Figure \ref{decompositiontwofigure}).
\item $\alpha_{\{(u_2,v_1)\}} = \sigma_{u_1,u_2 \to u_2} \circ \tau_{e} \circ \sigma_{u_1,u_2 \to u_1}^T$ (see Figure \ref{decompositionthreefigure}).
\item \begin{align*}
\alpha_{\{(u_1,v_1),(u_2,v_2)\}} &= \sigma_{Id:} \circ \alpha_{\{(u_1,v_1),(u_2,v_2)\}} \circ \sigma_{Id:}^T = \sigma_{Id:} \circ \alpha_{\{(u_1,v_2),(u_2,v_1)\}} \circ \sigma_{swap}^T \\
&= \sigma_{swap}^T \circ \alpha_{\{(u_1,v_2),(u_2,v_1)\}} \circ \sigma_{Id:} = \sigma_{swap} \circ \alpha_{\{(u_1,v_1),(u_2,v_2)\}} \circ \sigma_{swap}^T
\end{align*}
\end{enumerate}
\end{example}
\begin{remark}
Since there are $4$ different ways to decompose $\alpha_{\{(u_1,v_1),(u_2,v_2)\}}$, we split the coefficient $\lambda_{\alpha_{\{(u_1,v_1),(u_2,v_2)\}}}$ among these four decompositions. This is the reason for the factor of $4$ in the denominator in the entries of the matrix $H_{\tau}$.
\end{remark}
\begin{figure}[ht]\label{decompositiononefigure}
\centerline{\includegraphics[height=4cm]{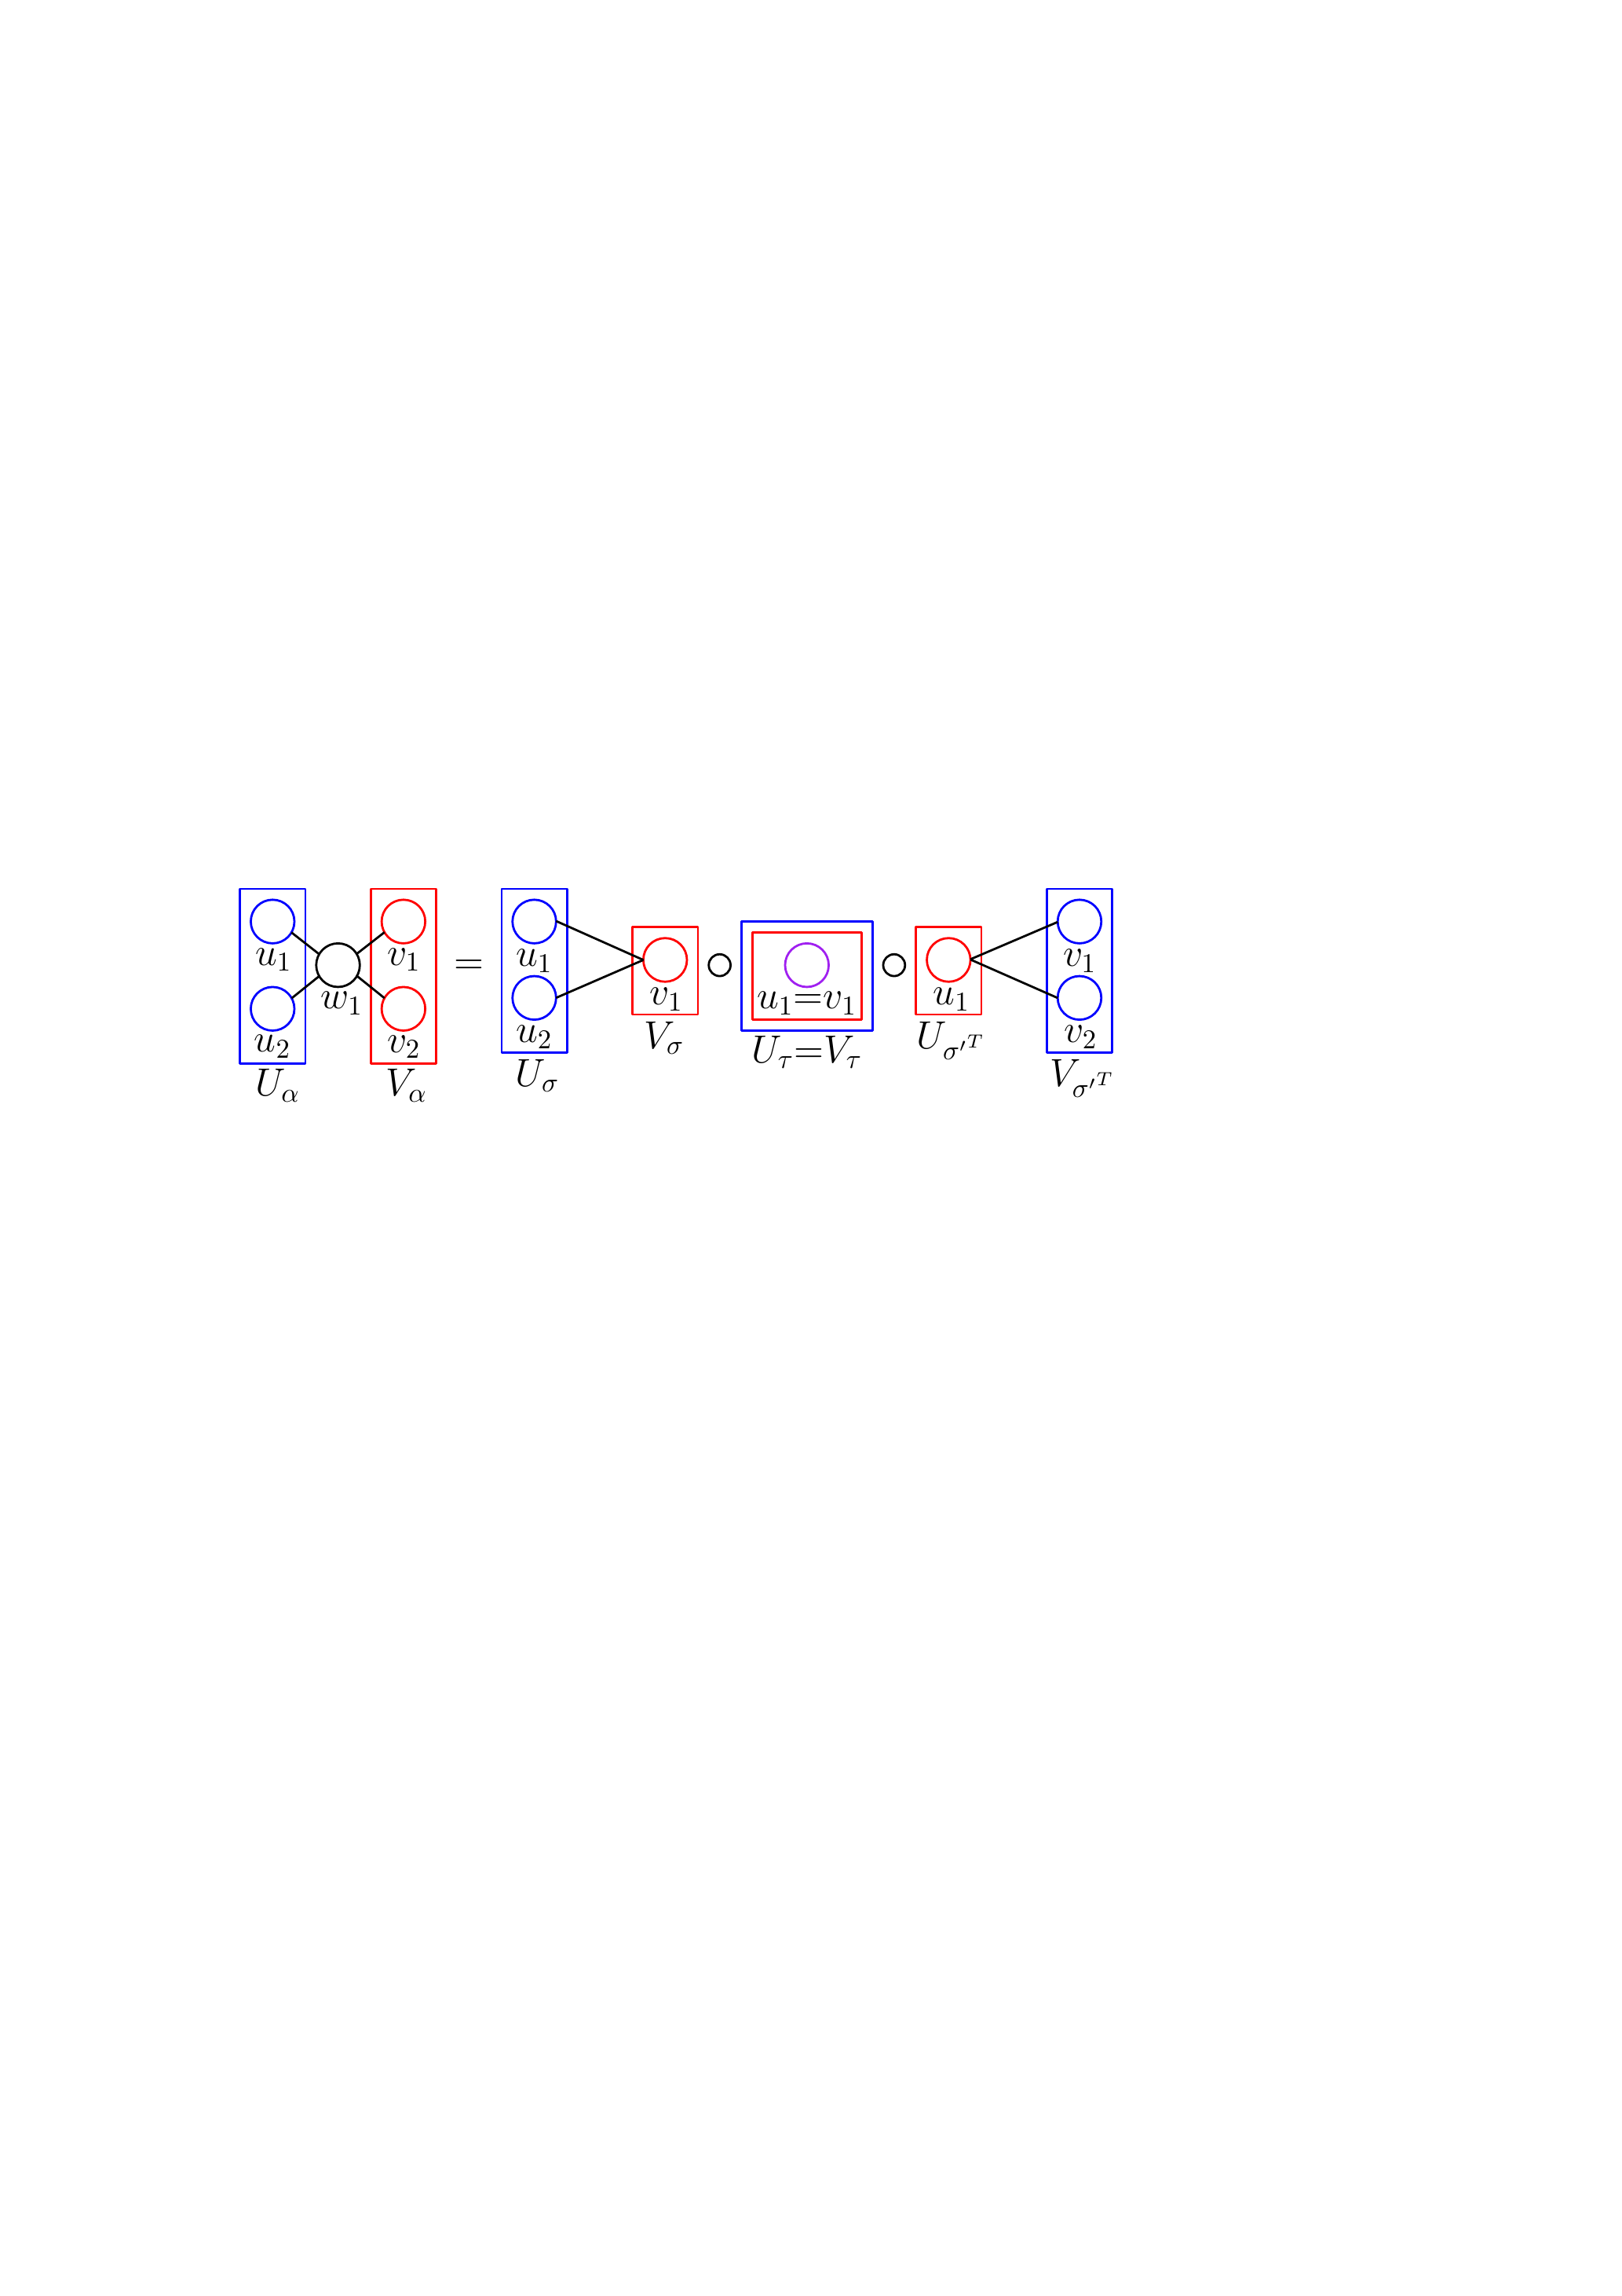}}
\caption{This figure shows the decomposition $\alpha_{X,\emptyset} = \sigma_7 \circ \tau_{Id\cdot} \circ \sigma_7^T$.}
\end{figure}
\begin{figure}[ht]\label{decompositiontwofigure}
\centerline{\includegraphics[height=4cm]{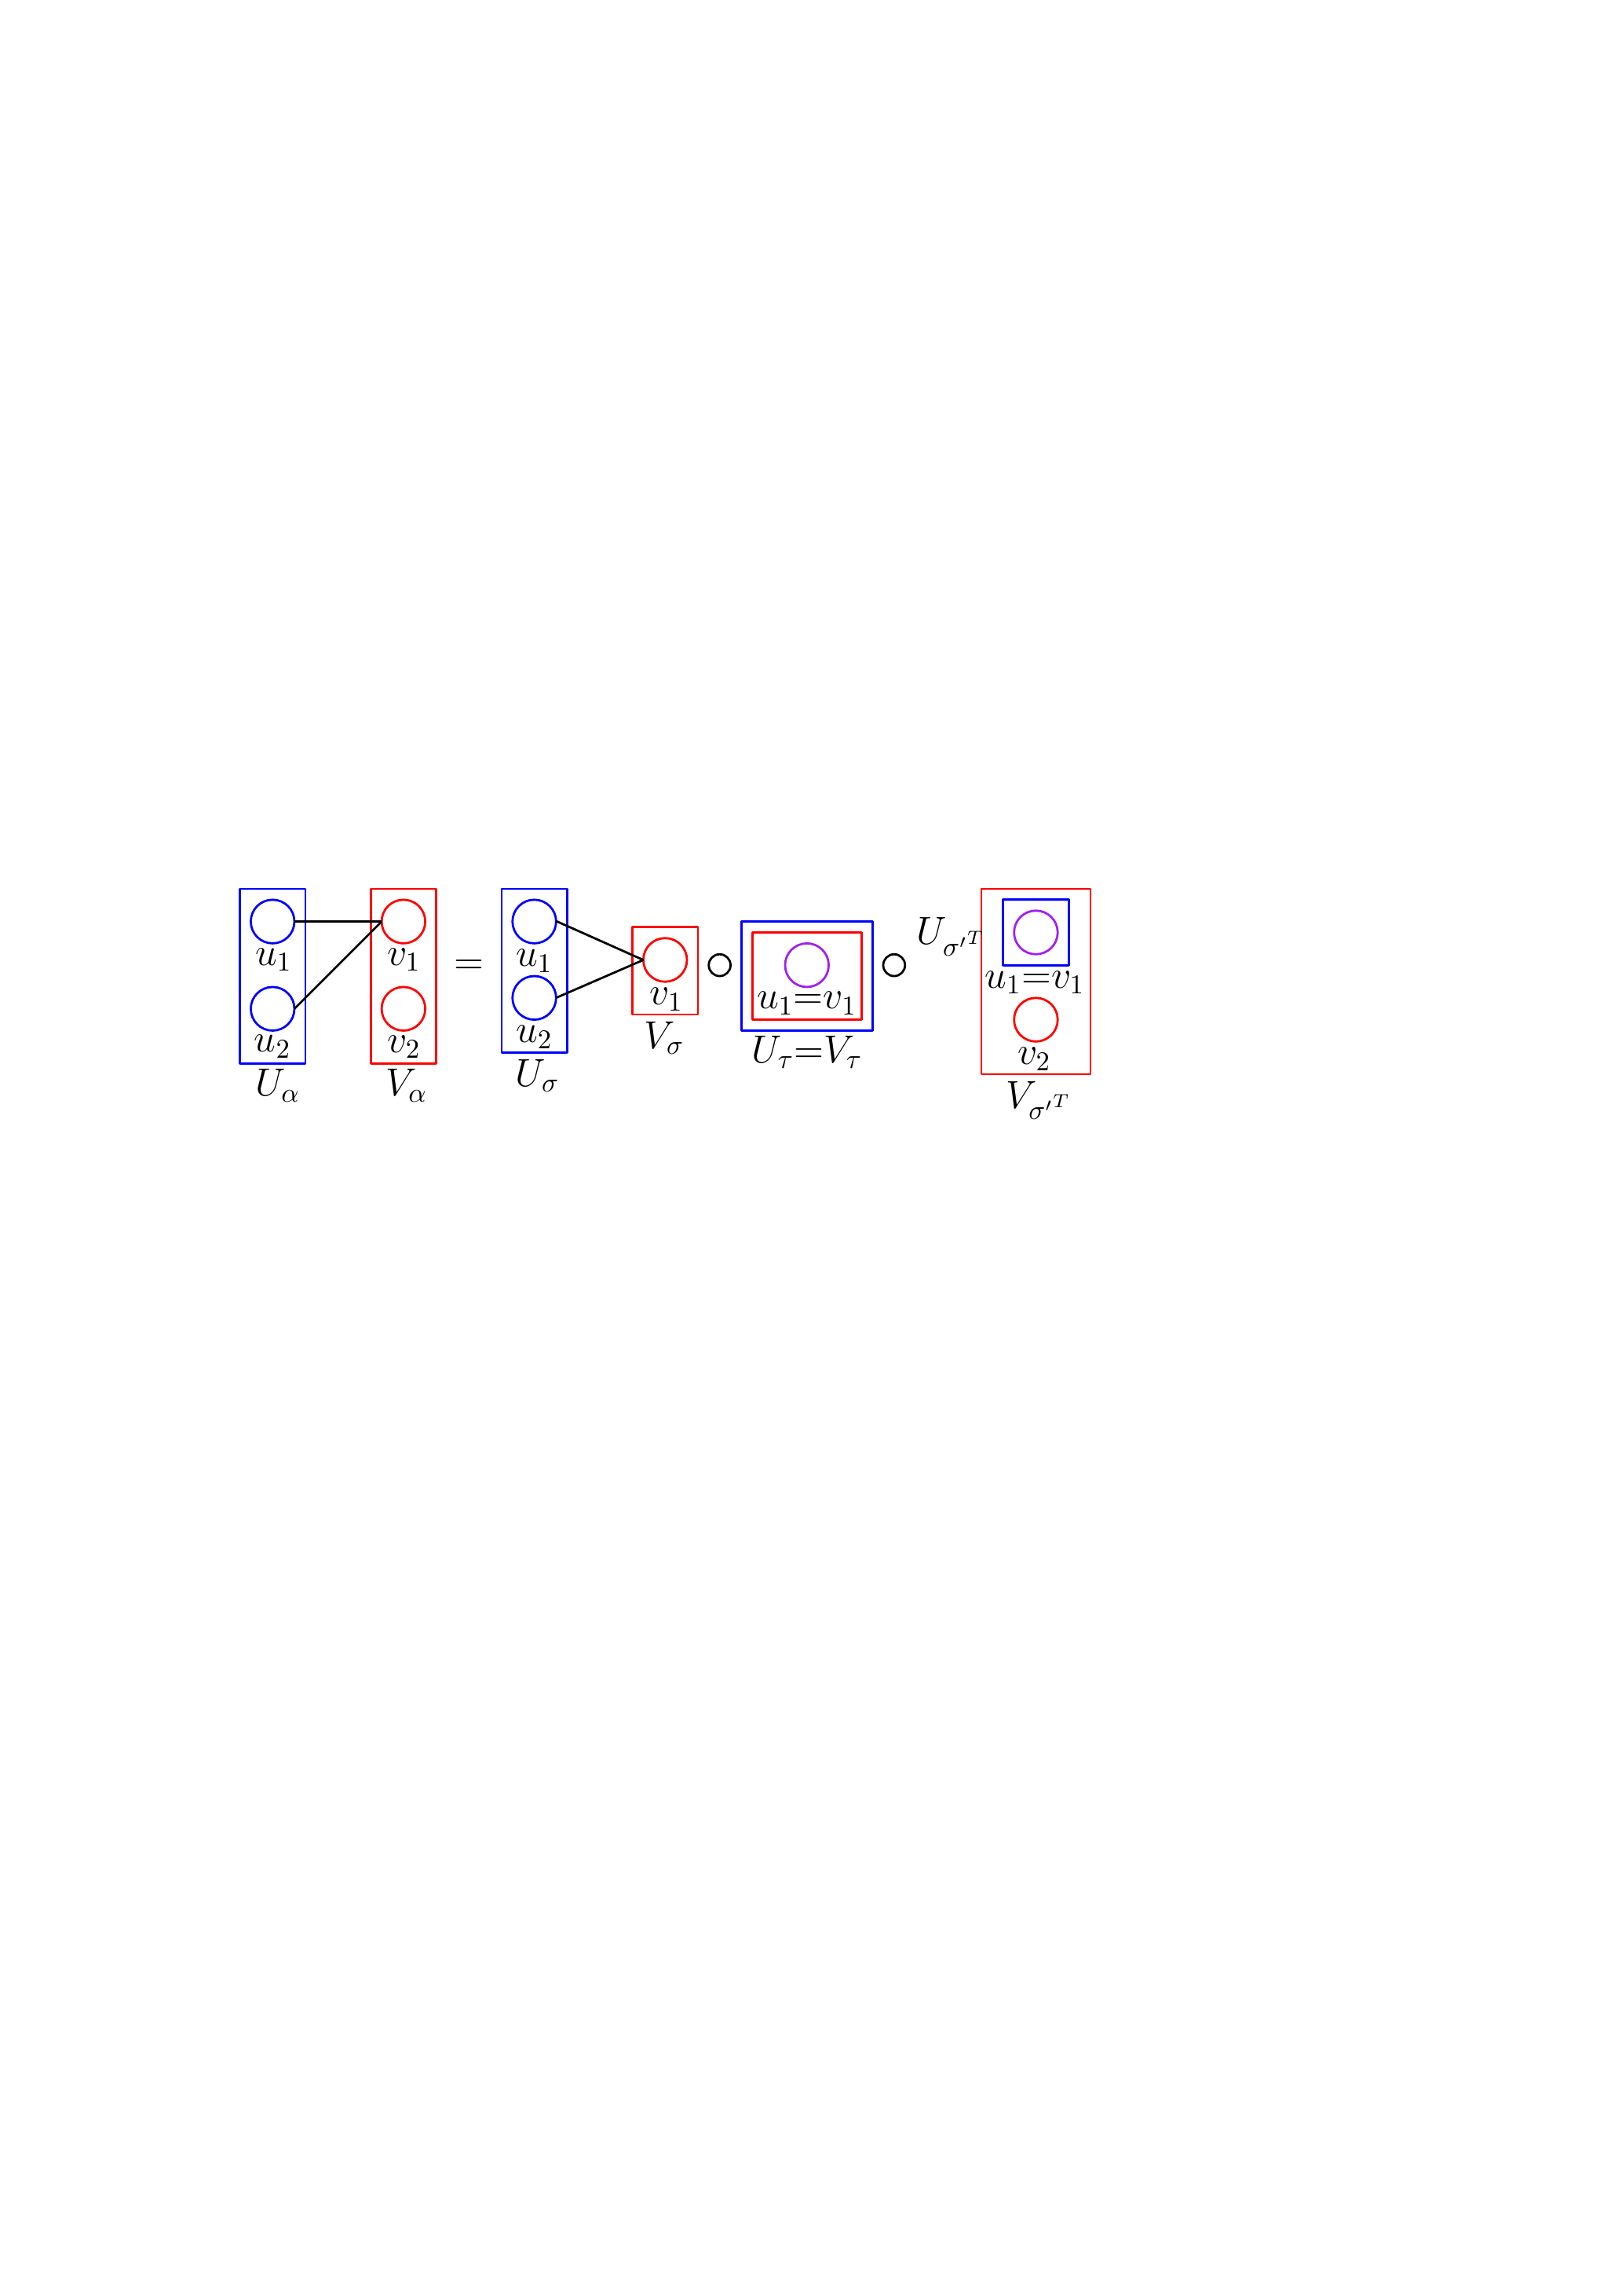}}
\caption{This figure shows the decomposition $\alpha_{\{(u_1,v_1),(u_2,v_1)\}} = \sigma_7 \circ \tau_{Id\cdot} \circ \sigma_{u_1,u_2 \to u_1}^T$.}
\end{figure}
\begin{figure}[ht]\label{decompositionthreefigure}
\centerline{\includegraphics[height=4cm]{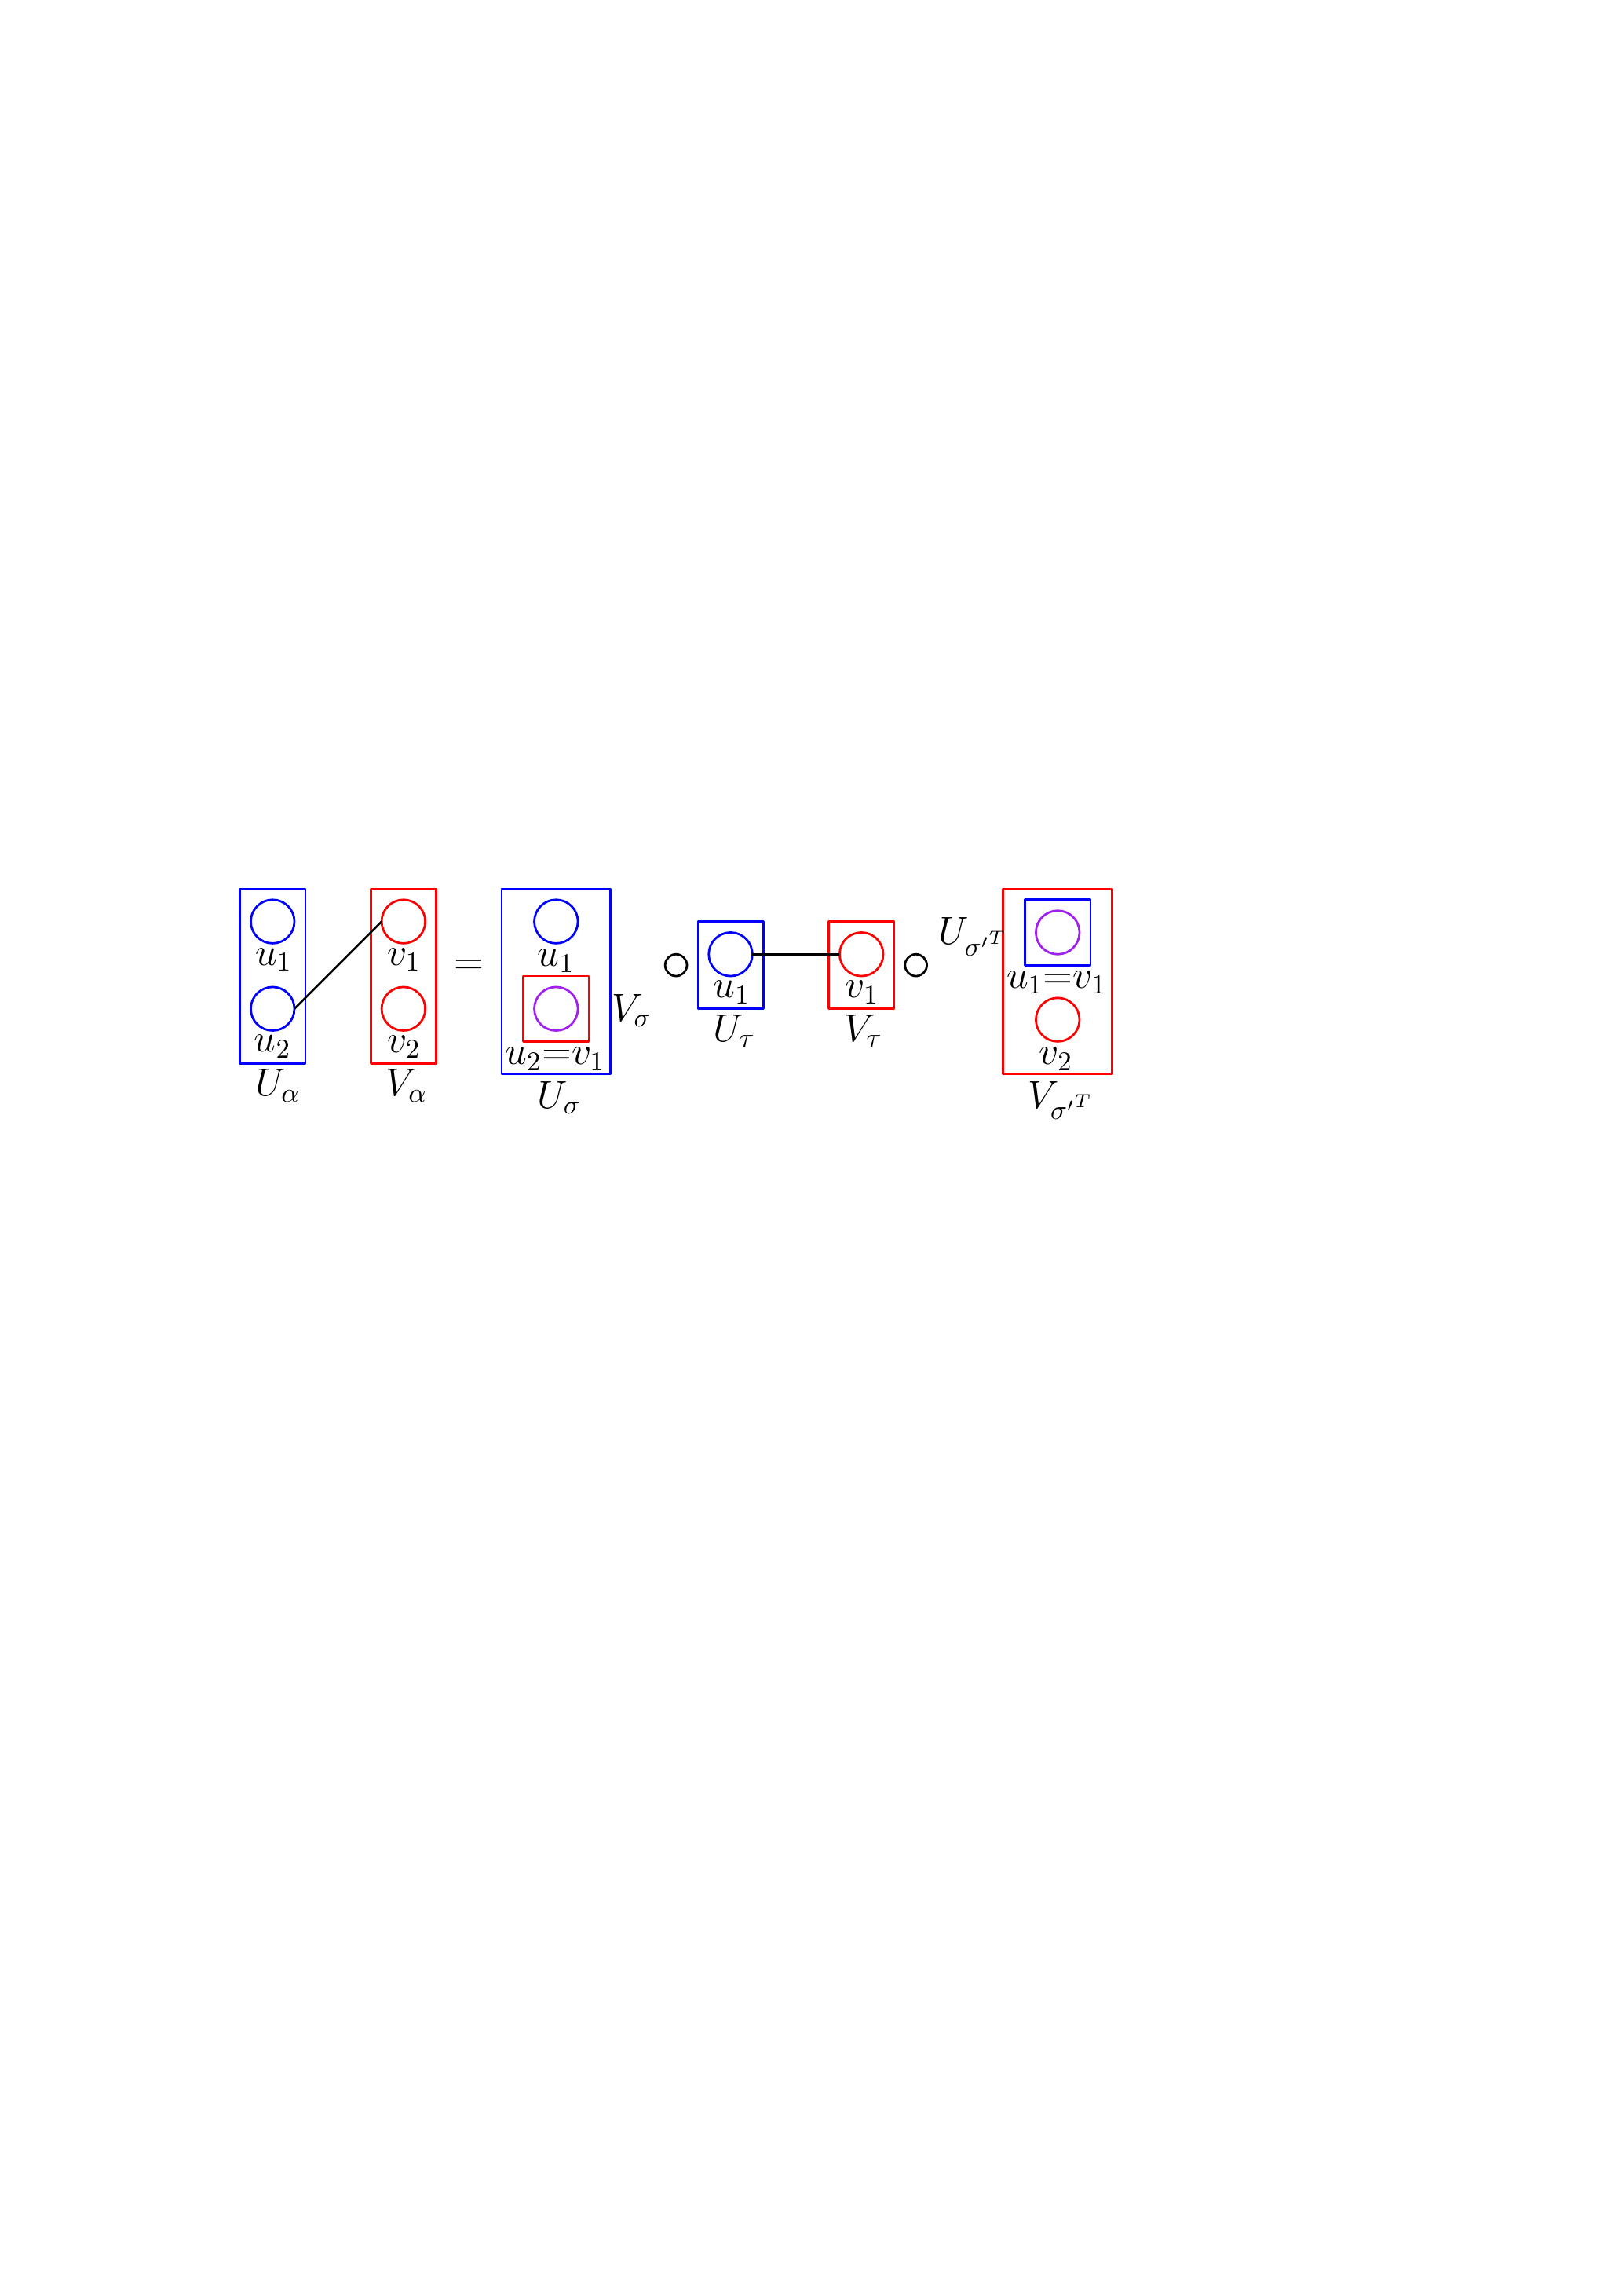}}
\caption{This figure shows the decomposition $\alpha_{\{(u_2,v_1)\}} = \sigma_{u_1,u_2 \to u_2} \circ \tau_{e} \circ \sigma_{u_1,u_2 \to u_1}^T$.}
\end{figure}

Our coefficient matrices are as follows (ignoring zero rows and columns):
\begin{enumerate}
\item $H_{Id_{(u_1,u_2)}}$ has two rows and columns indexed by $\sigma_{Id:}$ and $\sigma_{swap}$ and has entries $\left(\begin{matrix}
\frac{k^2}{2n^2} & \frac{k^2}{2n^2}\\
\frac{k^2}{2n^2} & \frac{k^2}{2n^2}\\
\end{matrix}\right)$.
\item $H_{Id_{(u_1)}}$ has rows and columns indexed by $\sigma_{u_1,u_2 \to u_1}$, $\sigma_{u_1,u_2 \to u_2}$, and $\sigma_7$ and has entries
\[
\left(\begin{matrix}
\frac{k^3}{n^3} & \frac{k^3}{n^3} & \frac{k^4}{n^4}\\
\frac{k^3}{n^3} & \frac{k^3}{n^3} & \frac{k^4}{n^4}\\
\frac{k^4}{n^4} & \frac{k^4}{n^4} & C\frac{k^5}{n^5}\\
\end{matrix}\right) \]
\item $H_{Id_{\emptyset}}$ has a single row and column indexed by $\sigma_{u_1,u_2 \to \emptyset}$ and has a single entry which is $\frac{k^4}{n^4}$.
\item For all $E \subseteq \{(u_1,v_1), (u_1,v_2), (u_2,v_1), (u_2,v_2)\}$ such that all four vertices $u_1,u_2,v_1,v_2$ are incident to at least one edge in $E$, $H_{\tau_{E}}$ has two rows and columns indexed by $\sigma_{Id:}$ and $\sigma_{swap}$ and has entries $\left(\begin{matrix}
\frac{k^4}{4n^4} & \frac{k^4}{4n^4}\\
\frac{k^4}{4n^4} & \frac{k^4}{4n^4}\\
\end{matrix}\right)$.
\item For all $E \subseteq \{(u_1,v_1), (u_1,v_2), (u_2,v_1), (u_2,v_2)\}$ such that $E \neq \emptyset$,  $H_{\tau_{X,E}}$ has two rows and columns indexed by $\sigma_{Id:}$ and $\sigma_{swap}$ and has entries $\left(\begin{matrix}
\frac{k^5}{4n^5} & \frac{k^5}{4n^5}\\
\frac{k^5}{4n^5} & \frac{k^5}{4n^5}\\
\end{matrix}\right)$.
\item For all $i,j \in \{1,2\}$, $H_{\tau_{u_i = v_j,e}}$ has two rows and columns indexed by $\sigma_{Id:}$ and $\sigma_{swap}$ and has entries $\left(\begin{matrix}
\frac{k^3}{4n^3} & \frac{k^3}{4n^3}\\
\frac{k^3}{4n^3} & \frac{k^3}{4n^3}\\
\end{matrix}\right)$.
\item $H_{\tau_{e}}$ has rows and columns indexed by $\sigma_{u_1,u_2 \to u_1}$ and $\sigma_{u_1,u_2 \to u_2}$ and has entries 
\[
\left(\begin{matrix}
\frac{k^4}{n^4} & \frac{k^4}{n^4}\\
\frac{k^4}{n^4} & \frac{k^4}{n^4}\\
\end{matrix}\right)\]
\end{enumerate}
\subsection{Verifying the first and second conditions of the machinery}
We can verify the fist and second conditions of the machinery as follows.
\begin{enumerate}
\item $H_{Id_{(u_1,u_2)}} \succeq 0$ and $H_{Id_{\emptyset}} \succeq 0$
\item As long as $C \geq 1$, $H_{Id_{(u_1)}} \succeq 0$. This condition is the reason why we need to add this term in.
\item For all $E \subseteq \{(u_1,v_1), (u_1,v_2), (u_2,v_1), (u_2,v_2)\}$ such that all four vertices $u_1,u_2,v_1,v_2$ are incident to at least one edge in $E$, $||M_{\tau_{E}}||$ is $\tilde{O}(n)$ so $||M_{\tau_{E}}||H_{\tau_{E}} \preceq H_{Id_{(u_1,u_2)}}$ as long as $k << \sqrt{n}$.
\item For all $E \subseteq \{(u_1,v_1), (u_1,v_2), (u_2,v_1), (u_2,v_2)\}$ such that $E \neq \emptyset$, 
$||M_{\tau_{X,E}}||$ is $\tilde{O}(n^{3/2})$ so $||M_{\tau_{X,E}}||H_{\tau_{X,E}} \preceq H_{Id_{(u_1,u_2)}}$ as long as $k << \sqrt{n}$.
\item For all $i,j \in \{1,2\}$, $||M_{\tau_{u_i = v_j,e}}||$ is $\tilde{O}(\sqrt{n})$ so $||M_{\tau_{u_i = v_j,e}}||H_{\tau_{u_i = v_j,e}} \preceq H_{Id_{(u_1,u_2)}}$ as long as $k << \sqrt{n}$.
\item Since $\left(\begin{matrix}
\frac{k^3}{n^3} & \frac{k^3}{n^3} & \frac{k^4}{n^4}\\
\frac{k^3}{n^3} & \frac{k^3}{n^3} & \frac{k^4}{n^4}\\
\frac{k^4}{n^4} & \frac{k^4}{n^4} & C\frac{k^5}{n^5}\\
\end{matrix}\right) \succeq (1 - \frac{1}{C})\left(\begin{matrix}
\frac{k^3}{n^3} & \frac{k^3}{n^3} & 0\\
\frac{k^3}{n^3} & \frac{k^3}{n^3} & 0\\
0 & 0 & 0\\
\end{matrix}\right)$ and $||M_{\tau_{e}}||$ is $\tilde{O}(\sqrt{n})$, $||M_{\tau_{e}}||H_{\tau_{e}} \preceq H_{Id_{(u_1)}}$ as long as $C > 1$ and $k << \sqrt{n}$. Note that for pseudo-calibration we take $C = 1$. We can do this because we have more terms which allows us to have a more delicate factorization.
\end{enumerate}
\subsection{Verifying the third condition of the machinery}
The following left shapes $\gamma$ appear.
\begin{definition} \ 
\begin{enumerate}
\item Define $\gamma_7 = \sigma_7$.
\item Define $\gamma_{u_1,u_2 \to u_1} = \sigma_{u_1,u_2 \to u_1}$.
\item Define $\gamma_{u_1,u_2 \to u_2} = \sigma_{u_1,u_2 \to u_2}$.
\item Define $\gamma_{u_1,u_2 \to \emptyset} = \sigma_{u_1,u_2 \to \emptyset}$.
\item Define $\gamma_{u_1 \to \emptyset}$ to be the shape with $U_{\gamma_{u_1 \to \emptyset}} = (u_1)$ and $V_{\gamma_{u_1 \to \emptyset}} = \emptyset$
\end{enumerate}
\end{definition}
For illustrations of these gammas, see Figure \ref{possiblegammasfigure}. \\
\begin{figure}[ht]\label{possiblegammasfigure}
\centerline{\includegraphics[height=4cm]{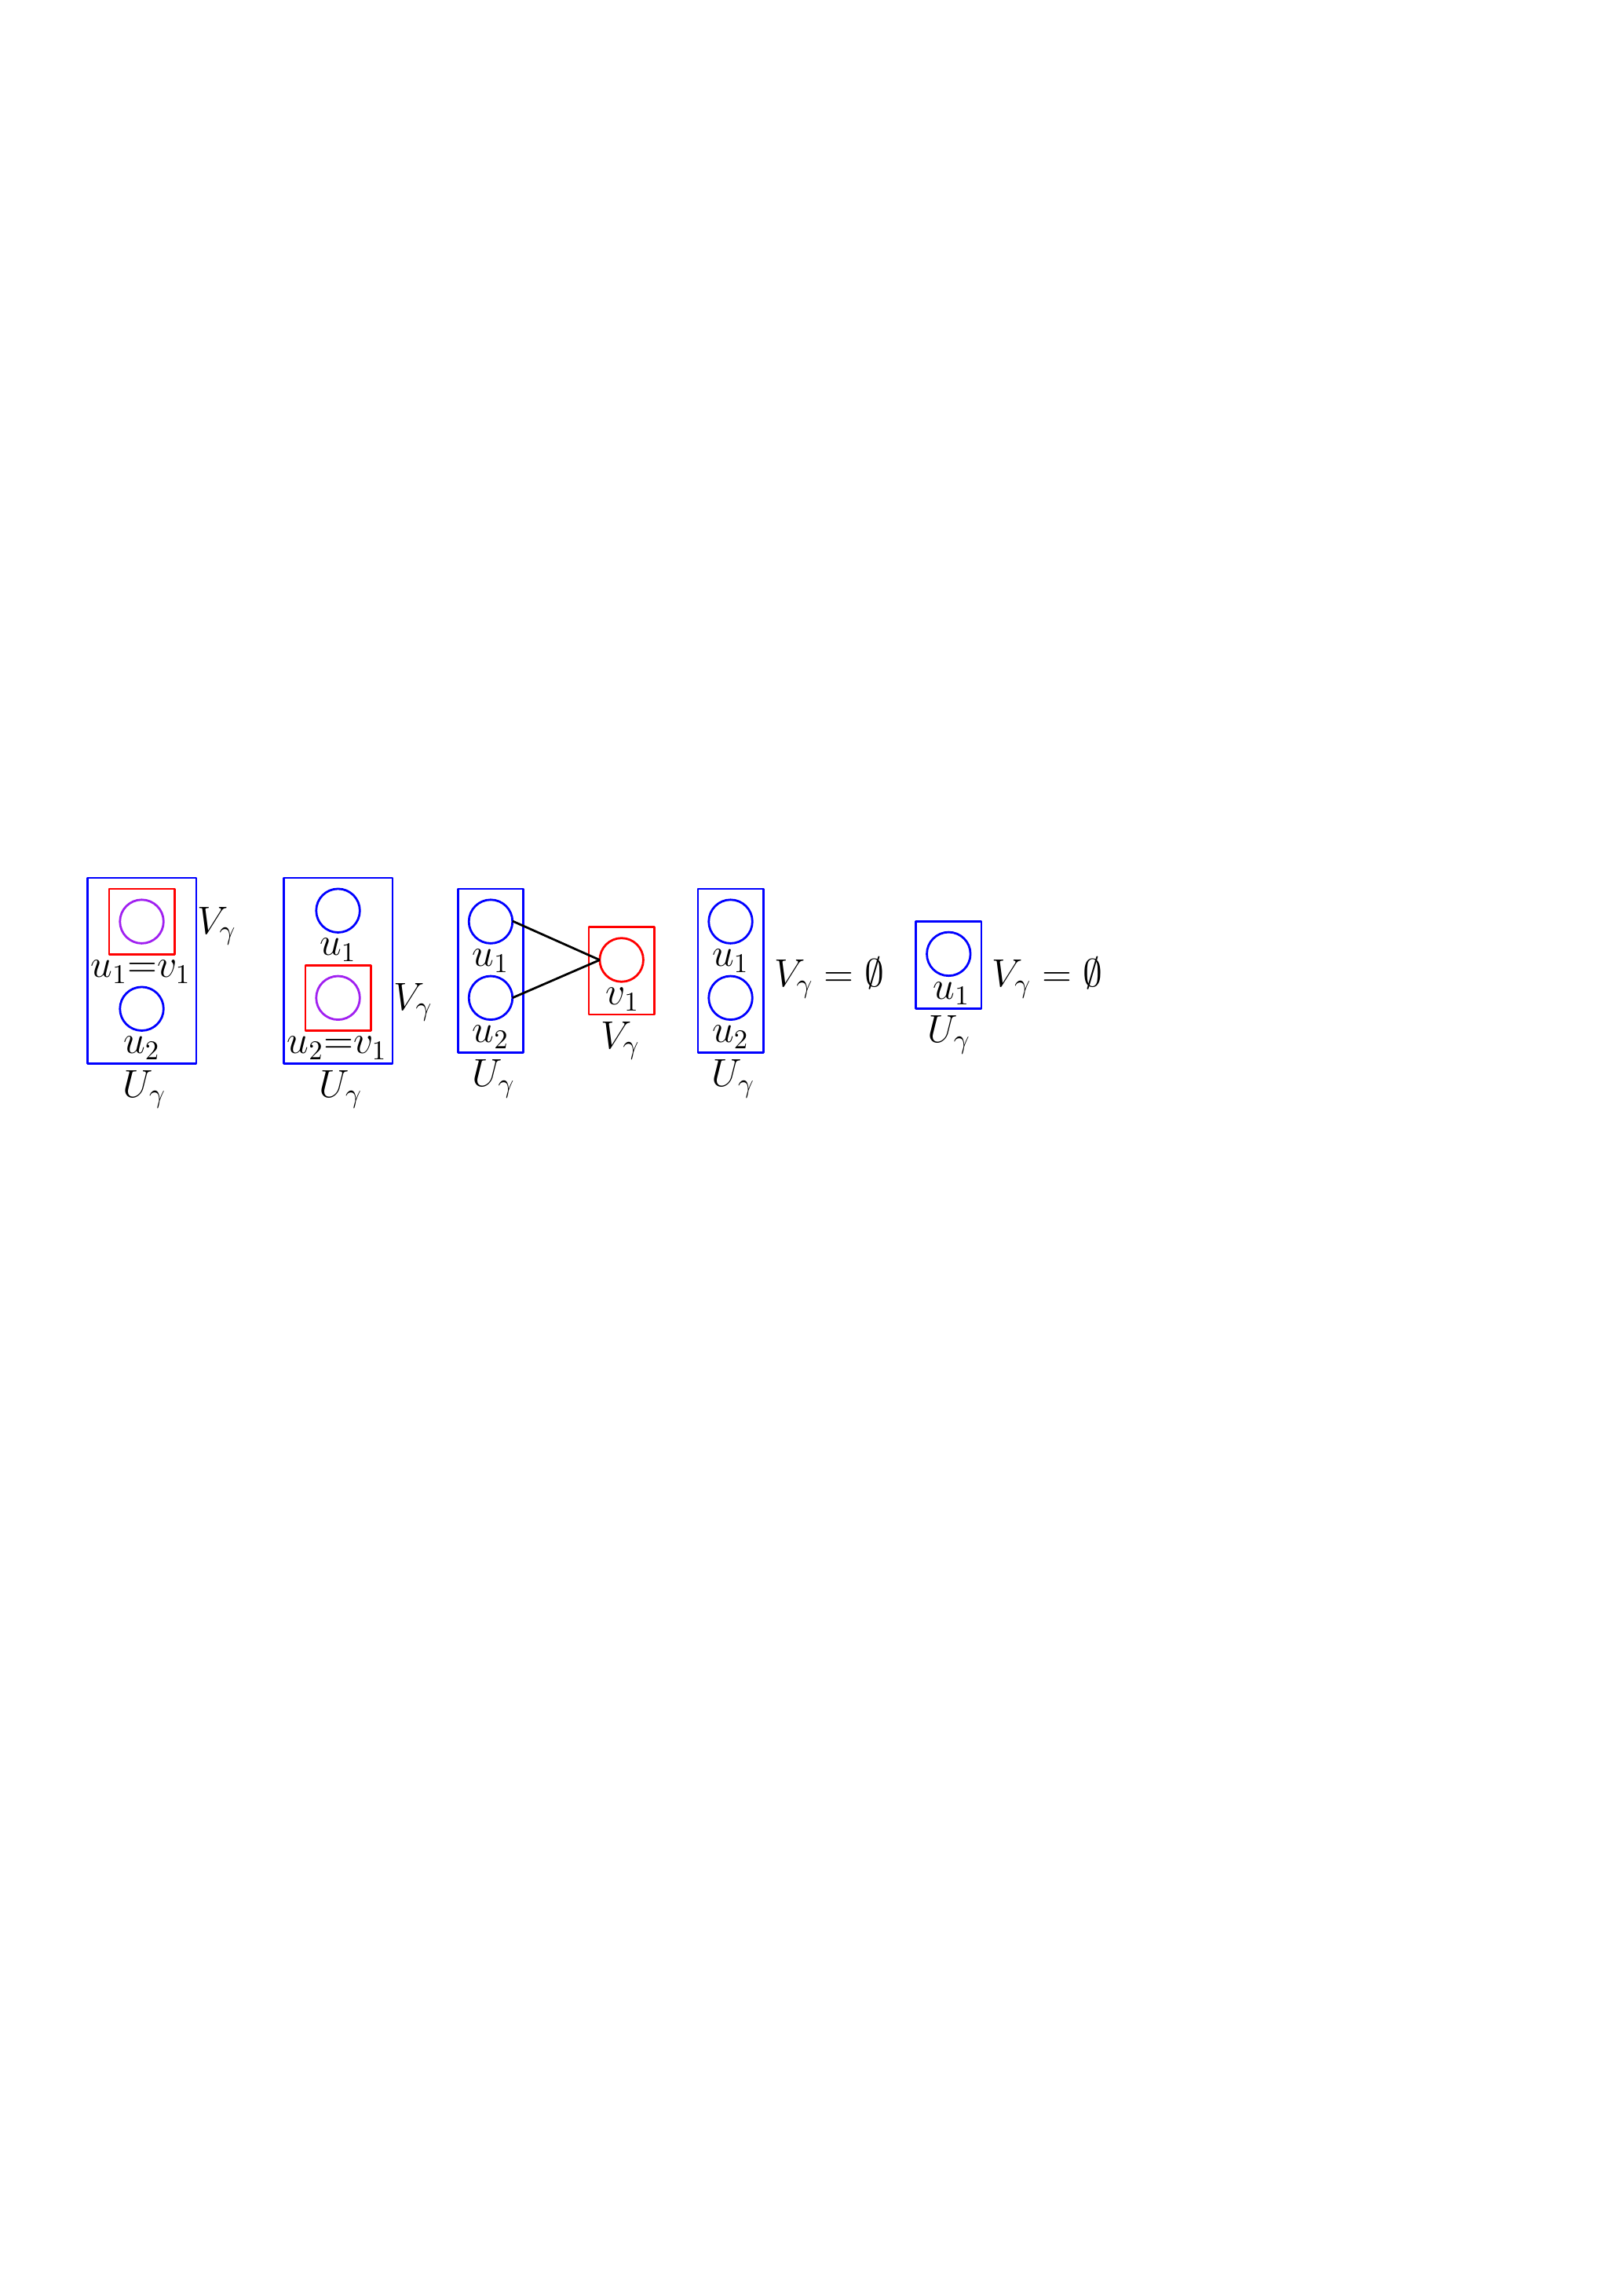}}
\caption{This figure shows the left shapes $\gamma$ which appear in the analysis. From left to right we have $\gamma_{u_1,u_2 \to u_1}$, $\gamma_{u_1,u_2 \to u_2}$, $\gamma_7$, $\gamma_{u_1,u_2 \to \emptyset}$, and $\gamma_{u_1 \to \emptyset}$}
\end{figure}
We have the following compositions.
\begin{enumerate}
\item $\sigma_{Id:} \circ \gamma_7 = \sigma_{swap} \circ \gamma_7 = \sigma_7$ (see Figure \ref{compositiononefigure}).
\item $\sigma_{Id:} \circ \gamma_{u_1,u_2 \to u_1} = \sigma_{u_1,u_2 \to u_1}$ and $\sigma_{swap} \circ \gamma_{u_1,u_2 \to u_1} = \sigma_{u_1,u_2 \to u_2}$ (see Figure \ref{compositiontwofigure}).
\item Similarly, $\sigma_{Id:} \circ \gamma_{u_1,u_2 \to u_2} = \sigma_{u_1,u_2 \to u_2}$ and $\sigma_{swap} \circ \gamma_{u_1,u_2 \to u_2} = \sigma_{u_1,u_2 \to u_1}$.
\item $\sigma_{Id:} \circ \gamma_{u_1,u_2 \to \emptyset} = \sigma_{swap} \circ \gamma_{u_1,u_2 \to \emptyset} = \sigma_{u_1,u_2 \to \emptyset}$.
\item $\sigma_{u_1,u_2 \to u_1} \circ \gamma_{u_1 \to \emptyset} = \sigma_{u_1,u_2 \to u_2} \circ \gamma_{u_1 \to \emptyset} = \sigma_{u_1,u_2 \to \emptyset}$ (see Figure \ref{compositionthreefigure}).
\end{enumerate}
\begin{figure}[ht]\label{compositiononefigure}
\centerline{\includegraphics[height=4cm]{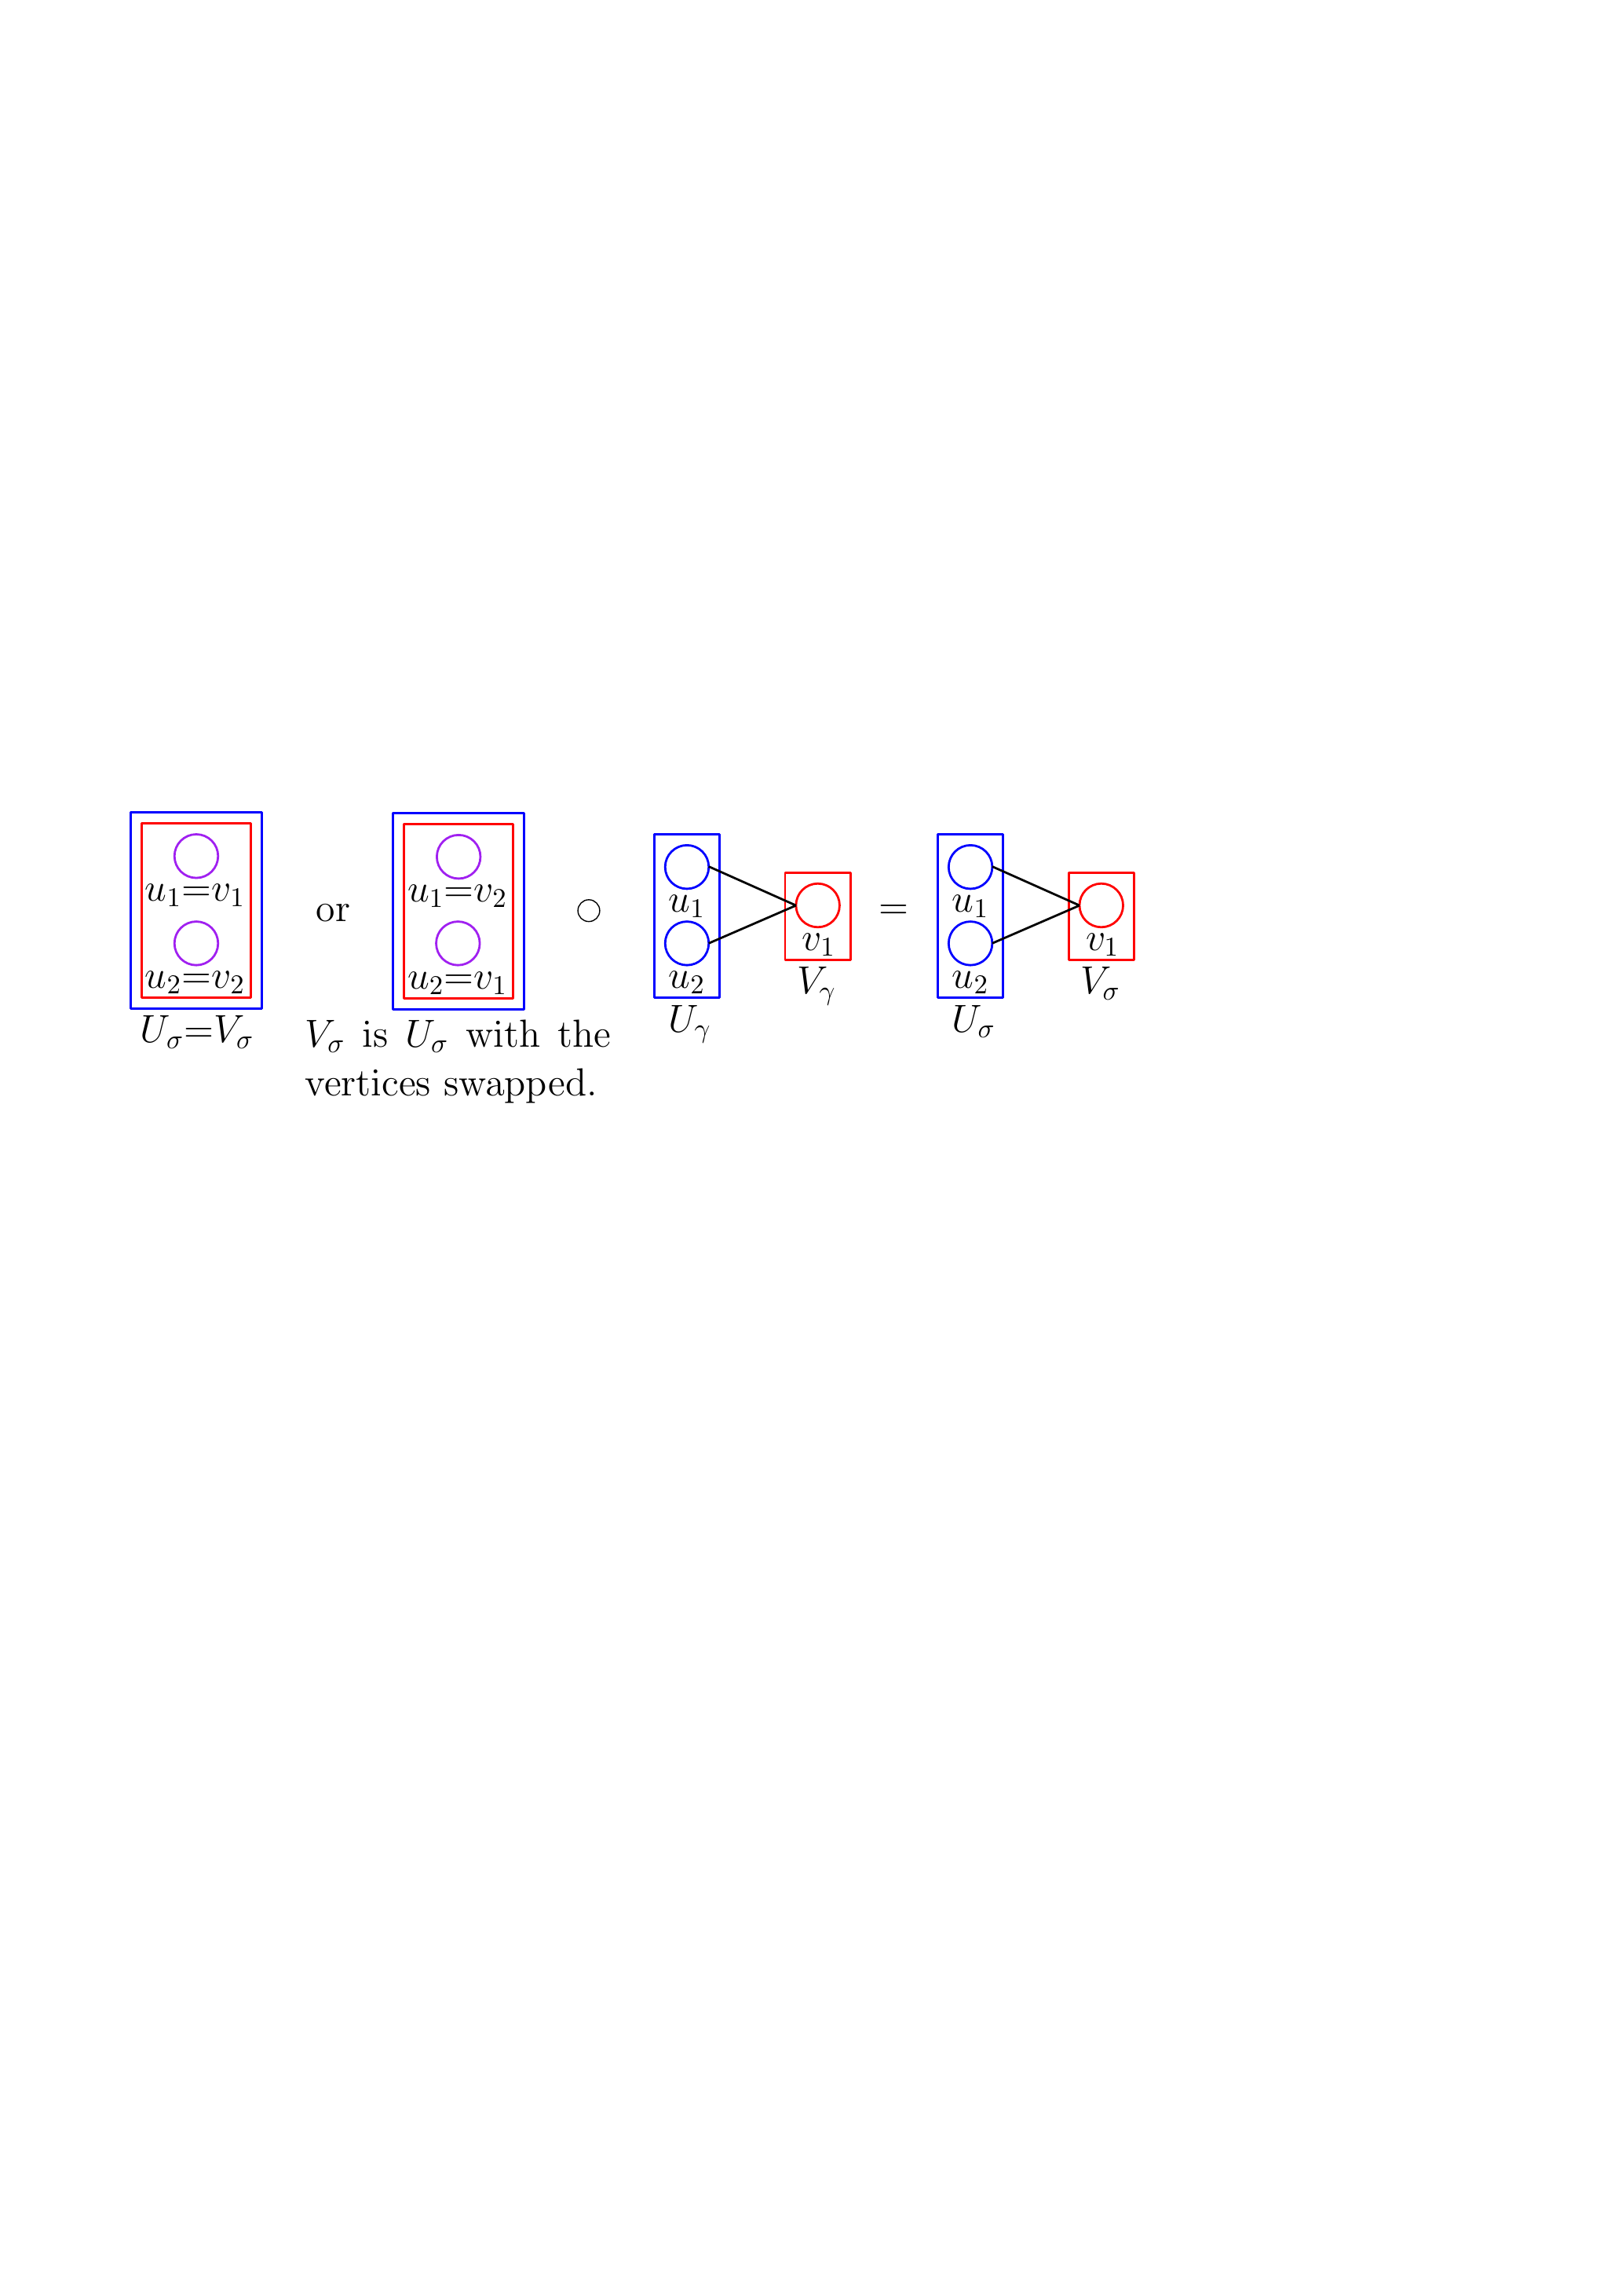}}
\caption{This figure shows the compositions $\sigma_{Id:} \circ \gamma_{7} = \sigma_{7}$ and $\sigma_{swap} \circ \gamma_{7} = \sigma_{7}$.}
\end{figure}
\begin{figure}[ht]\label{compositiontwofigure}
\centerline{\includegraphics[height=8cm]{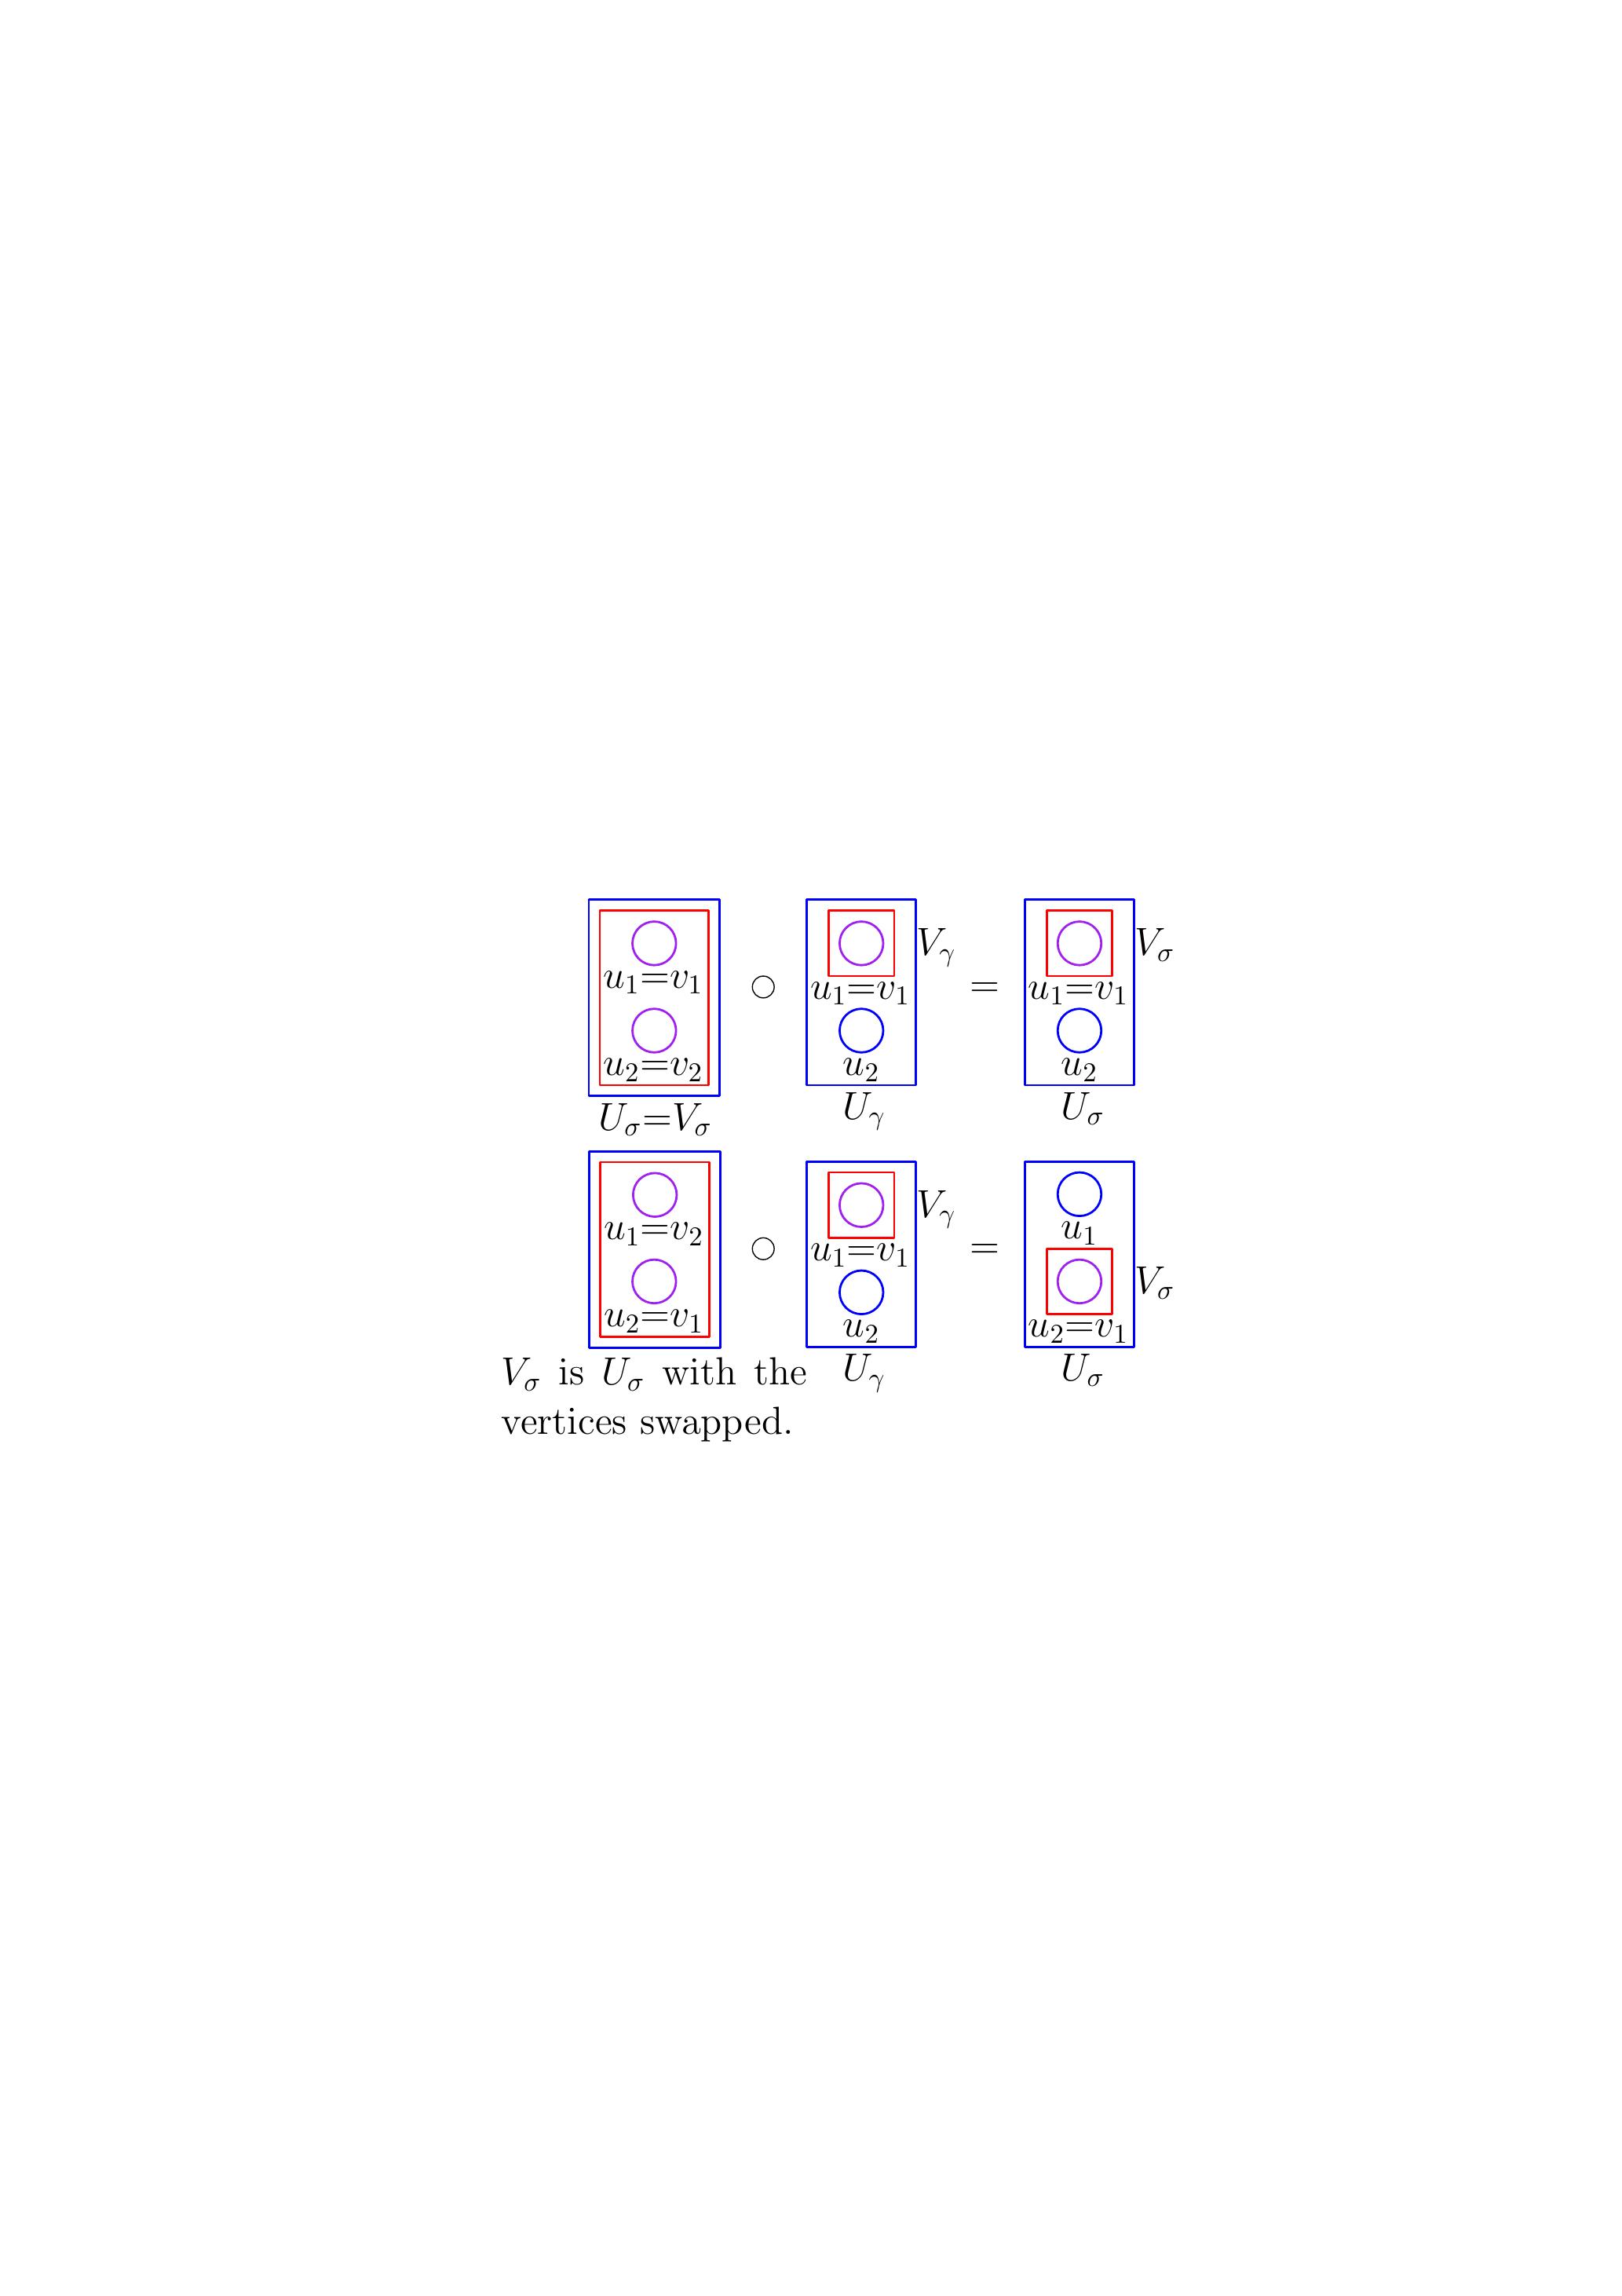}}
\caption{This figure shows the compositions $\sigma_{Id:} \circ \gamma_{u_1,u_2 \to u_1} = \sigma_{u_1,u_2 \to u_1}$ and $\sigma_{swap} \circ \gamma_{u_1,u_2 \to u_1} = \sigma_{u_1,u_2 \to u_2}$ .}
\end{figure}
\begin{figure}[ht]\label{compositionthreefigure}
\centerline{\includegraphics[height=4cm]{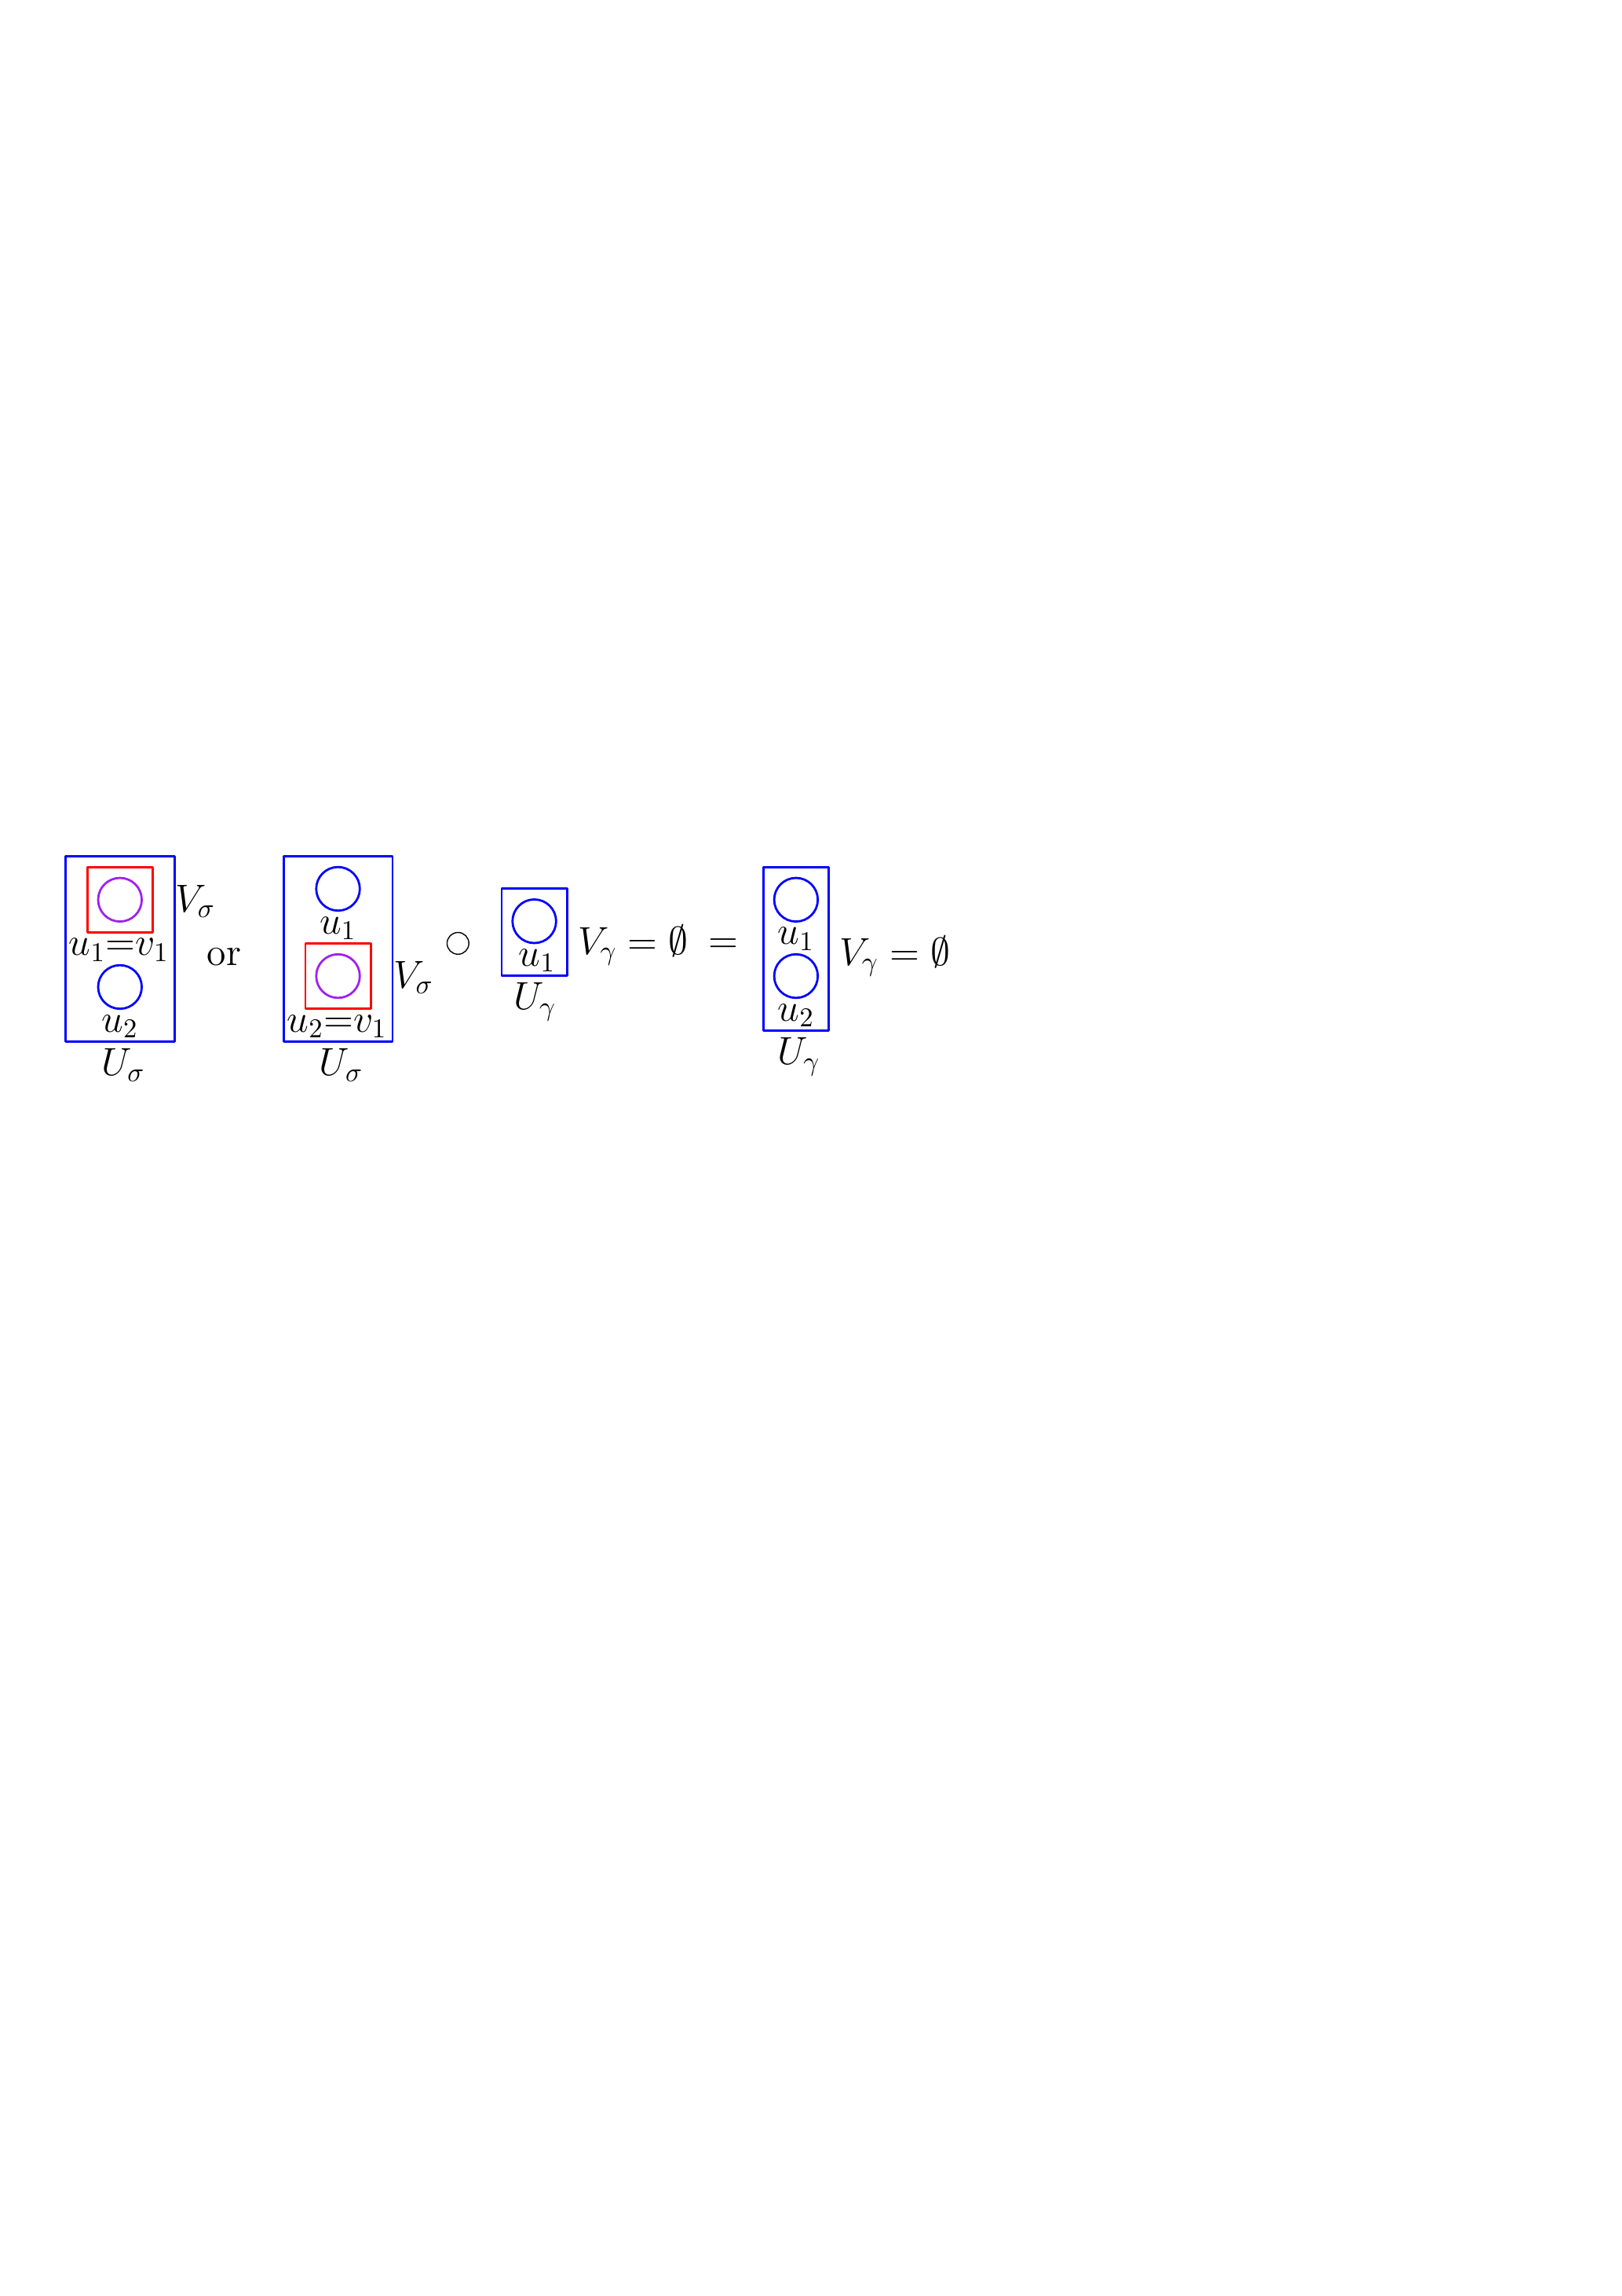}}
\caption{This figure shows the compositions $\sigma_{u_1,u_2 \to u_1} \circ \gamma_{u_1 \to \emptyset} = \sigma_{u_1,u_2 \to \emptyset}$ and $\sigma_{u_1,u_2 \to u_2} \circ \gamma_{u_1 \to \emptyset} = \sigma_{u_1,u_2 \to \emptyset}$.}
\end{figure}

Based on these compositions, we have the following matrices:
\begin{enumerate}
\item $H_{Id_{(u_1)}}^{-\gamma_7,\gamma_7}$ has two rows and columns indexed by $\sigma_{Id:}$ and $\sigma_{swap}$ and has entries $\left(\begin{matrix}
\frac{k^5}{n^5} & \frac{k^5}{n^5}\\
\frac{k^5}{n^5} & \frac{k^5}{n^5}\\
\end{matrix}\right)$.
\item $H_{Id_{(u_1)}}^{-\gamma_{u_1,u_2 \to u_1},\gamma_{u_1,u_2 \to u_1}}$ has two rows and columns indexed by $\sigma_{Id:}$ and $\sigma_{swap}$ and has entries $\left(\begin{matrix}
\frac{k^3}{n^3} & \frac{k^3}{n^3}\\
\frac{k^3}{n^3} & \frac{k^3}{n^3}\\
\end{matrix}\right)$.
\item $H_{Id_{(u_1)}}^{-\gamma_{u_1,u_2 \to u_2},\gamma_{u_1,u_2 \to u_2}} = H_{Id_{(u_1)}}^{-\gamma_{u_1,u_2 \to u_1},\gamma_{u_1,u_2 \to u_1}}$.
\item $H_{Id_{\emptyset}}^{-\gamma_{u_1,u_2 \to \emptyset},\gamma_{u_1,u_2 \to \emptyset}}$  has two rows and columns indexed by $\sigma_{Id:}$ and $\sigma_{swap}$ and has entries $\left(\begin{matrix}
\frac{k^4}{n^4} & \frac{k^4}{n^4}\\
\frac{k^4}{n^4} & \frac{k^4}{n^4}\\
\end{matrix}\right)$.
\item $H_{Id_{\emptyset}}^{-\gamma_{u_1 \to \emptyset},\gamma_{u_1 \to \emptyset}}$ has two rows and columns indexed by $\sigma_{u_1,u_2 \to u_1}$ and $\sigma_{u_1,u_2 \to u_2}$ and has entries $\left(\begin{matrix}
\frac{k^4}{n^4} & \frac{k^4}{n^4}\\
\frac{k^4}{n^4} & \frac{k^4}{n^4}\\
\end{matrix}\right)$.
\end{enumerate}
We can qualitatively verify the third condition of the machinery as follows
\begin{enumerate}
\item $B(\gamma_7)$ is $\tilde{O}(n^{\frac{|V(\gamma_7) \setminus U_{\gamma_7}|}{2}}) = \tilde{O}(\sqrt{n})$ so ${B(\gamma_7)^2}H_{Id_{(u_1)}}^{-\gamma_7,\gamma_7} \preceq H_{Id_{(u_1,u_2)}}$ as long as $k << n^{\frac{2}{3}}$.
\item $B(\gamma_{u_1,u_2 \to u_1})$ is $\tilde{O}(n^{\frac{|V(\gamma_{u_1,u_2 \to u_1}) \setminus U_{\gamma_{u_1,u_2 \to u_1}}|}{2}}) = \tilde{O}(1)$ so ${B(\gamma_{u_1,u_2 \to u_1})^2}H_{Id_{(u_1)}}^{-\gamma_{u_1,u_2 \to u_1},\gamma_{u_1,u_2 \to u_1}} \preceq H_{Id_{(u_1,u_2)}}$. Following the same logic, ${B(\gamma_{u_1,u_2 \to u_2})^2}H_{Id_{(u_1)}}^{-\gamma_{u_1,u_2 \to u_2},\gamma_{u_1,u_2 \to u_2}} \preceq H_{Id_{(u_1,u_2)}}$.
\item $B(\gamma_{u_1,u_2 \to \emptyset})$ is $\tilde{O}(n^{\frac{|V(\gamma_{u_1,u_2 \to \emptyset}) \setminus U_{\gamma_{u_1,u_2 \to \emptyset}}|}{2}}) = \tilde{O}(1)$ so ${B(\gamma_{u_1,u_2 \to \emptyset})^2}H_{Id_{\emptyset}}^{-\gamma_{u_1,u_2 \to \emptyset},\gamma_{u_1,u_2 \to \emptyset}} \preceq H_{Id_{(u_1,u_2)}}$.
\item $B(\gamma_{u_1 \to \emptyset})$ is $\tilde{O}(n^{\frac{|V(\gamma_{u_1 \to \emptyset}) \setminus U_{\gamma_{u_1 \to \emptyset}}|}{2}}) = \tilde{O}(1)$ so ${B(\gamma_{u_1 \to \emptyset})^2}H_{Id_{\emptyset}}^{-\gamma_{u_1 \to \emptyset},\gamma_{u_1 \to \emptyset}} \preceq H_{Id_{(u_1)}}$ as 
\[
\left(\begin{matrix}
\frac{k^3}{n^3} & \frac{k^3}{n^3} & \frac{k^4}{n^4}\\
\frac{k^3}{n^3} & \frac{k^3}{n^3} & \frac{k^4}{n^4}\\
\frac{k^4}{n^4} & \frac{k^4}{n^4} & C\frac{k^5}{n^5}\\
\end{matrix}\right) \succeq (1 - \frac{1}{C})\left(\begin{matrix}
\frac{k^3}{n^3} & \frac{k^3}{n^3} & 0\\
\frac{k^3}{n^3} & \frac{k^3}{n^3} & 0\\
0 & 0 & 0\\
\end{matrix}\right) \succeq \tilde{O}(1)\left(\begin{matrix}
\frac{k^4}{n^4} & \frac{k^4}{n^4} & 0\\
\frac{k^4}{n^4} & \frac{k^4}{n^4} & 0\\
0 & 0 & 0\\
\end{matrix}\right)
\].
\end{enumerate}	

%\end{appendix}
