# Supplementary material for: Nonlinear Random Matrices and Applications to the Sum of Squares Hierarchy
Source: arXiv:2302.04462 source file (2023-02-09)
Supplement: Supplementary file 2 [file CombinatorialPseudoCalibrationAppendix.tex]

\subsection{Combinatorial Proof of Lemma \ref{lem:fixed-moments}}\label{app:combinatorialpseudocalibration}
In this appendix, we give a combinatorial proof of Lemma \ref{lem:fixed-moments}. We recall the statement of Lemma \ref{lem:fixed-moments} here.
\begin{lemma}
Let $\alpha \in \N^n$. When $v$ is fixed and $b$ is fixed (not necessarily +1 or -1) and $d \sim N(0, I)$ conditioned on $\ip{v}{d} = b\norm{v}$, 
\[\E_{d}[h_{\alpha}(d)] = \frac{v^\alpha}{\norm{v}^{\abs{\alpha}}} \cdot h_{\abs{\alpha}}(b).\]
\end{lemma}
\begin{proof}
Again, it is sufficient to prove this lemma when $\norm{v} = 1$. For this proof, we need the following description of Hermite polynomials in terms of matchings and Isserlis' Theorem/Wick's Theorem.
\begin{fact}
\[
h_k(x) = \sum_{M: M \text{ is a matching on } [k]}{(-1)^{|M|}x^{k - 2|M|}}
\]
\end{fact}
\begin{theorem}[Isserlis' Theorem/Wick's Theorem]
For any vectors $u_1,\ldots,u_k$,
\[
E_{x \sim N(0,I)}\left[\prod_{j=1}^{k}{\ip{x}{u_j}}\right] = \sum_{M: M \text{ is a perfect matching on } [k]}\prod_{(i,j) \in M}{\ip{u_i}{u_j}}
\]
\end{theorem}
The idea behind this proof is to break up each coordinate vector $e_i$ into a component which is parallel to $v$ and a component which is perpendicular to $v$.
\begin{definition}
For each coordinate $i$, define $e_{i}^{\perp} = e_i - {v_i}v$
\end{definition}
\begin{proposition}
For any coordinate $i$, $\ip{e_{i}^{\perp}}{e_{i}^{\perp}} = 1-{v_i}^2$. For any pair of distinct coordintes $i$ and $i'$, $\ip{e_{i}^{\perp}}{e_{i'}^{\perp}} = -{v_i}{v_{i'}}$
\end{proposition}
\begin{proof}
Observe that for all i,
\[
\ip{e_{i}^{\perp}}{e_{i}^{\perp}} = \ip{e_{i} - {v_i}v}{e_{i} - v_{i}v} = \ip{e_{i}}{e_{i}}  - 2{v_i}\ip{v}{e_{i}} + {v_i}^2\ip{v}{v} = 1-{v_i}^2
\]
and if $i$ and $i'$ are distinct then
\[
\langle{e_{i}^{\perp},e_{i'}^{\perp}}\rangle = \langle{e_{i} - {v_i}v,e_{i'} - v_{i'}v}\rangle = \langle{e_{i},e_{i'}}\rangle  - {v_i}\langle{v,e_{i'}}\rangle - {v_{i'}}\langle{e_i,v}\rangle + {v_i}{v_{i'}}\langle{v,v}\rangle = -{v_i}{v_{i'}}
\]
\end{proof}
To evaluate $\E_{d}[h_{\alpha}(d)]$, we proceed as follows:
\begin{enumerate}
\item Break up each $d_i = \ip{d}{e_i}$ as $d_i = \ip{bv}{e_{i}} + \ip{d^{\perp}}{e_{i}} = bv_{i} + \ip{d^{\perp}}{e_{i}^{\perp}}$
where $d^{\perp}$ is the component of $d$ which is orthogonal to $v$.
\item Observe that since each $e^{\perp}_{i}$ is orthogonal to $v$, we can replace $d^{\perp}$ by a random vector $d' \sim N(0,I)$.
\item Apply Isserlis' Theorem/Wick's Theorem to evaluate these terms.
\end{enumerate}
For this calculation, it is convenient to think of $\alpha$ as a tuple of $|\alpha|$ elements where each $i \in [n]$ appears $\alpha_i$ times.
\begin{definition}
For each $j \in [\abs{\alpha}]$, we define $\alpha(j)$ to be the index $i$ such that $\sum_{i' = 1}^{i-1}{\alpha_{i'}} < j$ and $\sum_{i'=1}^{i}{\alpha_{i'}} \geq j$. For example, if $\alpha = (2,1,0,3)$ then $\alpha(1) = \alpha(2) = 1$, $\alpha(3) = 2$, and $\alpha(4) = \alpha(5) = \alpha(6) = 4$.
\end{definition}
In the special case when $\alpha(1),\ldots,\alpha(\abs{\alpha})$ are all distinct, 
\[
\E_{d}[h_{\alpha}(d)] = \E_d\Big[\prod_{j=1}^{\abs{\alpha}}{\ip{d}{e_{\alpha(j)}}}\Big] = \E_{d' \sim N(0,I)}\Big[\prod_{j=1}^{\abs{\alpha}}{\left(bv_{\alpha(j)} + \ip{d'}{e_{\alpha(j)}^{\perp}}\right)}\Big]
\]
In this case, we can associate a matching $M$ to each term we get after applying Isserlis' Theorem/Wick's Theorem as follows:
\begin{enumerate}
\item For each $j \in \abs{\alpha}$ where we have the $bv_{\alpha(j)}$ term, we take $j$ to be isolated.
\item For each pair of distinct $j,j' \in \abs{\alpha}$ such that we have the term $\ip{e_{\alpha
(j)}^{\perp}}{e_{\alpha(j')}^{\perp}}$ (which only happens if we start with the $\ip{d'}{e_{\alpha(j)}^{\perp}}$ and $\ip{d'}{e_{\alpha(j')}^{\perp}}$ terms and $e_{\alpha(j)}^{\perp}$ and $e_{\alpha(j')}^{\perp}$ are paired together after applying Isserlis' Theorem/Wick's Theorem), we add an edge between $j$ and $j'$ in $M$.
\end{enumerate}
We now have that
\begin{align*}
\E_{d}[h_{\alpha}(d)] &= \sum_{M:M \text{ is a matching on [\abs{\alpha}]}}{\left(\prod_{(j,j') \in M}{-v_{\alpha(j)}v_{\alpha(j')}}\right)\left(\prod_{j: j \text{ is unmatched by } M}{bv_{\alpha(j)}}\right)}\\ 
&= \left(\sum_{M:M \text{ is a matching on [\abs{\alpha}]}}{(-1)^{|M|}b^{\abs{\alpha} - 2|M|}}\right)\prod_{j=1}^{\abs{\alpha}}{v_{\alpha(j)}} \\
&= h_{\abs{\alpha}}(b)v^{\alpha} 
\end{align*}
For the general case, we use a similar idea although it is somewhat more complicated. In particular, we associate a multi-colored matching $M = M_{blue} \cup M_{red} \cup M_{purple}$ to each term. The idea is that whenever we have a blue edge, we could have had a red edge instead and vice versa, so we can combine terms with red and blue edges to make purple edges which gives us an ordinary matching as before. More precisely, the idea is as follows.
\begin{enumerate}
\item When we expand out $h_{\alpha}(d)$ in terms of matchings, we take $M_{blue}$ to be the union of these matchings.
\item For each $j \in \abs{\alpha}$ where we have the $bv_{\alpha(j)}$ term, we take $j$ to be isolated.
\item For each pair of distinct $j,j' \in \abs{\alpha}$ such that we have the term $\ip{e_{\alpha
(j)}^{\perp}}{e_{\alpha(j')}^{\perp}}$ (which only happens if we start with the $\ip{d'}{e_{\alpha(j)}^{\perp}}$ and $\ip{d'}{e_{\alpha(j')}^{\perp}}$ terms and $e_{\alpha(j)}^{\perp}$ and $e_{\alpha(j')}^{\perp}$ are paired together after applying Isserlis' Theorem/Wick's Theorem), we add an edge between $j$ and $j'$. If $\alpha(j') = \alpha(j)$ then we take this edge to be red and add it to $M_{red}$. If $\alpha(j') \neq \alpha(j)$ then we take this edge to be purple and add it to $M_{purple}$.
\end{enumerate}
We now implement this idea. We have that
\begin{align*}
&\E_{d}[h_{\alpha}(d)] = \sum_{M_{blue}: M_{blue} \text{ is a matching on } [\abs{\alpha}], \atop \forall (j,j') \in M_{blue}, \alpha(j) = \alpha(j')}{
(-1)^{|M_{blue}|}\E_{d}\Big[\prod_{j \in \abs{\alpha}: j \text{ is unmatched by } M_{blue}}{\ip{d}{e_{\alpha(j)}}}\Big]} \\
&=  \sum_{M_{blue}: M_{blue} \text{ is a matching on } [\abs{\alpha}], \atop \forall (j,j') \in M_{blue}, \alpha(j) = \alpha(j')}{
(-1)^{|M_{blue}|}\E_{d' \sim N(0,I)}\Big[\prod_{j \in \abs{\alpha}: j \text{ is unmatched by } M_{blue}}{\left(bv_{\alpha(j)} + \ip{d'}{e_{\alpha(j)}^{\perp}}\right)}\Big]}
\end{align*}
Expanding out $\E_{d' \sim N(0,I)}\Big[\prod_{j \in \abs{\alpha}: j \text{ is unmatched by } M_{blue}}{\left(bv_{\alpha(j)} + \ip{d'}{e_{\alpha(j)}^{\perp}}\right)}\Big]$ and applying Isserlis' Theorem/Wick's Theorem, we have that 
\begin{align*}
\E_{d}[h_{\alpha}(d)] &= \sum_{M_{blue},M_{red},M_{purple}}{(-1)^{|M_{blue}|}\prod_{(j,j') \in M_{red}}{(1-v^{2}_{\alpha(j)})}\prod_{(j,j') \in M_{purple}}{(-v_{\alpha(j)}v_{\alpha(j')})}} \\
&\prod_{j: j \text{ is unmatched by } M = M_{blue} \cup M_{red} \cup M_{purple}}{bv_{\alpha(j)}}
\end{align*}
where the sum is taken over all $M_{blue},M_{red},M_{purple}$ such that
\begin{enumerate}
\item $M = M_{blue} \cup M_{red} \cup M_{purple}$ is a matching on $[\abs{\alpha}]$ and $M_{blue},M_{red},M_{purple}$ are disjoint.
\item $\forall (j,j') \in M_{blue}, \alpha(j) = \alpha(j')$.
\item $\forall (j,j') \in M_{red}, \alpha(j) = \alpha(j')$.
\item $\forall (j,j') \in M_{purple}, \alpha(j) \neq \alpha(j')$.
\end{enumerate}
Since whenever we have a blue edge, we could have instead had a red edge and vice versa, for each distinct $j,j'$ such that $\alpha(j') = \alpha(j)$, we can combine terms which have a blue edge between $j$ and $j'$ with terms which have a red edge between $j$ and $j'$. A blue edge between $j$ and $j'$ has a coefficient of $-1$ and a red edge between $j$ and $j'$ has a coefficient of $1 - v^2_{\alpha(j)}$, so this effectively gives a purple edge with coefficient $-v^2_{\alpha(j)} = v_{\alpha(j)}v_{\alpha(j')}$. Thus, 
\begin{align*}
\E_{d}[h_{\alpha}(d)] &= \sum_{M:M \text{ is a matching on [\abs{\alpha}]}}{\left(\prod_{(j,j') \in M}{-v_{\alpha(j)}v_{\alpha(j')}}\right)\left(\prod_{j: j \text{ is unmatched by } M}{bv_{\alpha(j)}}\right)}\\ 
&= h_{\abs{\alpha}}(b)v^{\alpha} 
\end{align*}
\end{proof}
