# Supplementary material for: Nonlinear Random Matrices and Applications to the Sum of Squares Hierarchy
Source: arXiv:2302.04462 source file (2023-02-09)
Supplement: Supplementary file 3 [file ScalingAppendix.tex]

\subsection{Importance of Scaling}\label{app:scaling}
We remark that somewhat surprisingly, the scaling of the problem is important for our arguments. The reason this is somewhat surprising is that for the purpose of determining whether or not a matrix $M$ is PSD, the scaling of the rows and columns of $M$ doesn't matter. More precisely, we have the following proposition.
\begin{proposition}
For any symmetric $N \times N$ matrix $M$ and any $N \times N$ diagonal matrix $D$ such that $\forall i \in [N], D_{ii} \neq 0$, $M \succeq 0$ if and only if $DMD \succeq 0$.
\end{proposition}
However, for our techniques, we also use the fact that if $x$ is in the nullspace of $M$ then for the purposes of determining whether $M$ is PSD, we can freely add a non-negative multiple of $xx^T$ to $M$.
\begin{proposition}\label{addingnullspaceprop}
For any symmetric $N \times N$ symmetric matrix $M$, any vector $x$ such that $Mx = 0$, and any constant $c   $, $M \succeq 0$ if and only if $M+cxx^T \succeq 0$.
\end{proposition}
As shown by the following example, the set of matrices that can be obtained using Proposition \ref{addingnullspaceprop} depends on the scaling of $M$.

If $M = \begin{pmatrix}
1 & 1 & 2 \\
1 & 2 & 3 \\
2 & 3 & 5
\end{pmatrix}$, $x = \begin{pmatrix}
1\\
1\\
-1
\end{pmatrix}$, and $D = \begin{pmatrix}
1 & 0 & 0 \\
0 & 1 & 0 \\
0 & 0 & \lambda
\end{pmatrix}$
then $DMD = \begin{pmatrix}
1 & 1 & 2\lambda \\
1 & 2 & 3\lambda \\
2\lambda & 3\lambda & 5{\lambda}^2
\end{pmatrix}$ and 
\[
DMD + cD^{-1}x{x^T}D^{-1} = \begin{pmatrix}
1 + c & 1 + c & 2\lambda - \frac{c}{\lambda} \\
1 + c & 2 + c & 3\lambda - \frac{c}{\lambda} \\
2\lambda - \frac{c}{\lambda} & 3\lambda - \frac{c}{\lambda} & 5{\lambda}^2 + \frac{c}{{\lambda}^2}
\end{pmatrix}
\]
Scaling this so that the diagonal entries are $1$ gives the matrix 
\[
\begin{pmatrix}
1 & \frac{\sqrt{1+c}}{\sqrt{2+c}} & \frac{2\lambda - \frac{c}{\lambda}}{\sqrt{(1+c)(5{\lambda}^2 + \frac{c}{{\lambda}^2})}} \\
\frac{\sqrt{1+c}}{\sqrt{2+c}} & 1 & \frac{3\lambda - \frac{c}{\lambda}}{\sqrt{(2+c)(5{\lambda}^2 + \frac{c}{{\lambda}^2})}} \\
\frac{2\lambda - \frac{c}{\lambda}}{\sqrt{(1+c)(5{\lambda}^2 + \frac{c}{{\lambda}^2})}} & \frac{3\lambda - \frac{c}{\lambda}}{\sqrt{(2+c)(5{\lambda}^2 + \frac{c}{{\lambda}^2})}} & 1
\end{pmatrix}
\]
Note that the entries in the upper left $2 \times 2$ block only depend on $c$ and are different for each $c$ while the other off-diagonal entries also depend on $\lambda$. Thus, different $\lambda$ give different sets of matrices.
